# Supplementary material for: vMFCoOp: Towards Equilibrium on a Unified Hyperspherical Manifold for Prompting Biomedical VLMs
Source: arXiv:2511.09540 ancillary file (2025-11-20)
Supplement: Supplementary file 1 [file Appendix_document.pdf]

# vMFCoOp: Towards Equilibrium on a Unified Hyperspherical Manifold for Prompting Biomedical VLMs
# Appendix

## Detailed Dataset Description

Table A1 summarizes the 14 datasets utilized in our proposed *vMFCoOp* framework, spanning 12 distinct biomedical imaging modalities such as CT, brain MRI, cardiac MRI (CMRI), X-ray, ultrasound, and others, and covering 13 different anatomical organs. Each dataset is characterized by its imaging modality, target organ(s), number of semantic classes, and data split configuration (training/validation/test). These datasets encompass a wide range of challenging clinical scenarios, including kidney stones in CT, cardiac neoplastic conditions in CMRI, and brain tumors in brain MRI. Such diversity in disease categories and imaging types provides a rich and representative benchmark for evaluating biomedical image classification models. Rather than using the full training set of each dataset, we adopt randomly sampled few-shot subsets to simulate realistic low-data regimes and promote efficient and representative learning. To ensure balanced representation and fair evaluation, class-wise samples are proportionally distributed across the training, validation, and test splits. This strategy enhances the clinical relevance of model evaluation and contributes to the robustness of *vMFCoOp* across diverse biomedical classification tasks.

Specifically, for the UK Biobank datasets, we provide the corresponding ICD-10 diagnostic codes and their descriptions for each category. For cardiac MRI: *Congenital Heart Diseases* include Q22.6 (Hypoplastic right heart syndrome), Q23.4 (Hypoplastic left heart syndrome), Q24.4 (Other congenital malformations of heart), Q24.6 (Congenital heart block), Q24.8 (Other specified congenital malformations of heart), and Q24.9 (Unspecified congenital malformation of heart); *Ischemic Heart Diseases / Atherosclerosis* include I11 (Hypertensive heart disease), I25 (Chronic ischemic heart disease), and I25.1 (Atherosclerotic heart disease); *Valvular or Rheumatic Heart Diseases* include I05–I09 (Chronic rheumatic heart diseases); *Cardiomyopathies or Myocardial Injury* include S26 (Injury of heart) and I51.3 (Aneurysm of heart); *Infectious / Neoplastic Cardiac Diseases* include A39.5 (Meningococcal endocarditis) and C38 (Malignant neoplasm of heart, mediastinum, and pleura). For liver MRI: *Malignant Liver Tumors* correspond to C22 (Malignant neoplasm of liver and intrahepatic bile ducts); *Benign Liver Tumors* correspond to K75.0 (Liver cell adenoma); *Congenital Hepatobiliary Malformations* correspond to Q44 (Congenital malformations of gallbladder, bile ducts, and liver); *Liver Parasitic Infections* correspond to B67.5 (Echinococcus multilocularis infection of the liver); *Chronic Liver Diseases* correspond to K74 (Fibrosis and cirrhosis of liver); *Diffuse Hepatic Disorders* correspond to K76.0 (Fatty (change of) liver, not elsewhere classified). For pancreatic MRI: *Malignant Pancreatic Tumors* correspond to C25 (Malignant neoplasm of pancreas); *Overlapping or Unclassified Pancreatic Lesions* correspond to C25.8 (Overlapping lesion of pancreas); *Cystic Pancreatic Lesions* correspond to K86.2 (Cyst of pancreas); *Congenital Pancreatic Abnormalities* correspond to Q45.0 (Agenesis, aplasia and hypoplasia of pancreas).

Detailed patient demographics and clinical condition descriptions are provided in the `Participant_table.csv` files in the GitHub repository . All patient data have been de-identified to protect privacy.

**Important: Please note that all these patients' data are provided for reference only; any further sharing, citation or reproduction without prior authorisation would be inconsistent with the UK Biobank Access Terms and is not permitted.**

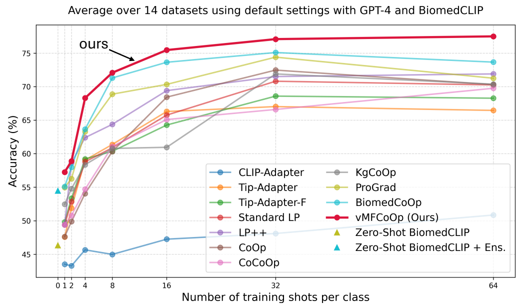


Figure A1: Average classification accuracy (%) of few-shot adaptation methods across 14 datasets with varying shots per class, using `GPT-4` and `BiomedCLIP`.


This paper has been selected for **Oral Presentation** at AAAI-2026 Main Technical Track, organized by the Association for the Advancement of Artificial Intelligence (www.aaai.org).

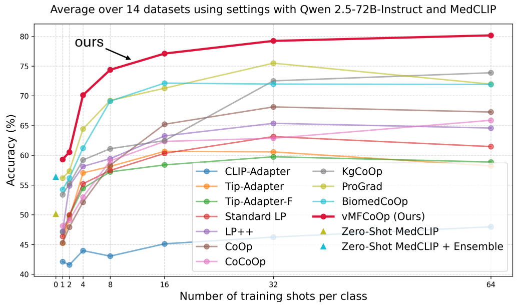


Figure A2: Average classification accuracy (%) of few-shot adaptation methods across 14 datasets with varying shots per class, using `Qwen 2.5-72B-Instruct` and `MedCLIP`.

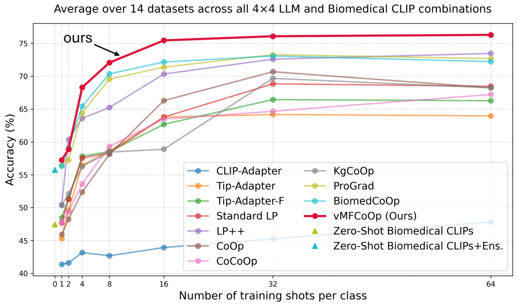


Figure A3: Average classification accuracy (%) of few-shot adaptation methods across 14 datasets with varying shots per class across all LLMs and Biomedical CLIPs pair.

## Full Details of Few-shot Results

Figure A1 illustrates the performance of vMFCoOp and baseline models across varying few-shot settings ($K$ = 1, 2, 4, 8, 16, 32, 64), highlighting the robustness of vMFCoOp under limited data conditions. In addition, Table A2 reports detailed per-dataset few-shot results, corresponding to Table 1 in the main text (GPT-4 + BiomedCLIP). Noted that to ensure a fair and informative comparison, we include *Biomedical CLIP (e.g., BiomedCLIP) + Ensemble* and *Biomedical CLIP + Selective Ensemble* baselines, which are implemented by following the BiomedCoOp framework. Specifically, *Biomedical CLIP + Ensemble* averages the $N$ LLM-generated prompt embeddings per class, while *+ Selective Ensemble* further excludes outlier prompts via a Median Absolute Deviation (MAD)-based filtering strategy prior to averaging.

Figure A2 presents the best-performing LLM–Biomedical CLIP pair for vMFCoOp under the Qwen2.5-72B-Instruct and MedCLIP setting. Notably, several competing methods exhibit noticeable performance drops or fluctuations when the pairing changes, indicating limited robustness. Detailed per-dataset results can be found in table A3.

To further assess the generalizability and flexibility of our method in adapting to various foundation model combinations for prompt learning, we summarize the performance across all 16 LLM–BiomedCLIP pairs. These include Qwen2.5-72B-Instruct, Claude 3.5–1022, DeepSeek-VL R1, and GPT-4 as LLMs, and BiomedCLIP, PubMedCLIP, MedCLIP, and PMC-CLIP as biomedical vision encoders, as described in the main paper. The overall performance comparison is visualized in fig. A3, with detailed dataset-wise averages provided in table A4. All experiments in this section are conducted using 50 prompts generated from the LLM. Overall, vMFCoOp achieves performance comparable to state-of-the-art methods and consistently outperforms them across 14 biomedical imaging datasets.

In addition, we provide the main code file of vMFCoOp; please refer to `main.py` in the `Supplementary Materials.zip`. The experiments and code were tested on a computing system equipped with an Intel Xeon Platinum 8370C CPU, NVIDIA A100 80GB GPU, 128GB RAM, running Ubuntu 22.04, using Python 3.8 and PyTorch 2.1.0 with CUDA 11.8. We report few-shot classification accuracy as the evaluation metric, which reflects the model's ability to generalize from limited examples, a key challenge in few-shot learning.

## Effect of the context vector length

As shown in table A7, increasing the context length consistently degrades performance on both base and novel classes, with a more pronounced decline on novel classes. A shorter context length (e.g., 4) offers a better trade-off, yielding a higher harmonic mean (HM). These results suggest that longer contexts may hinder the model's generalization across base and novel classes.

## Base-to-Novel Settings and Scaling Study

Table A8 presents the selected hyperparameters $\lambda_{\text{anc}}$ and $\lambda_{\text{sc}}$ for each medical imaging dataset under both Few-shot and Base-to-Novel evaluation protocols. Additionally, we evaluated the default GPT-4 + BioMedCLIP setup under 32-shot and 64-shot conditions; the comparative results are reported in table A7.

## Additional Visual Interpretations

To provide a more rigorous complement to the analysis of Visual Interpretability, we present additional details on other datasets and further include comparisons with the recent XCoOp (Bie et al. 2024) method. Specifically, we report results on the UK Biobank pancreas MRI, brain MRI across different planes (axial and sagittal), as well as dermoscopy and endoscopy datasets, as illustrated in fig. A4.

## Analysis of Number of LLM Prompts

As mentioned in the *Implementation Details*, we conducted additional experiments to analyze the *Effect of the Number of LLM Prompts*. All configurations follow our default setting with GPT-4 and BiomedCLIP, and each setup is repeated three times for robustness. We compare our method, *vMFCoOp*, with the recent state-of-the-art approach *BiomedCoOp*. As shown in table A9 and table A10, although their method achieves improvement under low-shot settings, it exhibits noticeably higher variance

when the number of prompts increases. In contrast, our approach maintains consistent performance even under varying prompt configurations and larger values of $K$, demonstrating better stability and generalization.

## Prompt Template Comparison Across LLMs

We present 15 representative prompts per LLM, showcasing examples generated by Qwen2.5 and GPT-4 across all classes and datasets. Table A11 and table A12 further illustrate the nearest words for each of the four context vectors learned by vMFCoOp from these prompts (with BiomedCLIP). *These results clearly reveal the semantic preference differences between foundation model families, further highlighting the significance of our study objective.*

**GPT-4:**

- `A brain MRI showing normal gray-white matter differentiation, intact sulci, and no abnormal masses or signal changes.`
- `MRI of the brain with glioma reveals a heterogeneous lesion with irregular borders and areas of central necrosis.`
- `Meningioma on MRI appears as a sharply circumscribed, dural-based mass with homogeneous enhancement and a dural tail.`
- `Breast ultrasound demonstrates a well-defined, hypoechoic nodule with smooth margins, characteristic of a benign lesion.`
- `Breast ultrasound reveals an irregular, hypoechoic mass with microcalcifications, suggestive of malignancy.`
- `Chest X-ray displays clear lung fields and sharp costophrenic angles, indicating normal pulmonary anatomy.`
- `Chest X-ray with multifocal ground-glass opacities and consolidations, typical findings in viral pneumonia.`
- `Renal CT shows a well-marginated, non-enhancing, low-density lesion consistent with a simple kidney cyst.`
- `Kidney CT scan reveals a hyperdense calculus with posterior acoustic shadowing, typical of a renal stone.`
- `Skin lesion photograph displays an asymmetric, darkly pigmented patch with irregular borders, concerning for melanoma.`
- `Endoscopic image reveals a lobulated, pedunculated polyp with a smooth surface in the colon.`
- `A normal heart MRI shows symmetrical chambers, normal wall motion, and no late gadolinium enhancement.`
- `Liver MRI demonstrates a homogenous parenchyma, sharp organ borders, and no evidence of focal lesions.`
- `Pancreatic MRI reveals a normal gland size, uniform signal intensity, and no cystic or solid masses.`
- `Ulcerative colitis on colonoscopy displays continuous mucosal erythema, edema, and loss of vascular pattern.`

**Qwen-2.5:**

- `T1-weighted MRI reveals exquisitely delineated gray-white matter differentiation without mass effect or aberrant signal intensity, characteristic of neurotypical parenchymal architecture.`
- `Glioblastoma multiforme demonstrates heterogeneous enhancement with central necrotic core and surrounding FLAIR hyperintensity, indicative of vasogenic edema infiltrating white matter tracts.`
- `Contrast-enhanced MRI exhibits a dural-based mass with homogeneous enhancement and meningeal tail sign, pathognomonic for parasagittal meningioma.`
- `Cardiac cine MRI reveals asymmetric septal hypertrophy with late gadolinium enhancement in the anteroseptal myocardium, consistent with hypertrophic cardiomyopathy phenotype.`
- `Dynamic contrast-enhanced liver MRI shows arterial phase hyperenhancement with subsequent washout in hepatobiliary phase, characteristic of dysplastic nodule in cirrhotic parenchyma.`
- `Pancreatic protocol CT demonstrates a hypodense lesion with ductal dilation and double-duct sign, highly suggestive of pancreatic adenocarcinoma.`
- `Ultrasound reveals an ovoid hypoechoic mass with parallel orientation and posterior acoustic enhancement, conforming to BI-RADS 3 benign fibroadenoma criteria.`
- `High-resolution CT exhibits diffuse ground-glass opacities with peripheral traction bronchiectasis, indicative of fibrotic phase COVID-19 pneumonitis.`

- Non-contrast CT scan depicts a staghorn calculus occupying the renal pelvis with associated hydronephrosis, diagnostic of struvite nephrolithiasis.
- Dermoscopic visualization reveals polymorphous vessels with blue-whitish veil and irregular pigment network, highly concerning for nodular melanoma subtype.
- Endoscopic image demonstrates circumferential mucosal erosion with friability and spontaneous bleeding, hallmark findings of severe ulcerative colitis exacerbation.
- Arterial spin labeling MRI shows perfusion asymmetry in the mesiotemporal structures, correlating with mesial temporal sclerosis epileptogenic focus.
- Diffusion-weighted imaging reveals restricted diffusion in the splenium corporis callosi, indicative of cytotoxic edema in PRES encephalopathy.
- Contrast-enhanced mammography displays clustered pleomorphic calcifications with associated architectural distortion, suspicious for ductal carcinoma in situ.
- MR cholangiopancreatography visualizes cystic dilation of side-branch ducts with communicating pancreatic cysts, diagnostic of IPMN precursor lesion.

## References

Bie, Y.; Luo, L.; Chen, Z.; and Chen, H. 2024. Xcoop: Explainable prompt learning for computer-aided diagnosis via concept-guided context optimization. In *International Conference on Medical Image Computing and Computer-Assisted Intervention*, 773–783. Springer.

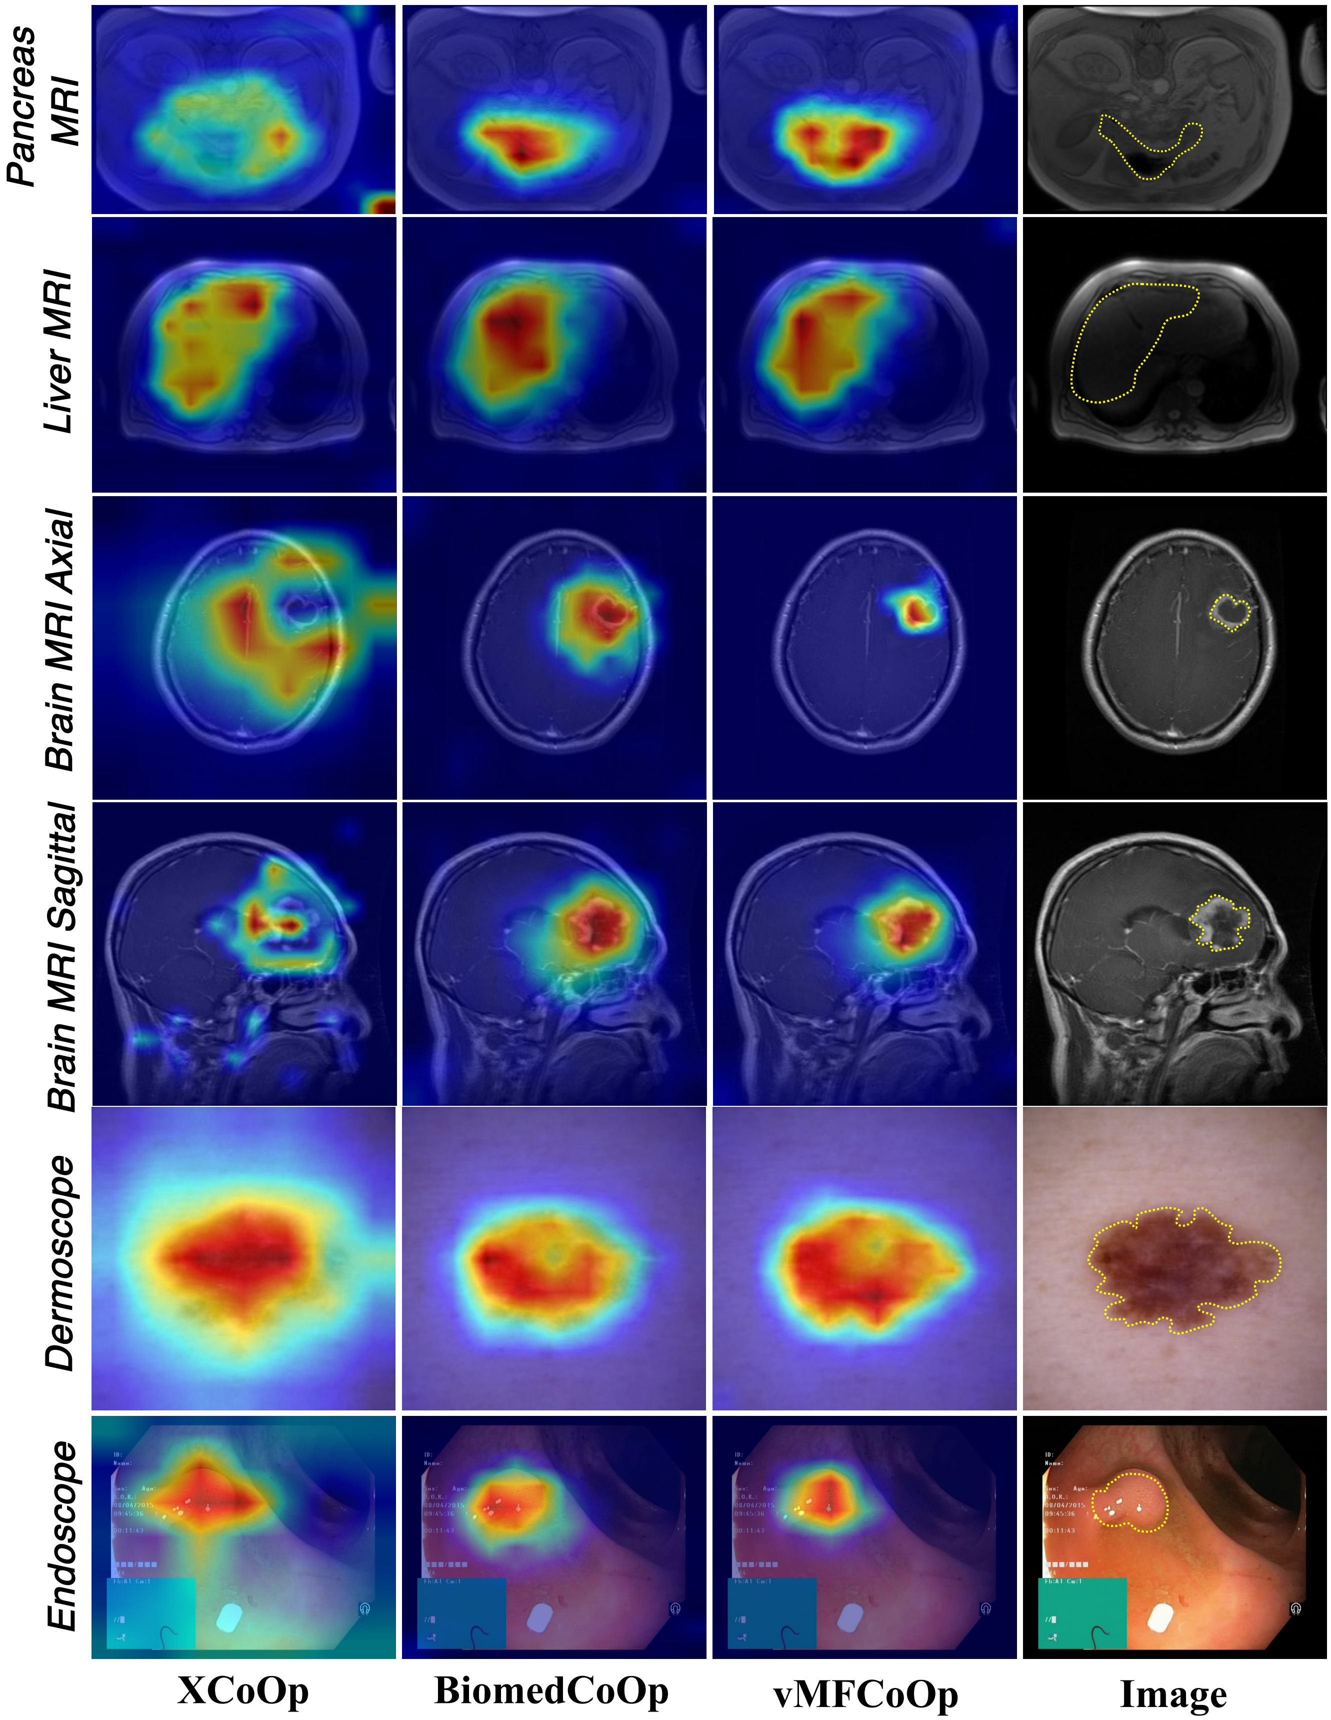


Figure A4: Additional qualitative results illustrating visual interpretability on UKB pancreas MRI, brain MRI (axial and sagittal planes), dermoscopy, and endoscopy, comparing our method with XCoOp and BiomedCoOp.

| Modality | Organ(s) | Name | Classes | # train/val/test |
|---|---|---|---|---|
| Computerized Tomography | Kidney | CTKidney | Kidney Cyst, Kidney Stone, Kidney Tumor, Normal Kidney | 6221/2487/3738 |
| Dermatoscopy | Skin | DermaMNIST | Actinic Keratosis, Basal Cell Carcinoma, Benign Keratosis, Dermatofibroma, Melanocytic nevus, Melanoma, Vascular Lesion | 7007/1003/2005 |
| Endoscopy | Colon | Kvasir | Dyed Lifted Polyps, Normal Cecum, Esophagitis, Dyed Resection Margins, Normal Pylorus, Normal Z Line, Polyps, Ulcerative Colitis | 2000/800/1200 |
| Fundus Photography | Retina | RETINA | Cataract, Diabetic Retinopathy, Glaucoma, Normal Retina | 2108/841/1268 |
| Histopathology | Lung Colon | LC25000 | Colon Adenocarcinoma, Colon Benign Tissue, Lung Adenocarcinoma, Lung Benign Tissue, Lung Squamous Cell Carcinoma | 12500/5000/7500 |
| | Colorectal | CHMNIST | Adipose Tissue, Complex Stroma, Debris, Empty Background, Immune Cells, Normal Mucosal Glands, Simple Stroma, Tumor Epithelium | 2496/1000/1504 |
| Brain MRI | Brain | BTMRI | Glioma Tumor, Meningioma Tumor, Normal Brain, Pituitary Tumor | 2854/1141/1717 |
| Cine MRI | Heart | UKB-CardiacMRI | Congenital Heart Diseases, Ischemic Heart Diseases / Atherosclerosis, Valvular or Rheumatic Heart Diseases, Cardiomyopathies or Myocardial Injury, Infectious / Neoplastic Cardiac Diseases | 17296/3706/3707 |
| Liver MRI | Liver | UKB-LiverMRI | Malignant Liver Tumors, Benign Liver Tumors, Congenital Hepatobiliary Malformations, Liver Parasitic Infections, Chronic Liver Diseases (Fibrosis and Cirrhosis), Diffuse Hepatic Disorders (e.g., Fatty Liver) | 3457/741/740 |
| Pancreas MRI | Pancreas | UKB-PancreasMRI | Malignant Pancreatic Tumors, Overlapping or Unclassified Pancreatic Lesions, Cystic Pancreatic Lesions, Congenital Pancreatic Abnormalities | 2049/439/439 |
| Optical Coherence Tomography | Retina | OCTMNIST | Choroidal Neovascularization, Drusen, Diabetic Macular Edema, Normal | 97477/10832/1000 |
| Ultrasound | Breast | BUSI | Benign Tumors, Malignant Tumors, Normal Scans | 389/155/236 |
| X-Ray | Chest | COVID-QU-Ex | COVID-19, Lung Opacity, Normal Lungs, Viral Pneumonia | 10582/4232/6351 |
| | Knee | KneeXray | No, Doubtful, Minimal, Moderate, and Severe Osteoarthritis | 5778/826/1656 |

Table A1: An overview of the 14 datasets used spanning 12 biomedical imaging modalities and 13 different organs.

| Dataset | Method | $K=1$ | $K=2$ | $K=4$ | $K=8$ | $K=16$ | $K=32$ | $K=64$ |
|---|---|---|---|---|---|---|---|---|
| | BiomedCLIP | | | | 60.07 | | | |
| | BiomedCLIP + Ensemble | | | | 63.87 | | | |
| | CLIP-Adapter | $55.08_{\pm3.79}$ | $56.18_{\pm3.67}$ | $57.96_{\pm3.45}$ | $56.79_{\pm3.82}$ | $61.05_{\pm3.54}$ | $61.31_{\pm3.67}$ | $63.94_{\pm3.76}$ |
| | Tip-Adapter | $64.04_{\pm3.29}$ | $66.83_{\pm2.73}$ | $77.35_{\pm1.48}$ | $72.44_{\pm3.12}$ | $77.05_{\pm1.31}$ | $78.82_{\pm1.02}$ | $78.56_{\pm1.19}$ |
| | Tip-Adapter-F | $57.45_{\pm2.27}$ | $61.83_{\pm5.63}$ | $74.57_{\pm1.54}$ | $72.81_{\pm1.76}$ | $74.01_{\pm2.04}$ | $77.93_{\pm2.18}$ | $77.80_{\pm2.49}$ |
| | Standard LP | $62.92_{\pm4.23}$ | $70.77_{\pm5.13}$ | $72.51_{\pm2.29}$ | $71.22_{\pm3.07}$ | $76.38_{\pm2.45}$ | $82.11_{\pm2.68}$ | $81.64_{\pm2.91}$ |
| BTMRI | LP++ | $67.12_{\pm5.39}$ | $76.60_{\pm5.31}$ | $77.68_{\pm1.22}$ | $76.20_{\pm1.27}$ | $81.86_{\pm1.33}$ | $83.91_{\pm1.44}$ | $84.67_{\pm1.75}$ |
| | CoOp | $61.80_{\pm3.47}$ | $63.92_{\pm4.85}$ | $68.25_{\pm2.44}$ | $73.65_{\pm1.92}$ | $80.15_{\pm1.74}$ | $84.81_{\pm1.72}$ | $82.47_{\pm1.83}$ |
| | CoCoOp | $60.96_{\pm3.74}$ | $63.56_{\pm3.58}$ | $66.43_{\pm4.31}$ | $70.08_{\pm4.22}$ | $76.54_{\pm1.49}$ | $78.20_{\pm1.64}$ | $81.62_{\pm1.87}$ |
| | KgCoOp | $63.85_{\pm3.61}$ | $71.36_{\pm5.14}$ | $75.58_{\pm2.37}$ | $75.80_{\pm1.03}$ | $76.74_{\pm3.28}$ | $87.49_{\pm3.47}$ | $86.13_{\pm3.52}$ |
| | ProGrad | $71.30_{\pm1.98}$ | $72.82_{\pm2.89}$ | $78.37_{\pm4.93}$ | $81.66_{\pm1.58}$ | $84.86_{\pm1.04}$ | $89.57_{\pm1.18}$ | $86.48_{\pm1.47}$ |
| | BiomedCoOp | $63.91_{\pm1.66}$ | $69.94_{\pm3.84}$ | $76.35_{\pm3.63}$ | $80.47_{\pm2.08}$ | $83.37_{\pm1.23}$ | $85.02_{\pm1.29}$ | $83.55_{\pm1.38}$ |
| | vMFCoOp | $64.67_{\pm1.72}$ | $69.29_{\pm3.97}$ | $80.22_{\pm3.72}$ | $80.96_{\pm2.07}$ | $84.98_{\pm1.18}$ | $86.82_{\pm1.34}$ | $87.49_{\pm1.45}$ |
| | BiomedCLIP | | | | 64.03 | | | |
| | BiomedCLIP + Ensemble | | | | 62.82 | | | |
| | CLIP-Adapter | $60.81_{\pm3.82}$ | $60.62_{\pm3.85}$ | $63.56_{\pm3.79}$ | $62.00_{\pm1.35}$ | $64.52_{\pm2.05}$ | $65.30_{\pm1.98}$ | $68.40_{\pm2.1}$ |
| | Tip-Adapter | $60.83_{\pm2.3}$ | $62.01_{\pm2.5}$ | $61.49_{\pm1.2}$ | $55.82_{\pm10.2}$ | $68.32_{\pm5.3}$ | $70.04_{\pm5.05}$ | $69.56_{\pm5.18}$ |
| | Tip-Adapter-F | $60.57_{\pm2.11}$ | $57.53_{\pm6.82}$ | $63.50_{\pm6.53}$ | $63.69_{\pm2.24}$ | $64.95_{\pm1.32}$ | $70.80_{\pm1.2}$ | $70.63_{\pm1.3}$ |
| | Standard LP | $52.51_{\pm10.55}$ | $46.91_{\pm6.07}$ | $51.12_{\pm7.12}$ | $60.31_{\pm6.2}$ | $64.45_{\pm1.75}$ | $70.90_{\pm1.88}$ | $70.21_{\pm1.97}$ |
| BUSI | LP++ | $53.82_{\pm5.13}$ | $61.40_{\pm2.28}$ | $63.65_{\pm3.05}$ | $66.29_{\pm2.24}$ | $70.89_{\pm1.62}$ | $74.14_{\pm1.7}$ | $74.90_{\pm1.85}$ |
| | CoOp | $47.51_{\pm3.05}$ | $49.73_{\pm2.78}$ | $55.02_{\pm3.48}$ | $59.57_{\pm5.95}$ | $68.07_{\pm3.12}$ | $73.22_{\pm3.4}$ | $70.84_{\pm3.5}$ |
| | CoCoOp | $54.62_{\pm3.53}$ | $49.76_{\pm2.59}$ | $59.71_{\pm1.78}$ | $65.75_{\pm3.48}$ | $70.07_{\pm1.1}$ | $71.87_{\pm1.25}$ | $75.06_{\pm1.3}$ |
| | KgCoOp | $55.08_{\pm7.12}$ | $57.71_{\pm2.97}$ | $63.10_{\pm4.28}$ | $64.92_{\pm2.22}$ | $66.94_{\pm1.98}$ | $78.15_{\pm2.35}$ | $76.46_{\pm2.4}$ |
| | ProGrad | $51.14_{\pm4.05}$ | $51.76_{\pm7.05}$ | $65.60_{\pm7.18}$ | $68.07_{\pm4.05}$ | $74.08_{\pm2.6}$ | $78.88_{\pm2.6}$ | $76.00_{\pm2.9}$ |
| | BiomedCoOp | $50.03_{\pm1.62}$ | $50.71_{\pm6.98}$ | $59.41_{\pm1.15}$ | $66.59_{\pm4.55}$ | $71.44_{\pm2.28}$ | $73.84_{\pm2.25}$ | $72.56_{\pm2.35}$ |
| | vMFCoOp | $52.11_{\pm1.73}$ | $51.13_{\pm7.01}$ | $63.36_{\pm1.07}$ | $66.64_{\pm4.53}$ | $73.99_{\pm2.12}$ | $75.59_{\pm2.29}$ | $76.24_{\pm2.34}$ |
| | BiomedCLIP | | | | 46.78 | | | |
| | BiomedCLIP + Ensemble | | | | 70.52 | | | |
| | CLIP-Adapter | $48.69_{\pm1.47}$ | $41.93_{\pm1.03}$ | $47.16_{\pm3.17}$ | $47.69_{\pm1.13}$ | $49.95_{\pm1.27}$ | $51.69_{\pm1.15}$ | $54.56_{\pm1.31}$ |
| | Tip-Adapter | $59.55_{\pm7.59}$ | $58.34_{\pm5.04}$ | $65.29_{\pm9.98}$ | $65.77_{\pm5.27}$ | $73.00_{\pm1.17}$ | $73.04_{\pm1.42}$ | $72.67_{\pm1.79}$ |
| | Tip-Adapter-F | $52.80_{\pm16.87}$ | $54.28_{\pm7.53}$ | $67.42_{\pm4.01}$ | $63.97_{\pm3.98}$ | $70.18_{\pm3.11}$ | $73.42_{\pm3.19}$ | $73.45_{\pm3.46}$ |
| | Standard LP | $50.31_{\pm10.55}$ | $46.37_{\pm15.93}$ | $56.67_{\pm12.67}$ | $62.34_{\pm5.84}$ | $68.21_{\pm1.89}$ | $73.06_{\pm2.17}$ | $72.54_{\pm2.34}$ |
| COVID-QU-Ex | LP++ | $48.26_{\pm10.42}$ | $61.23_{\pm14.47}$ | $64.44_{\pm9.08}$ | $65.16_{\pm8.23}$ | $72.72_{\pm1.11}$ | $75.02_{\pm1.36}$ | $75.57_{\pm1.57}$ |
| | CoOp | $56.79_{\pm13.95}$ | $53.83_{\pm7.76}$ | $60.91_{\pm6.29}$ | $69.14_{\pm3.33}$ | $75.29_{\pm1.47}$ | $79.35_{\pm1.84}$ | $77.09_{\pm2.12}$ |
| | CoCoOp | $70.85_{\pm2.53}$ | $68.37_{\pm2.47}$ | $62.39_{\pm9.67}$ | $68.47_{\pm3.05}$ | $73.54_{\pm3.68}$ | $74.87_{\pm3.95}$ | $77.86_{\pm1.13}$ |
| | KgCoOp | $62.45_{\pm9.24}$ | $55.83_{\pm11.75}$ | $65.57_{\pm8.37}$ | $72.55_{\pm3.35}$ | $72.15_{\pm3.93}$ | $82.83_{\pm1.12}$ | $81.22_{\pm1.27}$ |
| | ProGrad | $64.52_{\pm11.27}$ | $66.01_{\pm5.98}$ | $70.70_{\pm3.05}$ | $77.77_{\pm1.18}$ | $77.51_{\pm1.21}$ | $81.73_{\pm1.41}$ | $78.52_{\pm1.63}$ |
| | BiomedCoOp | $70.94_{\pm2.28}$ | $70.42_{\pm1.28}$ | $72.54_{\pm2.07}$ | $79.74_{\pm3.48}$ | $79.97_{\pm3.31}$ | $81.24_{\pm3.62}$ | $79.66_{\pm3.79}$ |
| | vMFCoOp | $71.94_{\pm2.36}$ | $70.01_{\pm1.54}$ | $76.06_{\pm2.22}$ | $79.37_{\pm3.52}$ | $81.06_{\pm3.34}$ | $82.76_{\pm3.67}$ | $83.18_{\pm0.82}$ |
| | BiomedCLIP | | | | 46.03 | | | |
| | BiomedCLIP + Ensemble | | | | 59.98 | | | |
| | CLIP-Adapter | $44.38_{\pm3.71}$ | $38.17_{\pm1.79}$ | $42.18_{\pm1.98}$ | $42.83_{\pm3.68}$ | $46.53_{\pm1.22}$ | $47.42_{\pm1.61}$ | $50.05_{\pm1.81}$ |
| | Tip-Adapter | $40.84_{\pm4.47}$ | $49.06_{\pm7.18}$ | $54.99_{\pm3.84}$ | $66.72_{\pm8.22}$ | $73.70_{\pm7.65}$ | $72.01_{\pm7.12}$ | $70.47_{\pm6.94}$ |
| | Tip-Adapter-F | $45.44_{\pm6.54}$ | $57.74_{\pm7.92}$ | $57.74_{\pm9.67}$ | $70.60_{\pm6.42}$ | $74.14_{\pm3.11}$ | $80.67_{\pm3.28}$ | $77.80_{\pm3.46}$ |
| | Standard LP | $42.69_{\pm5.23}$ | $56.71_{\pm5.98}$ | $65.57_{\pm6.84}$ | $71.05_{\pm7.12}$ | $78.48_{\pm5.31}$ | $81.29_{\pm5.02}$ | $81.12_{\pm5.17}$ |
| CTKIDNEY | LP++ | $57.31_{\pm2.78}$ | $67.34_{\pm3.42}$ | $66.78_{\pm8.04}$ | $74.70_{\pm7.67}$ | $79.83_{\pm7.05}$ | $78.82_{\pm6.74}$ | $78.67_{\pm6.56}$ |
| | CoOp | $50.41_{\pm8.15}$ | $56.73_{\pm2.36}$ | $60.15_{\pm2.47}$ | $69.59_{\pm3.72}$ | $80.20_{\pm1.93}$ | $82.71_{\pm1.65}$ | $81.95_{\pm1.52}$ |
| | CoCoOp | $47.91_{\pm6.88}$ | $50.92_{\pm9.27}$ | $59.55_{\pm1.22}$ | $72.13_{\pm1.45}$ | $76.04_{\pm2.58}$ | $76.72_{\pm2.42}$ | $80.67_{\pm2.57}$ |
| | KgCoOp | $59.91_{\pm1.22}$ | $62.67_{\pm3.05}$ | $67.60_{\pm5.46}$ | $75.32_{\pm4.15}$ | $71.77_{\pm2.58}$ | $82.61_{\pm2.82}$ | $81.29_{\pm2.67}$ |
| | ProGrad | $56.18_{\pm8.13}$ | $64.14_{\pm4.89}$ | $69.28_{\pm1.85}$ | $81.74_{\pm4.05}$ | $84.58_{\pm2.43}$ | $85.09_{\pm2.98}$ | $81.77_{\pm2.65}$ |
| | BiomedCoOp | $54.09_{\pm4.28}$ | $62.51_{\pm5.13}$ | $66.03_{\pm1.91}$ | $80.01_{\pm3.98}$ | $83.30_{\pm2.33}$ | $83.78_{\pm2.37}$ | $82.24_{\pm2.47}$ |
| | vMFCoOp | $58.02_{\pm4.47}$ | $64.76_{\pm5.44}$ | $71.35_{\pm2.13}$ | $81.40_{\pm4.35}$ | $86.78_{\pm2.55}$ | $89.76_{\pm2.68}$ | $89.46_{\pm0.72}$ |
| | BiomedCLIP | | | | 42.24 | | | |
| | BiomedCLIP + Ensemble | | | | 57.43 | | | |
| | CLIP-Adapter | $34.49_{\pm6.14}$ | $35.16_{\pm6.05}$ | $36.00_{\pm3.58}$ | $33.92_{\pm6.01}$ | $29.83_{\pm3.12}$ | $30.40_{\pm3.45}$ | $32.57_{\pm3.89}$ |
| | Tip-Adapter | $37.54_{\pm2.3}$ | $40.19_{\pm12.48}$ | $48.37_{\pm6.02}$ | $60.76_{\pm5.28}$ | $63.37_{\pm1.2}$ | $63.35_{\pm1.45}$ | $63.00_{\pm1.37}$ |
| | Tip-Adapter-F | $37.99_{\pm15.12}$ | $38.86_{\pm3.99}$ | $48.55_{\pm4.69}$ | $37.62_{\pm2.02}$ | $48.71_{\pm4.45}$ | $52.40_{\pm4.18}$ | $51.66_{\pm4.1}$ |
| | Standard LP | $31.03_{\pm12.8}$ | $36.78_{\pm9.95}$ | $46.69_{\pm8.05}$ | $47.30_{\pm3.12}$ | $50.27_{\pm3.17}$ | $55.87_{\pm3.4}$ | $54.12_{\pm3.24}$ |
| DermaMNIST | LP++ | $28.80_{\pm3.54}$ | $33.47_{\pm11.1}$ | $37.67_{\pm8.67}$ | $44.50_{\pm2.55}$ | $52.00_{\pm1.97}$ | $53.54_{\pm2.05}$ | $53.60_{\pm2.14}$ |
| | CoOp | $24.12_{\pm8.75}$ | $34.29_{\pm5.65}$ | $39.89_{\pm6.05}$ | $40.14_{\pm6.01}$ | $49.16_{\pm2.3}$ | $53.24_{\pm2.45}$ | $50.05_{\pm2.61}$ |
| | CoCoOp | $26.14_{\pm4.11}$ | $24.57_{\pm3.55}$ | $24.39_{\pm5.21}$ | $39.76_{\pm2.0}$ | $40.99_{\pm6.1}$ | $41.82_{\pm5.95}$ | $44.61_{\pm5.72}$ |
| | KgCoOp | $28.02_{\pm10.32}$ | $32.08_{\pm4.11}$ | $35.42_{\pm7.65}$ | $35.63_{\pm4.5}$ | $34.45_{\pm2.04}$ | $44.35_{\pm2.18}$ | $42.36_{\pm2.25}$ |
| | ProGrad | $37.93_{\pm10.2}$ | $39.46_{\pm6.12}$ | $46.40_{\pm10.21}$ | $53.55_{\pm2.09}$ | $48.58_{\pm4.8}$ | $53.68_{\pm4.9}$ | $50.20_{\pm5.0}$ |
| | BiomedCoOp | $57.27_{\pm4.21}$ | $56.30_{\pm1.15}$ | $61.69_{\pm1.95}$ | $64.49_{\pm3.67}$ | $65.12_{\pm1.25}$ | $66.44_{\pm1.48}$ | $64.66_{\pm1.55}$ |
| | vMFCoOp | $57.80_{\pm4.6}$ | $56.09_{\pm1.3}$ | $63.78_{\pm1.8}$ | $64.52_{\pm3.75}$ | $65.21_{\pm1.85}$ | $66.84_{\pm1.9}$ | $67.18_{\pm2.0}$ |
| | BiomedCLIP | | | | 57.82 | | | |
| | BiomedCLIP + Ensemble | | | | 60.57 | | | |
| | CLIP-Adapter | $51.85_{\pm3.68}$ | $53.13_{\pm3.71}$ | $53.90_{\pm3.62}$ | $53.25_{\pm3.83}$ | $55.54_{\pm3.92}$ | $55.89_{\pm1.07}$ | $58.75_{\pm1.18}$ |
| | Tip-Adapter | $52.91_{\pm2.12}$ | $60.11_{\pm4.22}$ | $69.84_{\pm1.76}$ | $66.96_{\pm1.18}$ | $71.93_{\pm1.33}$ | $72.57_{\pm1.52}$ | $72.13_{\pm1.61}$ |
| | Tip-Adapter-F | $58.44_{\pm3.93}$ | $65.74_{\pm3.17}$ | $68.58_{\pm2.14}$ | $69.98_{\pm3.87}$ | $73.05_{\pm1.18}$ | $77.48_{\pm1.29}$ | $77.50_{\pm1.34}$ |
| | Standard LP | $54.60_{\pm1.74}$ | $60.24_{\pm3.67}$ | $69.39_{\pm2.51}$ | $72.84_{\pm3.72}$ | $74.25_{\pm3.89}$ | $77.05_{\pm3.96}$ | $76.51_{\pm1.08}$ |
| Kvasir | LP++ | $59.12_{\pm3.23}$ | $67.06_{\pm3.18}$ | $71.77_{\pm3.83}$ | $72.36_{\pm2.71}$ | $74.80_{\pm1.13}$ | $76.89_{\pm1.22}$ | $77.38_{\pm1.34}$ |
| | CoOp | $55.96_{\pm1.59}$ | $62.54_{\pm1.23}$ | $64.15_{\pm3.49}$ | $71.39_{\pm1.41}$ | $76.68_{\pm1.17}$ | $79.59_{\pm1.36}$ | $77.78_{\pm1.45}$ |
| | CoCoOp | $60.80_{\pm3.1}$ | $64.07_{\pm3.21}$ | $67.44_{\pm1.29}$ | $71.25_{\pm1.47}$ | $74.72_{\pm2.06}$ | $75.70_{\pm2.12}$ | $78.57_{\pm2.14}$ |
| | KgCoOp | $63.03_{\pm2.25}$ | $69.03_{\pm1.67}$ | $70.20_{\pm3.45}$ | $69.09_{\pm1.83}$ | $68.78_{\pm1.32}$ | $79.71_{\pm1.18}$ | $77.98_{\pm1.29}$ |
| | ProGrad | $63.81_{\pm3.24}$ | $65.69_{\pm3.57}$ | $71.88_{\pm3.28}$ | $77.73_{\pm1.42}$ | $79.98_{\pm3.89}$ | $83.10_{\pm1.08}$ | $79.86_{\pm1.33}$ |
| | BiomedCoOp | $62.97_{\pm1.86}$ | $66.41_{\pm2.48}$ | $73.81_{\pm1.34}$ | $79.92_{\pm3.52}$ | $79.37_{\pm1.27}$ | $80.64_{\pm1.27}$ | $79.54_{\pm1.39}$ |
| | vMFCoOp | $63.98_{\pm1.96}$ | $67.75_{\pm2.63}$ | $78.10_{\pm1.12}$ | $80.17_{\pm3.51}$ | $81.45_{\pm1.23}$ | $82.01_{\pm1.39}$ | $82.55_{\pm1.56}$ |

Table A2: (1-6) Comparative classification accuracy (%) of vMFCoOp and competing methods across 14 benchmark datasets in the few-shot scenario. This table presents results for datasets 1–6. All experiments are conducted under the default configuration with `GPT-4` and `BiomedCLIP`.

| Dataset | Method | $K=1$ | $K=2$ | $K=4$ | $K=8$ | $K=16$ | $K=32$ | $K=64$ |
|---|---|---|---|---|---|---|---|---|
| | BiomedCLIP | | | | 39.56 | | | |
| | BiomedCLIP + Ensemble | | | | 38.36 | | | |
| | CLIP-Adapter | 35.36$_{\pm3.92}$ | 36.00$_{\pm3.87}$ | 39.53$_{\pm3.58}$ | 40.73$_{\pm1.27}$ | 47.60$_{\pm2.25}$ | 47.60$_{\pm2.1}$ | 49.92$_{\pm2.0}$ |
| | Tip-Adapter | 49.58$_{\pm9.28}$ | 67.11$_{\pm2.35}$ | 76.94$_{\pm1.05}$ | 73.97$_{\pm1.55}$ | 80.90$_{\pm1.3}$ | 81.36$_{\pm1.42}$ | 80.16$_{\pm1.48}$ |
| | Tip-Adapter-F | 56.27$_{\pm3.22}$ | 64.26$_{\pm4.65}$ | 74.63$_{\pm2.6}$ | 73.52$_{\pm2.1}$ | 78.10$_{\pm2.6}$ | 81.60$_{\pm2.12}$ | 81.03$_{\pm2.18}$ |
| | Standard LP | 64.70$_{\pm2.1}$ | 68.74$_{\pm3.4}$ | 74.19$_{\pm2.3}$ | 75.79$_{\pm3.1}$ | 80.10$_{\pm1.95}$ | 85.20$_{\pm2.05}$ | 84.01$_{\pm2.12}$ |
| CHMNIST | LP++ | 64.48$_{\pm6.25}$ | 70.53$_{\pm1.3}$ | 75.77$_{\pm6.4}$ | 76.39$_{\pm3.9}$ | 81.70$_{\pm1.6}$ | 83.64$_{\pm1.65}$ | 83.68$_{\pm1.7}$ |
| | CoOp | 61.04$_{\pm4.3}$ | 60.35$_{\pm1.2}$ | 67.29$_{\pm2.2}$ | 73.77$_{\pm3.85}$ | 82.07$_{\pm1.25}$ | 85.52$_{\pm1.3}$ | 82.89$_{\pm1.45}$ |
| | CoCoOp | 56.55$_{\pm4.4}$ | 56.59$_{\pm3.3}$ | 63.49$_{\pm2.1}$ | 71.35$_{\pm1.2}$ | 76.17$_{\pm3.55}$ | 77.62$_{\pm3.8}$ | 80.36$_{\pm3.95}$ |
| | KgCoOp | 65.08$_{\pm4.2}$ | 66.78$_{\pm1.15}$ | 74.12$_{\pm1.1}$ | 71.52$_{\pm3.12}$ | 74.73$_{\pm1.3}$ | 85.10$_{\pm1.05}$ | 83.16$_{\pm1.25}$ |
| | ProGrad | 69.21$_{\pm5.8}$ | 67.06$_{\pm1.5}$ | 76.80$_{\pm1.35}$ | 78.97$_{\pm3.45}$ | 82.08$_{\pm1.5}$ | 85.93$_{\pm1.75}$ | 82.50$_{\pm1.85}$ |
| | BiomedCoOp | 64.12$_{\pm2.55}$ | 64.52$_{\pm1.35}$ | 76.04$_{\pm1.75}$ | 82.74$_{\pm1.25}$ | 84.82$_{\pm2.15}$ | 85.39$_{\pm1.9}$ | 83.51$_{\pm2.05}$ |
| | vMFCoOp | 64.92$_{\pm2.65}$ | 63.49$_{\pm1.45}$ | 79.26$_{\pm1.85}$ | 81.57$_{\pm1.2}$ | 85.21$_{\pm2.1}$ | 85.79$_{\pm1.8}$ | 85.83$_{\pm2.0}$ |
| | BiomedCLIP | | | | 53.88 | | | |
| | BiomedCLIP + Ensemble | | | | 64.36 | | | |
| | CLIP-Adapter | 53.83$_{\pm3.42}$ | 53.20$_{\pm2.85}$ | 54.13$_{\pm1.62}$ | 56.30$_{\pm3.38}$ | 57.52$_{\pm1.05}$ | 58.03$_{\pm1.12}$ | 60.60$_{\pm1.23}$ |
| | Tip-Adapter | 73.11$_{\pm3.85}$ | 72.53$_{\pm7.2}$ | 84.92$_{\pm3.59}$ | 86.62$_{\pm1.65}$ | 88.02$_{\pm3.45}$ | 88.67$_{\pm3.6}$ | 88.21$_{\pm3.72}$ |
| | Tip-Adapter-F | 72.82$_{\pm4.1}$ | 72.23$_{\pm6.9}$ | 78.20$_{\pm9.84}$ | 84.67$_{\pm2.2}$ | 85.40$_{\pm1.05}$ | 89.76$_{\pm1.15}$ | 89.23$_{\pm1.28}$ |
| | Standard LP | 75.82$_{\pm2.55}$ | 77.35$_{\pm7.0}$ | 83.14$_{\pm3.25}$ | 84.39$_{\pm3.4}$ | 87.88$_{\pm1.1}$ | 93.40$_{\pm1.25}$ | 92.91$_{\pm1.4}$ |
| LC25000 | LP++ | 65.78$_{\pm9.27}$ | 77.07$_{\pm2.9}$ | 85.15$_{\pm2.27}$ | 88.94$_{\pm2.23}$ | 92.59$_{\pm3.35}$ | 94.77$_{\pm3.52}$ | 95.18$_{\pm3.65}$ |
| | CoOp | 70.47$_{\pm3.2}$ | 71.95$_{\pm2.63}$ | 78.81$_{\pm2.16}$ | 81.82$_{\pm3.35}$ | 90.41$_{\pm3.58}$ | 94.37$_{\pm3.55}$ | 92.19$_{\pm3.72}$ |
| | CoCoOp | 64.80$_{\pm4.1}$ | 72.03$_{\pm3.6}$ | 78.17$_{\pm2.34}$ | 85.25$_{\pm1.7}$ | 86.54$_{\pm3.5}$ | 88.12$_{\pm3.55}$ | 91.36$_{\pm3.68}$ |
| | KgCoOp | 73.03$_{\pm2.0}$ | 76.79$_{\pm1.27}$ | 82.91$_{\pm2.23}$ | 81.53$_{\pm3.25}$ | 82.43$_{\pm3.5}$ | 93.45$_{\pm3.6}$ | 92.30$_{\pm3.75}$ |
| | ProGrad | 76.96$_{\pm3.15}$ | 76.53$_{\pm1.39}$ | 87.38$_{\pm2.4}$ | 90.11$_{\pm3.8}$ | 92.93$_{\pm3.7}$ | 97.09$_{\pm3.75}$ | 94.14$_{\pm3.85}$ |
| | BiomedCoOp | 76.55$_{\pm2.76}$ | 76.85$_{\pm1.94}$ | 85.13$_{\pm1.5}$ | 90.74$_{\pm1.1}$ | 93.22$_{\pm3.6}$ | 94.64$_{\pm3.65}$ | 93.16$_{\pm3.72}$ |
| | vMFCoOp | 76.80$_{\pm2.83}$ | 75.84$_{\pm1.85}$ | 87.42$_{\pm1.55}$ | 90.02$_{\pm1.05}$ | 93.13$_{\pm3.55}$ | 94.74$_{\pm3.65}$ | 95.03$_{\pm0.8}$ |
| | BiomedCLIP | | | | 34.75 | | | |
| | BiomedCLIP + Ensemble | | | | 46.98 | | | |
| | CLIP-Adapter | 29.54$_{\pm3.55}$ | 29.86$_{\pm3.59}$ | 32.12$_{\pm3.52}$ | 30.23$_{\pm3.81}$ | 31.60$_{\pm3.48}$ | 32.51$_{\pm3.73}$ | 35.65$_{\pm3.86}$ |
| | Tip-Adapter | 28.84$_{\pm3.49}$ | 36.08$_{\pm3.75}$ | 49.92$_{\pm6.98}$ | 53.13$_{\pm7.12}$ | 58.63$_{\pm5.05}$ | 58.59$_{\pm4.98}$ | 58.00$_{\pm5.03}$ |
| | Tip-Adapter-F | 43.44$_{\pm10.11}$ | 38.99$_{\pm5.45}$ | 51.12$_{\pm6.51}$ | 55.57$_{\pm2.28}$ | 60.65$_{\pm1.27}$ | 64.23$_{\pm1.49}$ | 63.70$_{\pm1.69}$ |
| | Standard LP | 45.42$_{\pm6.52}$ | 49.71$_{\pm3.91}$ | 53.87$_{\pm6.17}$ | 53.60$_{\pm2.05}$ | 62.11$_{\pm2.69}$ | 66.48$_{\pm2.55}$ | 65.89$_{\pm2.78}$ |
| RETINA | LP++ | 43.52$_{\pm5.68}$ | 50.03$_{\pm6.77}$ | 55.12$_{\pm9.52}$ | 57.37$_{\pm1.94}$ | 64.89$_{\pm1.36}$ | 66.56$_{\pm1.49}$ | 66.68$_{\pm1.55}$ |
| | CoOp | 39.01$_{\pm1.33}$ | 36.52$_{\pm3.52}$ | 41.86$_{\pm3.05}$ | 50.87$_{\pm1.86}$ | 62.74$_{\pm3.98}$ | 65.90$_{\pm1.12}$ | 63.46$_{\pm1.29}$ |
| | CoCoOp | 40.38$_{\pm3.88}$ | 41.64$_{\pm4.18}$ | 44.50$_{\pm3.95}$ | 52.77$_{\pm1.32}$ | 57.91$_{\pm1.48}$ | 58.90$_{\pm1.65}$ | 61.85$_{\pm1.78}$ |
| | KgCoOp | 40.15$_{\pm2.83}$ | 42.55$_{\pm2.53}$ | 48.37$_{\pm3.22}$ | 52.78$_{\pm2.31}$ | 52.21$_{\pm1.67}$ | 62.77$_{\pm1.94}$ | 60.88$_{\pm2.05}$ |
| | ProGrad | 43.21$_{\pm1.98}$ | 44.06$_{\pm4.56}$ | 51.10$_{\pm3.85}$ | 59.50$_{\pm2.3}$ | 57.47$_{\pm2.46}$ | 61.49$_{\pm2.65}$ | 58.14$_{\pm2.72}$ |
| | BiomedCoOp | 40.92$_{\pm3.21}$ | 43.25$_{\pm1.92}$ | 50.67$_{\pm4.92}$ | 63.66$_{\pm1.42}$ | 67.24$_{\pm1.12}$ | 67.91$_{\pm1.23}$ | 66.28$_{\pm1.3}$ |
| | vMFCoOp | 41.70$_{\pm3.41}$ | 42.52$_{\pm1.87}$ | 54.00$_{\pm4.82}$ | 63.22$_{\pm1.35}$ | 67.86$_{\pm1.08}$ | 68.56$_{\pm1.25}$ | 68.65$_{\pm1.45}$ |
| | BiomedCLIP | | | | 37.52 | | | |
| | BiomedCLIP + Ensemble | | | | 46.86 | | | |
| | CLIP-Adapter | 32.36$_{\pm3.48}$ | 32.33$_{\pm3.51}$ | 34.90$_{\pm3.47}$ | 33.03$_{\pm3.65}$ | 34.44$_{\pm3.59}$ | 35.43$_{\pm3.52}$ | 38.25$_{\pm3.68}$ |
| | Tip-Adapter | 31.65$_{\pm3.62}$ | 36.99$_{\pm5.32}$ | 31.47$_{\pm4.12}$ | 30.47$_{\pm3.25}$ | 36.87$_{\pm7.02}$ | 37.36$_{\pm6.53}$ | 36.66$_{\pm6.3}$ |
| | Tip-Adapter-F | 33.15$_{\pm3.49}$ | 34.26$_{\pm2.31}$ | 30.27$_{\pm5.28}$ | 26.79$_{\pm1.96}$ | 26.45$_{\pm3.18}$ | 31.09$_{\pm2.83}$ | 30.57$_{\pm3.03}$ |
| | Standard LP | 30.70$_{\pm10.63}$ | 29.87$_{\pm5.18}$ | 29.89$_{\pm4.82}$ | 22.22$_{\pm3.55}$ | 24.52$_{\pm3.57}$ | 29.98$_{\pm3.52}$ | 29.72$_{\pm3.68}$ |
| KneeXray | LP++ | 28.93$_{\pm8.45}$ | 36.93$_{\pm3.22}$ | 36.42$_{\pm4.87}$ | 28.76$_{\pm2.58}$ | 31.75$_{\pm3.31}$ | 34.14$_{\pm3.38}$ | 34.63$_{\pm3.41}$ |
| | CoOp | 29.03$_{\pm9.05}$ | 27.00$_{\pm4.88}$ | 23.29$_{\pm4.38}$ | 26.12$_{\pm3.76}$ | 31.68$_{\pm1.85}$ | 35.39$_{\pm1.79}$ | 32.94$_{\pm1.87}$ |
| | CoCoOp | 32.65$_{\pm6.25}$ | 33.64$_{\pm8.07}$ | 34.44$_{\pm4.18}$ | 26.80$_{\pm8.22}$ | 28.62$_{\pm4.18}$ | 30.27$_{\pm4.02}$ | 33.31$_{\pm3.97}$ |
| | KgCoOp | 34.95$_{\pm3.28}$ | 34.51$_{\pm4.47}$ | 28.16$_{\pm2.88}$ | 25.99$_{\pm3.35}$ | 24.75$_{\pm3.52}$ | 36.37$_{\pm3.68}$ | 34.76$_{\pm3.77}$ |
| | ProGrad | 38.19$_{\pm5.76}$ | 31.11$_{\pm3.75}$ | 32.23$_{\pm2.85}$ | 32.77$_{\pm2.28}$ | 33.88$_{\pm3.16}$ | 38.33$_{\pm2.9}$ | 35.35$_{\pm3.02}$ |
| | BiomedCoOp | 38.73$_{\pm1.65}$ | 41.09$_{\pm3.59}$ | 39.22$_{\pm3.57}$ | 43.92$_{\pm3.9}$ | 43.77$_{\pm1.72}$ | 46.22$_{\pm1.78}$ | 44.48$_{\pm1.8}$ |
| | vMFCoOp | 41.22$_{\pm1.78}$ | 41.46$_{\pm3.57}$ | 43.93$_{\pm3.6}$ | 45.03$_{\pm1.08}$ | 46.26$_{\pm1.75}$ | 47.64$_{\pm1.9}$ | 47.93$_{\pm0.25}$ |
| | BiomedCLIP | | | | 33.26 | | | |
| | BiomedCLIP + Ensemble | | | | 50.67 | | | |
| | CLIP-Adapter | 42.89$_{\pm5.81}$ | 49.06$_{\pm2.47}$ | 50.47$_{\pm1.69}$ | 48.76$_{\pm3.71}$ | 54.07$_{\pm3.66}$ | 55.67$_{\pm3.72}$ | 58.68$_{\pm3.93}$ |
| | Tip-Adapter | 29.85$_{\pm3.78}$ | 33.51$_{\pm6.23}$ | 40.05$_{\pm5.04}$ | 53.38$_{\pm3.31}$ | 51.92$_{\pm4.03}$ | 53.13$_{\pm4.12}$ | 52.66$_{\pm4.34}$ |
| | Tip-Adapter-F | 45.60$_{\pm2.79}$ | 54.65$_{\pm1.79}$ | 53.32$_{\pm4.85}$ | 59.60$_{\pm6.45}$ | 65.93$_{\pm1.47}$ | 69.52$_{\pm1.59}$ | 69.72$_{\pm1.68}$ |
| | Standard LP | 47.76$_{\pm12.21}$ | 52.61$_{\pm8.44}$ | 58.29$_{\pm7.08}$ | 59.71$_{\pm9.11}$ | 64.45$_{\pm3.78}$ | 69.15$_{\pm3.89}$ | 69.13$_{\pm3.95}$ |
| OCTMNIST | LP++ | 49.19$_{\pm13.22}$ | 58.33$_{\pm9.11}$ | 61.69$_{\pm8.49}$ | 62.72$_{\pm8.15}$ | 68.11$_{\pm7.32}$ | 70.39$_{\pm7.28}$ | 70.73$_{\pm7.14}$ |
| | CoOp | 52.03$_{\pm2.98}$ | 50.50$_{\pm3.9}$ | 48.81$_{\pm2.39}$ | 59.02$_{\pm4.5}$ | 64.75$_{\pm7.5}$ | 69.58$_{\pm7.21}$ | 68.09$_{\pm7.52}$ |
| | CoCoOp | 51.02$_{\pm4.45}$ | 50.91$_{\pm7.95}$ | 47.79$_{\pm6.3}$ | 54.47$_{\pm2.0}$ | 58.79$_{\pm3.5}$ | 60.69$_{\pm3.6}$ | 63.90$_{\pm3.72}$ |
| | KgCoOp | 51.53$_{\pm3.25}$ | 52.65$_{\pm5.32}$ | 53.42$_{\pm1.6}$ | 58.02$_{\pm3.73}$ | 58.33$_{\pm3.95}$ | 69.15$_{\pm4.05}$ | 67.29$_{\pm4.25}$ |
| | ProGrad | 55.48$_{\pm3.12}$ | 57.16$_{\pm3.45}$ | 57.55$_{\pm1.3}$ | 64.52$_{\pm6.15}$ | 65.12$_{\pm6.27}$ | 68.90$_{\pm6.35}$ | 65.60$_{\pm6.45}$ |
| | BiomedCoOp | 51.57$_{\pm1.58}$ | 55.47$_{\pm4.8}$ | 55.59$_{\pm1.88}$ | 62.74$_{\pm5.45}$ | 68.62$_{\pm2.25}$ | 71.14$_{\pm2.3}$ | 69.91$_{\pm2.42}$ |
| | vMFCoOp | 52.70$_{\pm1.65}$ | 55.44$_{\pm4.9}$ | 59.38$_{\pm1.95}$ | 62.52$_{\pm5.5}$ | 70.21$_{\pm2.25}$ | 72.14$_{\pm2.35}$ | 72.58$_{\pm0.47}$ |
| | BiomedCLIP | | | | 44.66 | | | |
| | BiomedCLIP + Ensemble | | | | 47.24 | | | |
| | CLIP-Adapter | 39.89$_{\pm3.94}$ | 40.25$_{\pm3.98}$ | 42.18$_{\pm3.87}$ | 41.64$_{\pm1.06}$ | 43.90$_{\pm3.97}$ | 44.65$_{\pm3.88}$ | 47.18$_{\pm3.95}$ |
| | Tip-Adapter | 46.75$_{\pm2.43}$ | 48.01$_{\pm3.56}$ | 56.24$_{\pm3.75}$ | 58.62$_{\pm2.21}$ | 63.32$_{\pm1.37}$ | 64.44$_{\pm1.45}$ | 63.16$_{\pm1.46}$ |
| | Tip-Adapter-F | 44.60$_{\pm4.63}$ | 49.04$_{\pm5.11}$ | 55.05$_{\pm3.37}$ | 57.51$_{\pm2.58}$ | 62.92$_{\pm1.43}$ | 66.42$_{\pm1.52}$ | 66.04$_{\pm1.53}$ |
| | Standard LP | 43.13$_{\pm5.74}$ | 47.61$_{\pm6.31}$ | 54.29$_{\pm5.27}$ | 60.59$_{\pm4.45}$ | 67.20$_{\pm2.62}$ | 72.37$_{\pm2.78}$ | 71.29$_{\pm2.79}$ |
| UKB CardiacMRI | LP++ | 40.18$_{\pm3.51}$ | 52.14$_{\pm4.05}$ | 57.67$_{\pm4.15}$ | 64.34$_{\pm3.22}$ | 68.95$_{\pm2.14}$ | 71.54$_{\pm2.23}$ | 71.53$_{\pm2.34}$ |
| | CoOp | 37.17$_{\pm5.17}$ | 42.28$_{\pm2.48}$ | 48.19$_{\pm3.58}$ | 58.22$_{\pm2.61}$ | 67.89$_{\pm1.53}$ | 71.57$_{\pm1.64}$ | 68.84$_{\pm1.74}$ |
| | CoCoOp | 38.30$_{\pm2.78}$ | 43.83$_{\pm3.95}$ | 49.31$_{\pm5.04}$ | 58.25$_{\pm2.95}$ | 65.22$_{\pm1.23}$ | 66.22$_{\pm2.14}$ | 68.71$_{\pm2.35}$ |
| | KgCoOp | 45.75$_{\pm2.74}$ | 50.67$_{\pm2.82}$ | 55.62$_{\pm3.94}$ | 61.02$_{\pm4.1}$ | 62.73$_{\pm3.91}$ | 73.80$_{\pm3.94}$ | 72.21$_{\pm1.1}$ |
| | ProGrad | 48.08$_{\pm4.67}$ | 50.86$_{\pm3.34}$ | 60.55$_{\pm2.53}$ | 68.62$_{\pm1.97}$ | 70.33$_{\pm1.14}$ | 74.08$_{\pm1.26}$ | 70.35$_{\pm1.47}$ |
| | BiomedCoOp | 45.37$_{\pm2.24}$ | 49.37$_{\pm3.66}$ | 57.63$_{\pm1.92}$ | 68.24$_{\pm1.48}$ | 70.52$_{\pm1.2}$ | 72.19$_{\pm1.22}$ | 70.61$_{\pm1.21}$ |
| | vMFCoOp | 52.27$_{\pm2.43}$ | 55.68$_{\pm3.96}$ | 67.17$_{\pm2.03}$ | 73.40$_{\pm1.64}$ | 73.72$_{\pm1.23}$ | 75.69$_{\pm1.27}$ | 77.40$_{\pm1.48}$ |

Table A2: (7-12) Comparative classification accuracy (%) of vMFCoOp and competing methods across 14 benchmark datasets in the few-shot scenario. This table presents results for datasets 7–12. All experiments are conducted under the default configuration with `GPT-4` and `BiomedCLIP`.

| Dataset | Method | $K=1$ | $K=2$ | $K=4$ | $K=8$ | $K=16$ | $K=32$ | $K=64$ |
|---|---|---|---|---|---|---|---|---|
| UKB LiverMRI | BiomedCLIP | | | | 49.27 | | | |
| | BiomedCLIP + Ensemble | | | | 51.06 | | | |
| | CLIP-Adapter | $45.78_{\pm1.24}$ | $45.59_{\pm1.3}$ | $48.03_{\pm1.15}$ | $46.76_{\pm1.28}$ | $47.93_{\pm1.32}$ | $49.20_{\pm1.25}$ | $52.28_{\pm1.3}$ |
| | Tip-Adapter | $50.25_{\pm3.17}$ | $51.56_{\pm4.56}$ | $59.55_{\pm2.66}$ | $62.23_{\pm1.95}$ | $66.35_{\pm1.32}$ | $67.42_{\pm1.41}$ | $66.46_{\pm1.55}$ |
| | Tip-Adapter-F | $48.30_{\pm2.56}$ | $51.28_{\pm2.95}$ | $57.85_{\pm3.12}$ | $60.04_{\pm2.85}$ | $65.63_{\pm1.72}$ | $69.08_{\pm1.68}$ | $68.78_{\pm1.84}$ |
| | Standard LP | $48.41_{\pm5.02}$ | $52.12_{\pm6.15}$ | $58.96_{\pm4.55}$ | $61.97_{\pm3.95}$ | $69.70_{\pm2.13}$ | $74.52_{\pm2.28}$ | $73.79_{\pm2.37}$ |
| | LP++ | $45.66_{\pm3.44}$ | $56.82_{\pm3.05}$ | $62.34_{\pm4.22}$ | $65.95_{\pm3.17}$ | $71.44_{\pm1.52}$ | $73.49_{\pm1.62}$ | $73.31_{\pm1.74}$ |
| | CoOp | $45.59_{\pm2.5}$ | $46.78_{\pm2.28}$ | $51.65_{\pm3.35}$ | $59.52_{\pm2.15}$ | $71.45_{\pm1.51}$ | $75.15_{\pm1.68}$ | $72.34_{\pm1.8}$ |
| | CoCoOp | $46.62_{\pm4.05}$ | $46.69_{\pm3.2}$ | $55.79_{\pm2.95}$ | $62.98_{\pm1.85}$ | $68.61_{\pm3.98}$ | $69.84_{\pm1.08}$ | $72.64_{\pm1.18}$ |
| | KgCoOp | $49.58_{\pm1.7}$ | $49.95_{\pm1.58}$ | $49.96_{\pm1.45}$ | $54.52_{\pm2.75}$ | $54.79_{\pm1.38}$ | $65.88_{\pm1.45}$ | $64.33_{\pm1.51}$ |
| | ProGrad | $49.75_{\pm4.35}$ | $53.51_{\pm3.08}$ | $63.07_{\pm2.68}$ | $70.75_{\pm1.98}$ | $73.75_{\pm1.14}$ | $77.74_{\pm1.24}$ | $73.85_{\pm1.47}$ |
| | BiomedCoOp | $51.33_{\pm2.34}$ | $54.87_{\pm3.72}$ | $59.72_{\pm1.95}$ | $68.64_{\pm1.48}$ | $73.92_{\pm1.2}$ | $74.96_{\pm1.22}$ | $73.95_{\pm1.28}$ |
| | vMFCoOp | $55.07_{\pm2.99}$ | $57.78_{\pm3.49}$ | $67.06_{\pm2.28}$ | $71.13_{\pm1.14}$ | $76.16_{\pm1.11}$ | $79.26_{\pm1.15}$ | $80.75_{\pm1.1}$ |
| UKB PancreasMRI | BiomedCLIP | | | | 38.56 | | | |
| | BiomedCLIP + Ensemble | | | | 41.74 | | | |
| | CLIP-Adapter | $34.33_{\pm3.45}$ | $34.30_{\pm4.05}$ | $37.08_{\pm3.65}$ | $35.73_{\pm3.25}$ | $37.02_{\pm2.95}$ | $38.25_{\pm2.85}$ | $41.05_{\pm2.87}$ |
| | Tip-Adapter | $40.35_{\pm6.34}$ | $43.96_{\pm7.22}$ | $50.17_{\pm6.11}$ | $52.27_{\pm5.05}$ | $54.74_{\pm4.33}$ | $57.44_{\pm3.32}$ | $58.61_{\pm2.56}$ |
| | Tip-Adapter-F | $40.62_{\pm7.45}$ | $46.13_{\pm8.1}$ | $48.10_{\pm7.92}$ | $48.52_{\pm6.05}$ | $49.60_{\pm5.47}$ | $55.68_{\pm4.15}$ | $57.88_{\pm3.67}$ |
| | Standard LP | $41.30_{\pm8.21}$ | $44.10_{\pm9.12}$ | $48.38_{\pm8.45}$ | $48.99_{\pm7.28}$ | $52.45_{\pm6.55}$ | $59.83_{\pm5.22}$ | $60.61_{\pm4.37}$ |
| | LP++ | $39.30_{\pm7.11}$ | $51.71_{\pm8.38}$ | $57.27_{\pm7.11}$ | $57.49_{\pm6.41}$ | $60.05_{\pm5.06}$ | $64.16_{\pm4.2}$ | $65.99_{\pm3.28}$ |
| | CoOp | $35.94_{\pm6.9}$ | $41.90_{\pm7.4}$ | $48.44_{\pm6.05}$ | $51.67_{\pm5.05}$ | $57.52_{\pm4.33}$ | $64.05_{\pm3.15}$ | $63.31_{\pm2.9}$ |
| | CoCoOp | $40.45_{\pm7.02}$ | $44.24_{\pm8.12}$ | $52.29_{\pm7.15}$ | $55.77_{\pm6.45}$ | $57.47_{\pm5.28}$ | $61.37_{\pm4.35}$ | $65.96_{\pm3.72}$ |
| | KgCoOp | $42.03_{\pm3.42}$ | $44.33_{\pm4.15}$ | $46.87_{\pm3.6}$ | $52.22_{\pm4.05}$ | $52.48_{\pm3.12}$ | $64.75_{\pm2.48}$ | $64.71_{\pm2.15}$ |
| | ProGrad | $43.81_{\pm5.95}$ | $47.66_{\pm6.98}$ | $55.00_{\pm5.53}$ | $58.37_{\pm4.56}$ | $59.53_{\pm3.4}$ | $65.83_{\pm2.21}$ | $64.80_{\pm2.05}$ |
| | BiomedCoOp | $43.27_{\pm2.65}$ | $50.07_{\pm3.9}$ | $57.24_{\pm2.1}$ | $66.14_{\pm1.5}$ | $66.14_{\pm1.3}$ | $67.69_{\pm1.45}$ | $66.96_{\pm1.52}$ |
| | vMFCoOp | $48.35_{\pm2.1}$ | $53.04_{\pm1.8}$ | $64.98_{\pm1.5}$ | $69.07_{\pm1.32}$ | $70.31_{\pm1.25}$ | $71.54_{\pm1.28}$ | $70.58_{\pm1.3}$ |
| Average | BiomedCLIP | | | | 46.32 | | | |
| | BiomedCLIP + Ensemble | | | | 54.46 | | | |
| | CLIP-Adapter | $43.52_{\pm1.25}$ | $43.27_{\pm2.36}$ | $45.66_{\pm2.01}$ | $44.98_{\pm3.13}$ | $47.25_{\pm2.58}$ | $48.10_{\pm1.55}$ | $50.85_{\pm1.40}$ |
| | Tip-Adapter | $47.58_{\pm4.36}$ | $51.88_{\pm5.69}$ | $59.04_{\pm4.51}$ | $61.37_{\pm4.62}$ | $66.29_{\pm2.10}$ | $67.02_{\pm2.86}$ | $66.45_{\pm2.97}$ |
| | Tip-Adapter-F | $49.82_{\pm7.64}$ | $53.34_{\pm4.36}$ | $59.21_{\pm3.28}$ | $60.35_{\pm2.84}$ | $64.27_{\pm4.33}$ | $68.58_{\pm3.59}$ | $68.27_{\pm0.69}$ |
| | Standard LP | $49.38_{\pm5.77}$ | $52.85_{\pm5.39}$ | $58.78_{\pm3.87}$ | $60.88_{\pm7.62}$ | $65.75_{\pm4.27}$ | $70.80_{\pm3.45}$ | $70.25_{\pm2.40}$ |
| | LP++ | $49.39_{\pm7.28}$ | $58.62_{\pm5.43}$ | $62.39_{\pm3.10}$ | $64.37_{\pm5.64}$ | $69.40_{\pm2.91}$ | $71.50_{\pm2.30}$ | $71.89_{\pm2.87}$ |
| | CoOp | $47.63_{\pm4.52}$ | $49.88_{\pm3.27}$ | $54.05_{\pm2.19}$ | $60.32_{\pm1.07}$ | $68.43_{\pm1.57}$ | $72.46_{\pm1.20}$ | $70.30_{\pm3.25}$ |
| | CoCoOp | $49.43_{\pm3.25}$ | $50.77_{\pm3.29}$ | $54.69_{\pm4.79}$ | $61.08_{\pm3.49}$ | $65.09_{\pm2.87}$ | $66.59_{\pm6.50}$ | $69.75_{\pm4.10}$ |
| | KgCoOp | $52.46_{\pm3.89}$ | $54.78_{\pm3.29}$ | $58.35_{\pm4.05}$ | $60.78_{\pm6.34}$ | $60.95_{\pm7.48}$ | $71.89_{\pm3.54}$ | $70.36_{\pm2.38}$ |
| | ProGrad | $54.97_{\pm5.39}$ | $56.27_{\pm4.46}$ | $63.28_{\pm4.23}$ | $68.87_{\pm4.69}$ | $70.33_{\pm4.98}$ | $74.39_{\pm1.58}$ | $71.25_{\pm4.38}$ |
| | BiomedCoOp | $55.08_{\pm5.85}$ | $57.98_{\pm4.20}$ | $63.65_{\pm3.27}$ | $71.29_{\pm2.19}$ | $73.63_{\pm1.27}$ | $75.08_{\pm3.28}$ | $73.65_{\pm3.98}$ |
| | vMFCoOp (Ours) | $57.25_{\pm4.75}$ | $58.88_{\pm3.95}$ | $68.29_{\pm2.07}$ | $72.07_{\pm1.98}$ | $75.45_{\pm1.48}$ | $77.08_{\pm1.36}$ | $77.49_{\pm1.05}$ |

Table A2: (13–14) Comparative classification accuracy (%) of vMFCoOp and competing methods on the final two of 14 benchmark datasets under the few-shot setting. This table also includes the overall average accuracy, corresponding to Table 1 in the main paper. All experiments follow the default configuration using `GPT-4` and `BiomedCLIP`.

| Dataset | Method | $K=1$ | $K=2$ | $K=4$ | $K=8$ | $K=16$ | $K=32$ | $K=64$ |
|---|---|---|---|---|---|---|---|---|
| | MedCLIP | $63.87_{\pm0.00}$ | $63.87_{\pm0.00}$ | $63.87_{\pm0.00}$ | $63.87_{\pm0.00}$ | $63.87_{\pm0.00}$ | $63.87_{\pm0.00}$ | $63.87_{\pm0.00}$ |
| | MedCLIP + Ensemble | $65.78_{\pm0.00}$ | $65.78_{\pm0.00}$ | $65.78_{\pm0.00}$ | $65.78_{\pm0.00}$ | $65.78_{\pm0.00}$ | $65.78_{\pm0.00}$ | $65.78_{\pm0.00}$ |
| | CLIP-Adapter | $53.69_{\pm3.79}$ | $54.49_{\pm3.67}$ | $56.28_{\pm3.45}$ | $54.86_{\pm3.82}$ | $58.92_{\pm3.54}$ | $59.46_{\pm3.67}$ | $61.07_{\pm3.76}$ |
| | Tip-Adapter | $61.69_{\pm3.29}$ | $64.40_{\pm2.73}$ | $75.35_{\pm1.48}$ | $69.20_{\pm3.12}$ | $71.43_{\pm1.31}$ | $72.38_{\pm1.02}$ | $70.33_{\pm1.19}$ |
| | Tip-Adapter-F | $54.74_{\pm2.27}$ | $58.36_{\pm5.63}$ | $69.81_{\pm1.54}$ | $69.68_{\pm1.76}$ | $68.13_{\pm2.04}$ | $69.11_{\pm2.18}$ | $68.41_{\pm2.49}$ |
| | Standard LP | $59.91_{\pm4.23}$ | $67.89_{\pm5.13}$ | $68.94_{\pm2.29}$ | $67.79_{\pm3.07}$ | $70.96_{\pm2.45}$ | $74.46_{\pm2.68}$ | $72.86_{\pm2.91}$ |
| BTMRI | LP++ | $64.95_{\pm5.39}$ | $72.85_{\pm5.31}$ | $73.42_{\pm1.22}$ | $71.27_{\pm1.27}$ | $75.72_{\pm1.33}$ | $77.79_{\pm1.44}$ | $77.37_{\pm1.75}$ |
| | CoOp | $59.45_{\pm3.47}$ | $61.97_{\pm4.85}$ | $66.31_{\pm2.44}$ | $71.67_{\pm1.92}$ | $76.94_{\pm1.74}$ | $80.49_{\pm1.72}$ | $79.45_{\pm1.83}$ |
| | CoCoOp | $59.65_{\pm3.74}$ | $61.93_{\pm3.58}$ | $64.72_{\pm4.31}$ | $68.07_{\pm4.22}$ | $73.79_{\pm1.49}$ | $74.48_{\pm1.64}$ | $77.76_{\pm1.87}$ |
| | KgCoOp | $64.76_{\pm3.61}$ | $71.80_{\pm5.14}$ | $76.44_{\pm2.37}$ | $76.13_{\pm1.03}$ | $78.26_{\pm3.28}$ | $88.12_{\pm3.47}$ | $89.65_{\pm3.52}$ |
| | ProGrad | $72.51_{\pm1.98}$ | $73.89_{\pm2.89}$ | $79.52_{\pm4.93}$ | $82.01_{\pm1.58}$ | $85.81_{\pm1.04}$ | $90.67_{\pm1.18}$ | $87.20_{\pm1.47}$ |
| | BiomedCoOp | $63.10_{\pm1.66}$ | $68.13_{\pm3.84}$ | $73.92_{\pm3.63}$ | $78.29_{\pm2.08}$ | $81.88_{\pm1.23}$ | $81.92_{\pm1.29}$ | $81.82_{\pm1.38}$ |
| | vMFCoOp (Ours) | $66.74_{\pm1.72}$ | $70.95_{\pm3.97}$ | $82.05_{\pm3.72}$ | $83.27_{\pm2.07}$ | $86.64_{\pm1.18}$ | $88.98_{\pm1.34}$ | $90.17_{\pm1.45}$ |
| | MedCLIP | $67.83_{\pm0.00}$ | $67.83_{\pm0.00}$ | $67.83_{\pm0.00}$ | $67.83_{\pm0.00}$ | $67.83_{\pm0.00}$ | $67.83_{\pm0.00}$ | $67.83_{\pm0.00}$ |
| | MedCLIP + Ensemble | $64.73_{\pm0.00}$ | $64.73_{\pm0.00}$ | $64.73_{\pm0.00}$ | $64.73_{\pm0.00}$ | $64.73_{\pm0.00}$ | $64.73_{\pm0.00}$ | $64.73_{\pm0.00}$ |
| | CLIP-Adapter | $59.42_{\pm3.82}$ | $58.93_{\pm3.85}$ | $61.88_{\pm3.79}$ | $60.07_{\pm1.35}$ | $62.39_{\pm2.05}$ | $63.45_{\pm1.98}$ | $65.53_{\pm2.10}$ |
| | Tip-Adapter | $58.48_{\pm2.30}$ | $59.58_{\pm2.50}$ | $59.49_{\pm1.20}$ | $52.58_{\pm10.20}$ | $62.70_{\pm5.30}$ | $63.60_{\pm5.05}$ | $61.33_{\pm5.18}$ |
| | Tip-Adapter-F | $57.86_{\pm2.11}$ | $54.06_{\pm6.82}$ | $58.74_{\pm6.53}$ | $60.56_{\pm2.24}$ | $59.07_{\pm1.32}$ | $61.98_{\pm1.20}$ | $61.24_{\pm1.30}$ |
| | Standard LP | $49.50_{\pm10.55}$ | $44.03_{\pm6.07}$ | $47.55_{\pm7.12}$ | $56.88_{\pm6.20}$ | $59.03_{\pm1.75}$ | $63.25_{\pm1.88}$ | $61.43_{\pm1.97}$ |
| BUSI | LP++ | $51.65_{\pm5.13}$ | $57.65_{\pm2.28}$ | $59.39_{\pm3.05}$ | $61.36_{\pm2.24}$ | $64.75_{\pm1.62}$ | $68.02_{\pm1.70}$ | $67.60_{\pm1.85}$ |
| | CoOp | $45.16_{\pm3.05}$ | $47.78_{\pm2.78}$ | $53.08_{\pm3.48}$ | $57.59_{\pm5.95}$ | $64.86_{\pm3.12}$ | $68.90_{\pm3.40}$ | $67.82_{\pm3.50}$ |
| | CoCoOp | $53.31_{\pm3.53}$ | $48.13_{\pm2.59}$ | $58.00_{\pm1.78}$ | $63.74_{\pm3.48}$ | $67.32_{\pm1.10}$ | $68.15_{\pm1.25}$ | $71.20_{\pm1.30}$ |
| | KgCoOp | $55.99_{\pm7.12}$ | $58.15_{\pm2.97}$ | $63.96_{\pm4.28}$ | $65.25_{\pm2.22}$ | $68.46_{\pm1.98}$ | $78.78_{\pm2.35}$ | $79.98_{\pm2.40}$ |
| | ProGrad | $52.35_{\pm4.05}$ | $52.83_{\pm7.05}$ | $66.75_{\pm7.18}$ | $68.42_{\pm4.05}$ | $75.03_{\pm2.60}$ | $79.98_{\pm2.60}$ | $76.72_{\pm2.90}$ |
| | BiomedCoOp | $49.22_{\pm1.62}$ | $48.90_{\pm6.98}$ | $56.98_{\pm1.15}$ | $64.41_{\pm4.55}$ | $69.95_{\pm2.28}$ | $70.74_{\pm2.25}$ | $70.83_{\pm2.35}$ |
| | vMFCoOp (Ours) | $54.18_{\pm1.73}$ | $52.79_{\pm7.01}$ | $65.19_{\pm1.07}$ | $68.95_{\pm4.53}$ | $75.65_{\pm2.12}$ | $77.75_{\pm2.29}$ | $78.92_{\pm2.34}$ |
| | MedCLIP | $50.58_{\pm0.00}$ | $50.58_{\pm0.00}$ | $50.58_{\pm0.00}$ | $50.58_{\pm0.00}$ | $50.58_{\pm0.00}$ | $50.58_{\pm0.00}$ | $50.58_{\pm0.00}$ |
| | MedCLIP + Ensemble | $72.43_{\pm0.00}$ | $72.43_{\pm0.00}$ | $72.43_{\pm0.00}$ | $72.43_{\pm0.00}$ | $72.43_{\pm0.00}$ | $72.43_{\pm0.00}$ | $72.43_{\pm0.00}$ |
| | CLIP-Adapter | $47.30_{\pm1.47}$ | $40.24_{\pm1.03}$ | $45.48_{\pm3.17}$ | $45.76_{\pm1.13}$ | $47.82_{\pm1.27}$ | $49.84_{\pm1.15}$ | $51.69_{\pm1.31}$ |
| | Tip-Adapter | $57.20_{\pm7.59}$ | $55.91_{\pm5.04}$ | $63.29_{\pm9.98}$ | $62.53_{\pm5.27}$ | $67.38_{\pm1.17}$ | $66.60_{\pm1.42}$ | $64.44_{\pm1.79}$ |
| | Tip-Adapter-F | $50.09_{\pm16.87}$ | $50.81_{\pm7.53}$ | $62.66_{\pm4.01}$ | $60.84_{\pm3.98}$ | $64.30_{\pm3.11}$ | $64.60_{\pm3.19}$ | $64.06_{\pm3.46}$ |
| | Standard LP | $47.30_{\pm10.55}$ | $43.49_{\pm15.93}$ | $53.10_{\pm12.67}$ | $58.91_{\pm5.84}$ | $62.79_{\pm1.89}$ | $65.41_{\pm2.17}$ | $63.76_{\pm2.34}$ |
| COVID-QU-Ex | LP++ | $46.09_{\pm10.42}$ | $57.48_{\pm14.47}$ | $60.18_{\pm9.08}$ | $60.23_{\pm8.23}$ | $66.57_{\pm1.11}$ | $68.90_{\pm1.36}$ | $68.27_{\pm1.57}$ |
| | CoOp | $54.44_{\pm13.95}$ | $51.88_{\pm7.76}$ | $58.97_{\pm6.29}$ | $67.16_{\pm3.33}$ | $72.08_{\pm1.47}$ | $75.03_{\pm1.84}$ | $74.07_{\pm2.12}$ |
| | CoCoOp | $69.54_{\pm2.53}$ | $66.74_{\pm2.47}$ | $60.68_{\pm9.67}$ | $66.46_{\pm3.05}$ | $70.79_{\pm3.68}$ | $71.15_{\pm3.95}$ | $74.00_{\pm1.13}$ |
| | KgCoOp | $63.36_{\pm9.24}$ | $56.27_{\pm11.75}$ | $66.43_{\pm8.37}$ | $72.88_{\pm3.35}$ | $73.67_{\pm3.93}$ | $83.46_{\pm1.12}$ | $84.74_{\pm1.27}$ |
| | ProGrad | $65.73_{\pm11.27}$ | $67.08_{\pm5.98}$ | $71.85_{\pm3.05}$ | $78.12_{\pm1.18}$ | $78.46_{\pm1.21}$ | $82.83_{\pm1.41}$ | $79.24_{\pm1.63}$ |
| | BiomedCoOp | $70.13_{\pm2.28}$ | $68.61_{\pm1.28}$ | $70.11_{\pm2.07}$ | $77.56_{\pm3.48}$ | $78.48_{\pm3.31}$ | $78.14_{\pm3.62}$ | $77.93_{\pm3.79}$ |
| | vMFCoOp (Ours) | $74.01_{\pm2.36}$ | $71.67_{\pm1.54}$ | $77.89_{\pm2.22}$ | $81.68_{\pm3.52}$ | $82.72_{\pm3.34}$ | $84.92_{\pm3.67}$ | $85.86_{\pm0.82}$ |
| | MedCLIP | $49.83_{\pm0.00}$ | $49.83_{\pm0.00}$ | $49.83_{\pm0.00}$ | $49.83_{\pm0.00}$ | $49.83_{\pm0.00}$ | $49.83_{\pm0.00}$ | $49.83_{\pm0.00}$ |
| | MedCLIP + Ensemble | $61.89_{\pm0.00}$ | $61.89_{\pm0.00}$ | $61.89_{\pm0.00}$ | $61.89_{\pm0.00}$ | $61.89_{\pm0.00}$ | $61.89_{\pm0.00}$ | $61.89_{\pm0.00}$ |
| | CLIP-Adapter | $42.99_{\pm3.71}$ | $36.48_{\pm1.79}$ | $40.50_{\pm1.98}$ | $40.90_{\pm3.68}$ | $44.40_{\pm1.22}$ | $45.57_{\pm1.61}$ | $47.18_{\pm1.81}$ |
| | Tip-Adapter | $38.49_{\pm4.47}$ | $46.63_{\pm7.18}$ | $52.99_{\pm3.84}$ | $63.48_{\pm8.22}$ | $68.08_{\pm7.65}$ | $65.57_{\pm7.12}$ | $62.24_{\pm6.94}$ |
| | Tip-Adapter-F | $42.73_{\pm6.54}$ | $54.27_{\pm7.92}$ | $52.98_{\pm9.67}$ | $67.47_{\pm6.42}$ | $68.26_{\pm3.11}$ | $71.85_{\pm3.28}$ | $68.41_{\pm3.46}$ |
| | Standard LP | $39.68_{\pm5.23}$ | $53.83_{\pm5.98}$ | $62.00_{\pm6.84}$ | $67.62_{\pm7.12}$ | $73.06_{\pm5.31}$ | $73.64_{\pm5.02}$ | $72.34_{\pm5.17}$ |
| CTKIDNEY | LP++ | $55.14_{\pm2.78}$ | $63.59_{\pm3.42}$ | $62.52_{\pm8.04}$ | $69.77_{\pm7.67}$ | $73.69_{\pm7.05}$ | $72.70_{\pm6.74}$ | $71.37_{\pm6.56}$ |
| | CoOp | $48.06_{\pm8.15}$ | $54.78_{\pm2.36}$ | $58.21_{\pm2.47}$ | $67.61_{\pm3.72}$ | $76.99_{\pm1.93}$ | $78.39_{\pm1.65}$ | $78.93_{\pm1.52}$ |
| | CoCoOp | $46.60_{\pm6.88}$ | $49.29_{\pm9.27}$ | $57.84_{\pm1.22}$ | $70.12_{\pm1.45}$ | $73.29_{\pm2.58}$ | $73.00_{\pm2.42}$ | $76.81_{\pm2.57}$ |
| | KgCoOp | $60.82_{\pm1.22}$ | $63.11_{\pm3.05}$ | $68.46_{\pm5.46}$ | $75.65_{\pm4.15}$ | $73.29_{\pm2.58}$ | $83.24_{\pm2.82}$ | $84.81_{\pm2.67}$ |
| | ProGrad | $57.39_{\pm8.13}$ | $65.21_{\pm4.89}$ | $70.43_{\pm1.85}$ | $82.09_{\pm4.05}$ | $85.53_{\pm2.43}$ | $86.19_{\pm2.98}$ | $82.49_{\pm2.65}$ |
| | BiomedCoOp | $53.28_{\pm4.28}$ | $60.70_{\pm5.13}$ | $63.60_{\pm1.91}$ | $77.83_{\pm3.98}$ | $81.81_{\pm2.33}$ | $80.68_{\pm2.37}$ | $80.51_{\pm2.47}$ |
| | vMFCoOp (Ours) | $60.09_{\pm4.47}$ | $66.42_{\pm5.44}$ | $73.18_{\pm2.13}$ | $83.71_{\pm4.35}$ | $88.44_{\pm2.55}$ | $91.92_{\pm2.68}$ | $92.14_{\pm0.72}$ |
| | MedCLIP | $46.04_{\pm0.00}$ | $46.04_{\pm0.00}$ | $46.04_{\pm0.00}$ | $46.04_{\pm0.00}$ | $46.04_{\pm0.00}$ | $46.04_{\pm0.00}$ | $46.04_{\pm0.00}$ |
| | MedCLIP + Ensemble | $59.34_{\pm0.00}$ | $59.34_{\pm0.00}$ | $59.34_{\pm0.00}$ | $59.34_{\pm0.00}$ | $59.34_{\pm0.00}$ | $59.34_{\pm0.00}$ | $59.34_{\pm0.00}$ |
| | CLIP-Adapter | $33.10_{\pm6.14}$ | $33.47_{\pm6.05}$ | $34.32_{\pm3.58}$ | $31.99_{\pm6.01}$ | $27.70_{\pm3.12}$ | $28.55_{\pm3.45}$ | $29.70_{\pm3.89}$ |
| | Tip-Adapter | $35.19_{\pm2.30}$ | $37.76_{\pm12.48}$ | $46.37_{\pm6.02}$ | $57.52_{\pm5.28}$ | $57.75_{\pm1.20}$ | $56.91_{\pm1.45}$ | $54.77_{\pm1.37}$ |
| | Tip-Adapter-F | $35.28_{\pm15.12}$ | $35.39_{\pm3.99}$ | $43.79_{\pm4.69}$ | $34.49_{\pm2.02}$ | $42.83_{\pm4.45}$ | $43.58_{\pm4.18}$ | $42.27_{\pm4.10}$ |
| | Standard LP | $28.02_{\pm12.80}$ | $33.90_{\pm9.95}$ | $43.12_{\pm8.05}$ | $43.87_{\pm3.12}$ | $44.85_{\pm3.17}$ | $48.22_{\pm3.40}$ | $45.34_{\pm3.24}$ |
| DermaMNIST | LP++ | $26.63_{\pm3.54}$ | $29.72_{\pm11.10}$ | $33.41_{\pm8.67}$ | $39.57_{\pm2.55}$ | $45.86_{\pm1.97}$ | $47.42_{\pm2.05}$ | $46.30_{\pm2.14}$ |
| | CoOp | $21.77_{\pm8.75}$ | $32.34_{\pm5.65}$ | $37.95_{\pm6.05}$ | $38.16_{\pm6.01}$ | $45.95_{\pm2.30}$ | $48.92_{\pm2.45}$ | $47.03_{\pm2.61}$ |
| | CoCoOp | $24.83_{\pm4.11}$ | $22.94_{\pm3.55}$ | $22.68_{\pm5.21}$ | $37.75_{\pm2.00}$ | $38.24_{\pm6.10}$ | $38.10_{\pm5.95}$ | $40.75_{\pm5.72}$ |
| | KgCoOp | $28.93_{\pm10.32}$ | $32.52_{\pm4.11}$ | $36.28_{\pm7.65}$ | $35.96_{\pm4.50}$ | $35.97_{\pm2.04}$ | $44.98_{\pm2.18}$ | $45.88_{\pm2.25}$ |
| | ProGrad | $39.14_{\pm10.20}$ | $40.53_{\pm6.12}$ | $47.55_{\pm10.21}$ | $53.90_{\pm2.09}$ | $49.53_{\pm4.80}$ | $54.78_{\pm4.90}$ | $50.92_{\pm5.00}$ |
| | BiomedCoOp | $56.46_{\pm4.21}$ | $54.49_{\pm1.15}$ | $59.26_{\pm1.95}$ | $62.31_{\pm3.67}$ | $63.63_{\pm1.25}$ | $63.34_{\pm1.48}$ | $62.93_{\pm1.55}$ |
| | vMFCoOp (Ours) | $59.87_{\pm4.60}$ | $57.75_{\pm1.30}$ | $65.61_{\pm1.80}$ | $66.83_{\pm3.75}$ | $66.87_{\pm1.85}$ | $69.00_{\pm1.90}$ | $69.86_{\pm2.00}$ |
| | MedCLIP | $61.62_{\pm0.00}$ | $61.62_{\pm0.00}$ | $61.62_{\pm0.00}$ | $61.62_{\pm0.00}$ | $61.62_{\pm0.00}$ | $61.62_{\pm0.00}$ | $61.62_{\pm0.00}$ |
| | MedCLIP + Ensemble | $62.48_{\pm0.00}$ | $62.48_{\pm0.00}$ | $62.48_{\pm0.00}$ | $62.48_{\pm0.00}$ | $62.48_{\pm0.00}$ | $62.48_{\pm0.00}$ | $62.48_{\pm0.00}$ |
| | CLIP-Adapter | $50.46_{\pm3.68}$ | $51.44_{\pm3.71}$ | $52.22_{\pm3.62}$ | $51.32_{\pm3.83}$ | $53.41_{\pm3.92}$ | $54.04_{\pm1.07}$ | $55.88_{\pm1.18}$ |
| | Tip-Adapter | $50.56_{\pm2.12}$ | $57.68_{\pm4.22}$ | $67.84_{\pm1.76}$ | $63.72_{\pm1.18}$ | $66.31_{\pm1.33}$ | $66.13_{\pm1.52}$ | $63.90_{\pm1.61}$ |
| | Tip-Adapter-F | $55.73_{\pm3.93}$ | $62.27_{\pm3.17}$ | $63.82_{\pm2.14}$ | $66.85_{\pm3.87}$ | $67.17_{\pm1.18}$ | $68.66_{\pm1.29}$ | $68.11_{\pm1.34}$ |
| | Standard LP | $51.59_{\pm1.74}$ | $57.36_{\pm3.67}$ | $65.82_{\pm2.51}$ | $69.41_{\pm3.72}$ | $68.83_{\pm3.89}$ | $69.40_{\pm3.96}$ | $67.73_{\pm1.08}$ |
| Kvasir | LP++ | $56.95_{\pm3.23}$ | $63.31_{\pm3.18}$ | $67.51_{\pm3.83}$ | $67.43_{\pm2.71}$ | $68.66_{\pm1.13}$ | $70.77_{\pm1.22}$ | $70.08_{\pm1.34}$ |
| | CoOp | $53.61_{\pm1.59}$ | $60.59_{\pm1.23}$ | $62.21_{\pm3.49}$ | $69.41_{\pm1.41}$ | $73.47_{\pm1.17}$ | $75.27_{\pm1.36}$ | $74.76_{\pm1.45}$ |
| | CoCoOp | $59.49_{\pm3.10}$ | $62.44_{\pm3.21}$ | $65.73_{\pm1.29}$ | $69.24_{\pm1.47}$ | $71.97_{\pm2.06}$ | $71.98_{\pm2.12}$ | $74.71_{\pm2.14}$ |
| | KgCoOp | $63.94_{\pm2.25}$ | $69.47_{\pm1.67}$ | $71.06_{\pm3.45}$ | $69.42_{\pm1.83}$ | $70.30_{\pm1.32}$ | $80.34_{\pm1.18}$ | $81.50_{\pm1.29}$ |
| | ProGrad | $65.02_{\pm3.24}$ | $66.76_{\pm3.57}$ | $73.03_{\pm3.28}$ | $78.08_{\pm1.42}$ | $80.93_{\pm3.89}$ | $84.20_{\pm1.08}$ | $80.58_{\pm1.33}$ |
| | BiomedCoOp | $62.16_{\pm1.86}$ | $64.60_{\pm2.48}$ | $71.38_{\pm1.34}$ | $77.74_{\pm3.52}$ | $77.88_{\pm1.27}$ | $77.54_{\pm1.27}$ | $77.81_{\pm1.39}$ |
| | vMFCoOp (Ours) | $66.05_{\pm1.96}$ | $69.41_{\pm2.63}$ | $79.93_{\pm1.12}$ | $82.48_{\pm3.51}$ | $83.11_{\pm1.23}$ | $84.17_{\pm1.39}$ | $85.23_{\pm1.56}$ |

Table A3: (1-6) Comparative classification accuracy (%) of vMFCoOp and competing methods across 14 benchmark datasets in the few-shot scenario. This table presents results for datasets 1–6. All experiments are conducted under the configuration with `Qwen-2.5` and `MedCLIP`.

| Dataset | Method | $K = 1$ | $K = 2$ | $K = 4$ | $K = 8$ | $K = 16$ | $K = 32$ | $K = 64$ |
|---|---|---|---|---|---|---|---|---|
| | MedCLIP | $43.36_{\pm 0.00}$ | $43.36_{\pm 0.00}$ | $43.36_{\pm 0.00}$ | $43.36_{\pm 0.00}$ | $43.36_{\pm 0.00}$ | $43.36_{\pm 0.00}$ | $43.36_{\pm 0.00}$ |
| | MedCLIP + Ensemble | $40.27_{\pm 0.00}$ | $40.27_{\pm 0.00}$ | $40.27_{\pm 0.00}$ | $40.27_{\pm 0.00}$ | $40.27_{\pm 0.00}$ | $40.27_{\pm 0.00}$ | $40.27_{\pm 0.00}$ |
| | CLIP-Adapter | $33.97_{\pm 3.92}$ | $34.31_{\pm 3.87}$ | $37.85_{\pm 3.58}$ | $38.80_{\pm 1.27}$ | $45.47_{\pm 2.25}$ | $45.75_{\pm 2.10}$ | $47.05_{\pm 2.00}$ |
| | Tip-Adapter | $47.23_{\pm 9.28}$ | $64.68_{\pm 2.35}$ | $74.94_{\pm 1.05}$ | $70.73_{\pm 1.55}$ | $75.28_{\pm 1.30}$ | $74.92_{\pm 1.42}$ | $71.93_{\pm 1.48}$ |
| | Tip-Adapter-F | $53.56_{\pm 3.22}$ | $60.79_{\pm 4.65}$ | $69.87_{\pm 2.60}$ | $70.39_{\pm 2.10}$ | $72.22_{\pm 2.60}$ | $72.78_{\pm 2.12}$ | $71.64_{\pm 2.18}$ |
| | Standard LP | $61.69_{\pm 2.10}$ | $65.86_{\pm 3.40}$ | $70.62_{\pm 2.30}$ | $72.36_{\pm 3.10}$ | $74.68_{\pm 1.95}$ | $77.55_{\pm 2.05}$ | $75.23_{\pm 2.12}$ |
| CHMNIST | LP++ | $62.31_{\pm 6.25}$ | $66.78_{\pm 1.30}$ | $71.51_{\pm 6.40}$ | $71.46_{\pm 3.90}$ | $75.56_{\pm 1.60}$ | $77.52_{\pm 1.65}$ | $76.38_{\pm 1.70}$ |
| | CoOp | $58.69_{\pm 4.30}$ | $58.40_{\pm 1.20}$ | $65.35_{\pm 2.20}$ | $71.79_{\pm 3.85}$ | $78.86_{\pm 1.25}$ | $81.20_{\pm 1.30}$ | $79.87_{\pm 1.45}$ |
| | CoCoOp | $55.24_{\pm 4.40}$ | $54.96_{\pm 3.30}$ | $61.78_{\pm 2.10}$ | $69.34_{\pm 1.20}$ | $73.42_{\pm 3.55}$ | $73.90_{\pm 3.80}$ | $76.50_{\pm 3.95}$ |
| | KgCoOp | $65.99_{\pm 4.20}$ | $67.22_{\pm 1.15}$ | $74.98_{\pm 1.10}$ | $71.85_{\pm 3.12}$ | $76.25_{\pm 1.30}$ | $85.73_{\pm 1.05}$ | $86.68_{\pm 1.25}$ |
| | ProGrad | $70.42_{\pm 5.80}$ | $68.13_{\pm 1.50}$ | $77.95_{\pm 1.35}$ | $79.32_{\pm 3.45}$ | $83.03_{\pm 1.50}$ | $87.03_{\pm 1.75}$ | $83.22_{\pm 1.85}$ |
| | BiomedCoOp | $63.31_{\pm 2.55}$ | $62.71_{\pm 1.35}$ | $73.61_{\pm 1.75}$ | $80.56_{\pm 1.25}$ | $83.33_{\pm 2.15}$ | $82.29_{\pm 1.90}$ | $81.78_{\pm 2.05}$ |
| | vMFCoOp (Ours) | $66.99_{\pm 2.65}$ | $65.15_{\pm 1.45}$ | $81.09_{\pm 1.85}$ | $83.88_{\pm 1.20}$ | $86.87_{\pm 2.10}$ | $87.95_{\pm 1.80}$ | $88.51_{\pm 2.00}$ |
| | MedCLIP | $57.68_{\pm 0.00}$ | $57.68_{\pm 0.00}$ | $57.68_{\pm 0.00}$ | $57.68_{\pm 0.00}$ | $57.68_{\pm 0.00}$ | $57.68_{\pm 0.00}$ | $57.68_{\pm 0.00}$ |
| | MedCLIP + Ensemble | $66.27_{\pm 0.00}$ | $66.27_{\pm 0.00}$ | $66.27_{\pm 0.00}$ | $66.27_{\pm 0.00}$ | $66.27_{\pm 0.00}$ | $66.27_{\pm 0.00}$ | $66.27_{\pm 0.00}$ |
| | CLIP-Adapter | $52.44_{\pm 3.42}$ | $51.51_{\pm 2.85}$ | $52.45_{\pm 1.62}$ | $54.37_{\pm 3.38}$ | $55.39_{\pm 1.05}$ | $56.18_{\pm 1.12}$ | $57.73_{\pm 1.23}$ |
| | Tip-Adapter | $70.76_{\pm 3.85}$ | $70.10_{\pm 7.20}$ | $82.92_{\pm 3.59}$ | $83.38_{\pm 1.65}$ | $82.40_{\pm 3.45}$ | $82.23_{\pm 3.60}$ | $79.98_{\pm 3.72}$ |
| | Tip-Adapter-F | $70.11_{\pm 4.10}$ | $68.76_{\pm 6.90}$ | $73.44_{\pm 9.84}$ | $81.54_{\pm 2.20}$ | $79.52_{\pm 1.05}$ | $80.94_{\pm 1.15}$ | $79.84_{\pm 1.28}$ |
| | Standard LP | $72.81_{\pm 2.55}$ | $74.47_{\pm 7.00}$ | $79.57_{\pm 3.25}$ | $80.96_{\pm 3.40}$ | $82.46_{\pm 1.10}$ | $85.75_{\pm 1.25}$ | $84.13_{\pm 1.40}$ |
| LC25000 | LP++ | $63.61_{\pm 9.27}$ | $73.32_{\pm 2.90}$ | $80.89_{\pm 2.27}$ | $84.01_{\pm 2.23}$ | $86.45_{\pm 3.35}$ | $88.65_{\pm 3.52}$ | $87.88_{\pm 3.65}$ |
| | CoOp | $68.12_{\pm 3.20}$ | $70.00_{\pm 2.63}$ | $76.87_{\pm 2.16}$ | $79.84_{\pm 3.35}$ | $87.20_{\pm 3.58}$ | $90.05_{\pm 3.55}$ | $89.17_{\pm 3.72}$ |
| | CoCoOp | $63.49_{\pm 4.10}$ | $70.40_{\pm 3.60}$ | $76.46_{\pm 2.34}$ | $83.24_{\pm 1.70}$ | $83.79_{\pm 3.50}$ | $84.40_{\pm 3.55}$ | $87.50_{\pm 3.68}$ |
| | KgCoOp | $73.94_{\pm 2.00}$ | $77.23_{\pm 1.27}$ | $83.77_{\pm 2.23}$ | $81.86_{\pm 3.25}$ | $83.95_{\pm 3.50}$ | $94.08_{\pm 3.60}$ | $95.82_{\pm 3.75}$ |
| | ProGrad | $78.17_{\pm 3.15}$ | $77.60_{\pm 1.39}$ | $88.53_{\pm 2.40}$ | $90.46_{\pm 3.80}$ | $93.88_{\pm 3.70}$ | $98.19_{\pm 3.75}$ | $94.86_{\pm 3.85}$ |
| | BiomedCoOp | $75.74_{\pm 2.76}$ | $75.04_{\pm 1.94}$ | $82.70_{\pm 1.50}$ | $88.56_{\pm 1.10}$ | $91.73_{\pm 3.60}$ | $91.54_{\pm 3.65}$ | $91.43_{\pm 3.72}$ |
| | vMFCoOp (Ours) | $78.87_{\pm 2.83}$ | $77.50_{\pm 1.85}$ | $89.25_{\pm 1.55}$ | $92.33_{\pm 1.05}$ | $94.79_{\pm 3.55}$ | $96.90_{\pm 3.65}$ | $97.71_{\pm 0.80}$ |
| | MedCLIP | $38.55_{\pm 0.00}$ | $38.55_{\pm 0.00}$ | $38.55_{\pm 0.00}$ | $38.55_{\pm 0.00}$ | $38.55_{\pm 0.00}$ | $38.55_{\pm 0.00}$ | $38.55_{\pm 0.00}$ |
| | MedCLIP + Ensemble | $48.89_{\pm 0.00}$ | $48.89_{\pm 0.00}$ | $48.89_{\pm 0.00}$ | $48.89_{\pm 0.00}$ | $48.89_{\pm 0.00}$ | $48.89_{\pm 0.00}$ | $48.89_{\pm 0.00}$ |
| | CLIP-Adapter | $28.15_{\pm 3.55}$ | $28.17_{\pm 3.59}$ | $30.44_{\pm 3.52}$ | $28.30_{\pm 3.81}$ | $29.47_{\pm 3.48}$ | $30.66_{\pm 3.73}$ | $32.78_{\pm 3.86}$ |
| | Tip-Adapter | $26.49_{\pm 3.49}$ | $33.65_{\pm 3.75}$ | $47.92_{\pm 6.98}$ | $49.89_{\pm 7.12}$ | $53.01_{\pm 5.05}$ | $52.15_{\pm 4.98}$ | $49.77_{\pm 5.03}$ |
| | Tip-Adapter-F | $40.73_{\pm 10.11}$ | $35.52_{\pm 5.45}$ | $46.36_{\pm 6.51}$ | $52.44_{\pm 2.28}$ | $54.77_{\pm 1.27}$ | $55.41_{\pm 1.49}$ | $54.31_{\pm 1.69}$ |
| | Standard LP | $42.41_{\pm 6.52}$ | $46.83_{\pm 3.91}$ | $50.30_{\pm 6.17}$ | $50.17_{\pm 2.05}$ | $56.69_{\pm 2.69}$ | $58.83_{\pm 2.55}$ | $57.11_{\pm 2.78}$ |
| RETINA | LP++ | $41.35_{\pm 5.68}$ | $46.28_{\pm 6.77}$ | $50.86_{\pm 9.52}$ | $52.44_{\pm 1.94}$ | $58.74_{\pm 1.36}$ | $60.44_{\pm 1.49}$ | $59.38_{\pm 1.55}$ |
| | CoOp | $36.66_{\pm 1.33}$ | $34.57_{\pm 3.52}$ | $39.92_{\pm 3.05}$ | $48.89_{\pm 1.86}$ | $59.53_{\pm 3.98}$ | $61.58_{\pm 1.12}$ | $60.44_{\pm 1.29}$ |
| | CoCoOp | $39.07_{\pm 3.88}$ | $40.01_{\pm 4.18}$ | $42.79_{\pm 3.95}$ | $50.76_{\pm 1.32}$ | $55.16_{\pm 1.48}$ | $55.18_{\pm 1.65}$ | $57.99_{\pm 1.78}$ |
| | KgCoOp | $41.06_{\pm 2.83}$ | $42.99_{\pm 2.53}$ | $49.23_{\pm 3.22}$ | $53.11_{\pm 2.31}$ | $53.73_{\pm 1.67}$ | $63.40_{\pm 1.94}$ | $64.40_{\pm 2.05}$ |
| | ProGrad | $44.42_{\pm 1.98}$ | $45.13_{\pm 4.56}$ | $52.25_{\pm 3.85}$ | $59.85_{\pm 2.30}$ | $58.42_{\pm 2.46}$ | $62.59_{\pm 2.65}$ | $58.86_{\pm 2.72}$ |
| | BiomedCoOp | $40.11_{\pm 3.21}$ | $41.44_{\pm 1.92}$ | $48.24_{\pm 4.92}$ | $61.48_{\pm 1.42}$ | $65.75_{\pm 1.12}$ | $64.81_{\pm 1.23}$ | $64.55_{\pm 1.30}$ |
| | vMFCoOp (Ours) | $43.77_{\pm 3.41}$ | $44.18_{\pm 1.87}$ | $55.83_{\pm 4.82}$ | $65.53_{\pm 1.35}$ | $69.52_{\pm 1.08}$ | $70.72_{\pm 1.25}$ | $71.33_{\pm 1.45}$ |
| | MedCLIP | $41.32_{\pm 0.00}$ | $41.32_{\pm 0.00}$ | $41.32_{\pm 0.00}$ | $41.32_{\pm 0.00}$ | $41.32_{\pm 0.00}$ | $41.32_{\pm 0.00}$ | $41.32_{\pm 0.00}$ |
| | MedCLIP + Ensemble | $48.77_{\pm 0.00}$ | $48.77_{\pm 0.00}$ | $48.77_{\pm 0.00}$ | $48.77_{\pm 0.00}$ | $48.77_{\pm 0.00}$ | $48.77_{\pm 0.00}$ | $48.77_{\pm 0.00}$ |
| | CLIP-Adapter | $30.97_{\pm 3.48}$ | $30.64_{\pm 3.51}$ | $33.22_{\pm 3.47}$ | $31.10_{\pm 3.65}$ | $32.31_{\pm 3.59}$ | $33.58_{\pm 3.52}$ | $35.38_{\pm 3.68}$ |
| | Tip-Adapter | $29.30_{\pm 3.62}$ | $34.56_{\pm 5.32}$ | $29.47_{\pm 4.12}$ | $27.23_{\pm 3.25}$ | $31.25_{\pm 7.02}$ | $30.92_{\pm 6.53}$ | $28.43_{\pm 6.30}$ |
| | Tip-Adapter-F | $30.44_{\pm 3.49}$ | $30.79_{\pm 2.31}$ | $25.51_{\pm 5.28}$ | $23.66_{\pm 1.96}$ | $20.57_{\pm 3.18}$ | $22.27_{\pm 2.83}$ | $21.18_{\pm 3.03}$ |
| | Standard LP | $27.69_{\pm 10.63}$ | $26.99_{\pm 5.18}$ | $26.32_{\pm 4.82}$ | $18.79_{\pm 3.55}$ | $19.10_{\pm 3.57}$ | $22.33_{\pm 3.52}$ | $20.94_{\pm 3.68}$ |
| KneeXray | LP++ | $26.76_{\pm 8.45}$ | $33.18_{\pm 3.22}$ | $32.16_{\pm 4.87}$ | $23.83_{\pm 2.58}$ | $25.61_{\pm 3.31}$ | $28.02_{\pm 3.38}$ | $27.33_{\pm 3.41}$ |
| | CoOp | $26.68_{\pm 9.05}$ | $25.05_{\pm 4.88}$ | $21.35_{\pm 4.38}$ | $24.14_{\pm 3.76}$ | $28.47_{\pm 1.85}$ | $31.07_{\pm 1.79}$ | $29.92_{\pm 1.87}$ |
| | CoCoOp | $31.34_{\pm 6.25}$ | $32.01_{\pm 8.07}$ | $32.73_{\pm 4.18}$ | $24.79_{\pm 8.22}$ | $25.87_{\pm 4.18}$ | $26.55_{\pm 4.02}$ | $29.45_{\pm 3.97}$ |
| | KgCoOp | $35.86_{\pm 3.28}$ | $34.95_{\pm 4.47}$ | $29.02_{\pm 2.88}$ | $26.32_{\pm 3.35}$ | $26.27_{\pm 3.52}$ | $37.00_{\pm 3.68}$ | $38.28_{\pm 3.77}$ |
| | ProGrad | $39.40_{\pm 5.76}$ | $32.18_{\pm 3.75}$ | $33.38_{\pm 2.85}$ | $33.12_{\pm 2.28}$ | $34.83_{\pm 3.16}$ | $39.43_{\pm 2.90}$ | $36.07_{\pm 3.02}$ |
| | BiomedCoOp | $37.92_{\pm 1.65}$ | $39.28_{\pm 3.59}$ | $36.79_{\pm 3.57}$ | $41.74_{\pm 3.90}$ | $42.28_{\pm 1.72}$ | $43.12_{\pm 1.78}$ | $42.75_{\pm 1.80}$ |
| | vMFCoOp (Ours) | $43.29_{\pm 1.78}$ | $43.12_{\pm 3.57}$ | $45.76_{\pm 3.60}$ | $47.34_{\pm 1.08}$ | $47.92_{\pm 1.75}$ | $49.80_{\pm 1.90}$ | $50.61_{\pm 0.25}$ |
| | MedCLIP | $37.06_{\pm 0.00}$ | $37.06_{\pm 0.00}$ | $37.06_{\pm 0.00}$ | $37.06_{\pm 0.00}$ | $37.06_{\pm 0.00}$ | $37.06_{\pm 0.00}$ | $37.06_{\pm 0.00}$ |
| | MedCLIP + Ensemble | $52.58_{\pm 0.00}$ | $52.58_{\pm 0.00}$ | $52.58_{\pm 0.00}$ | $52.58_{\pm 0.00}$ | $52.58_{\pm 0.00}$ | $52.58_{\pm 0.00}$ | $52.58_{\pm 0.00}$ |
| | CLIP-Adapter | $41.50_{\pm 5.81}$ | $47.37_{\pm 2.47}$ | $48.79_{\pm 1.69}$ | $46.83_{\pm 3.71}$ | $51.94_{\pm 3.66}$ | $53.82_{\pm 3.72}$ | $55.81_{\pm 3.93}$ |
| | Tip-Adapter | $27.50_{\pm 3.78}$ | $31.08_{\pm 6.23}$ | $38.05_{\pm 5.04}$ | $50.14_{\pm 3.31}$ | $46.30_{\pm 4.03}$ | $46.69_{\pm 4.12}$ | $44.43_{\pm 4.34}$ |
| | Tip-Adapter-F | $42.89_{\pm 2.79}$ | $51.18_{\pm 1.79}$ | $48.56_{\pm 4.85}$ | $56.47_{\pm 6.45}$ | $60.05_{\pm 1.47}$ | $60.70_{\pm 1.59}$ | $60.33_{\pm 1.68}$ |
| | Standard LP | $44.75_{\pm 12.21}$ | $49.73_{\pm 8.44}$ | $54.72_{\pm 7.08}$ | $56.28_{\pm 9.11}$ | $59.03_{\pm 3.78}$ | $61.50_{\pm 3.89}$ | $60.35_{\pm 3.95}$ |
| OCTMNIST | LP++ | $47.02_{\pm 13.22}$ | $54.58_{\pm 9.11}$ | $57.43_{\pm 8.49}$ | $57.79_{\pm 8.15}$ | $61.97_{\pm 7.32}$ | $64.27_{\pm 7.28}$ | $63.43_{\pm 7.14}$ |
| | CoOp | $49.68_{\pm 2.98}$ | $48.55_{\pm 3.90}$ | $46.87_{\pm 2.39}$ | $57.04_{\pm 4.50}$ | $61.54_{\pm 7.50}$ | $65.26_{\pm 7.21}$ | $65.07_{\pm 7.52}$ |
| | CoCoOp | $49.71_{\pm 4.45}$ | $49.28_{\pm 7.95}$ | $46.08_{\pm 6.30}$ | $52.46_{\pm 2.00}$ | $56.04_{\pm 3.50}$ | $56.97_{\pm 3.60}$ | $60.04_{\pm 3.72}$ |
| | KgCoOp | $52.44_{\pm 3.25}$ | $53.09_{\pm 5.32}$ | $54.28_{\pm 1.60}$ | $58.35_{\pm 3.73}$ | $59.85_{\pm 3.95}$ | $69.78_{\pm 4.05}$ | $70.81_{\pm 4.25}$ |
| | ProGrad | $56.69_{\pm 3.12}$ | $58.23_{\pm 3.45}$ | $58.70_{\pm 1.30}$ | $64.87_{\pm 6.15}$ | $66.08_{\pm 6.27}$ | $70.00_{\pm 6.35}$ | $66.32_{\pm 6.45}$ |
| | BiomedCoOp | $50.76_{\pm 1.58}$ | $53.66_{\pm 4.80}$ | $53.16_{\pm 1.88}$ | $60.56_{\pm 5.45}$ | $67.13_{\pm 2.25}$ | $68.04_{\pm 2.30}$ | $68.18_{\pm 2.42}$ |
| | vMFCoOp (Ours) | $54.77_{\pm 1.65}$ | $57.10_{\pm 4.90}$ | $61.21_{\pm 1.95}$ | $64.83_{\pm 5.50}$ | $71.87_{\pm 2.25}$ | $74.30_{\pm 2.35}$ | $75.26_{\pm 0.47}$ |
| | MedCLIP | $48.46_{\pm 0.00}$ | $48.46_{\pm 0.00}$ | $48.46_{\pm 0.00}$ | $48.46_{\pm 0.00}$ | $48.46_{\pm 0.00}$ | $48.46_{\pm 0.00}$ | $48.46_{\pm 0.00}$ |
| | MedCLIP + Ensemble | $49.15_{\pm 0.00}$ | $49.15_{\pm 0.00}$ | $49.15_{\pm 0.00}$ | $49.15_{\pm 0.00}$ | $49.15_{\pm 0.00}$ | $49.15_{\pm 0.00}$ | $49.15_{\pm 0.00}$ |
| | CLIP-Adapter | $38.50_{\pm 3.94}$ | $38.56_{\pm 3.98}$ | $40.50_{\pm 3.87}$ | $39.71_{\pm 1.06}$ | $41.77_{\pm 3.97}$ | $42.80_{\pm 3.88}$ | $44.31_{\pm 3.95}$ |
| | Tip-Adapter | $44.40_{\pm 2.43}$ | $45.58_{\pm 3.56}$ | $54.24_{\pm 3.75}$ | $55.38_{\pm 2.21}$ | $57.70_{\pm 1.37}$ | $58.00_{\pm 1.45}$ | $54.93_{\pm 1.46}$ |
| | Tip-Adapter-F | $41.89_{\pm 4.63}$ | $45.57_{\pm 5.11}$ | $50.29_{\pm 3.37}$ | $54.38_{\pm 2.58}$ | $57.04_{\pm 1.43}$ | $57.60_{\pm 1.52}$ | $56.65_{\pm 1.53}$ |
| | Standard LP | $40.12_{\pm 5.74}$ | $44.73_{\pm 6.31}$ | $50.72_{\pm 5.27}$ | $57.16_{\pm 4.45}$ | $61.78_{\pm 2.62}$ | $64.72_{\pm 2.78}$ | $62.51_{\pm 2.79}$ |
| UKB CardiacMRI | LP++ | $38.01_{\pm 3.51}$ | $48.39_{\pm 4.05}$ | $53.41_{\pm 4.15}$ | $59.41_{\pm 3.22}$ | $62.81_{\pm 2.14}$ | $65.42_{\pm 2.23}$ | $64.23_{\pm 2.34}$ |
| | CoOp | $34.82_{\pm 5.17}$ | $40.33_{\pm 2.48}$ | $46.25_{\pm 3.58}$ | $56.24_{\pm 2.61}$ | $64.68_{\pm 1.53}$ | $67.25_{\pm 1.64}$ | $65.82_{\pm 1.74}$ |
| | CoCoOp | $36.99_{\pm 2.78}$ | $42.20_{\pm 3.95}$ | $47.60_{\pm 5.04}$ | $56.24_{\pm 2.95}$ | $62.47_{\pm 1.23}$ | $62.50_{\pm 2.14}$ | $64.85_{\pm 2.35}$ |
| | KgCoOp | $46.66_{\pm 2.74}$ | $51.11_{\pm 2.82}$ | $56.48_{\pm 3.94}$ | $61.35_{\pm 4.10}$ | $64.25_{\pm 3.91}$ | $74.43_{\pm 3.94}$ | $75.73_{\pm 1.10}$ |
| | ProGrad | $49.29_{\pm 4.67}$ | $51.93_{\pm 3.34}$ | $61.70_{\pm 2.53}$ | $68.97_{\pm 1.97}$ | $71.28_{\pm 1.14}$ | $75.18_{\pm 1.26}$ | $71.07_{\pm 1.47}$ |
| | BiomedCoOp | $44.56_{\pm 2.24}$ | $47.56_{\pm 3.66}$ | $55.20_{\pm 1.92}$ | $66.06_{\pm 1.48}$ | $69.03_{\pm 1.20}$ | $69.09_{\pm 1.22}$ | $68.88_{\pm 1.21}$ |
| | vMFCoOp (Ours) | $54.34_{\pm 2.43}$ | $57.34_{\pm 3.96}$ | $69.00_{\pm 2.03}$ | $75.71_{\pm 1.64}$ | $75.38_{\pm 1.23}$ | $77.85_{\pm 1.27}$ | $80.08_{\pm 1.48}$ |

Table A3: (7-12) Comparative classification accuracy (%) of vMFCoOp and competing methods across 14 benchmark datasets in the few-shot scenario. This table presents results for datasets 7–12. All experiments are conducted under the configuration with `Qwen-2.5` and `MedCLIP`.

| **Dataset** | **Method** | $K = 1$ | $K = 2$ | $K = 4$ | $K = 8$ | $K = 16$ | $K = 32$ | $K = 64$ |
|---|---|---|---|---|---|---|---|---|
| UKB LiverMRI | MedCLIP | 53.07$_{\pm0.00}$ | 53.07$_{\pm0.00}$ | 53.07$_{\pm0.00}$ | 53.07$_{\pm0.00}$ | 53.07$_{\pm0.00}$ | 53.07$_{\pm0.00}$ | 53.07$_{\pm0.00}$ |
| | MedCLIP + Ensemble | 52.97$_{\pm0.00}$ | 52.97$_{\pm0.00}$ | 52.97$_{\pm0.00}$ | 52.97$_{\pm0.00}$ | 52.97$_{\pm0.00}$ | 52.97$_{\pm0.00}$ | 52.97$_{\pm0.00}$ |
| | CLIP-Adapter | 44.39$_{\pm1.24}$ | 43.90$_{\pm1.30}$ | 46.35$_{\pm1.15}$ | 44.83$_{\pm1.28}$ | 45.80$_{\pm1.32}$ | 47.35$_{\pm1.25}$ | 49.41$_{\pm1.30}$ |
| | Tip-Adapter | 47.90$_{\pm3.17}$ | 49.13$_{\pm4.56}$ | 57.55$_{\pm2.66}$ | 58.99$_{\pm1.95}$ | 60.73$_{\pm1.32}$ | 60.98$_{\pm1.41}$ | 58.23$_{\pm1.55}$ |
| | Tip-Adapter-F | 45.59$_{\pm2.56}$ | 47.81$_{\pm2.95}$ | 53.09$_{\pm3.12}$ | 56.91$_{\pm2.85}$ | 59.75$_{\pm1.72}$ | 60.26$_{\pm1.68}$ | 59.39$_{\pm1.84}$ |
| | Standard LP | 45.40$_{\pm5.02}$ | 49.24$_{\pm6.15}$ | 55.39$_{\pm4.55}$ | 58.54$_{\pm3.95}$ | 64.28$_{\pm2.13}$ | 66.87$_{\pm2.28}$ | 65.01$_{\pm2.37}$ |
| | LP++ | 43.49$_{\pm3.44}$ | 53.07$_{\pm3.05}$ | 58.08$_{\pm4.22}$ | 61.02$_{\pm3.17}$ | 65.29$_{\pm1.52}$ | 67.37$_{\pm1.62}$ | 66.01$_{\pm1.74}$ |
| | CoOp | 43.24$_{\pm2.50}$ | 44.83$_{\pm2.28}$ | 49.71$_{\pm3.35}$ | 57.54$_{\pm2.15}$ | 68.24$_{\pm1.51}$ | 70.83$_{\pm1.68}$ | 69.32$_{\pm1.80}$ |
| | CoCoOp | 45.31$_{\pm4.05}$ | 45.06$_{\pm3.20}$ | 54.08$_{\pm2.95}$ | 60.97$_{\pm1.85}$ | 65.86$_{\pm3.98}$ | 66.12$_{\pm1.08}$ | 68.78$_{\pm1.18}$ |
| | KgCoOp | 50.49$_{\pm1.70}$ | 50.39$_{\pm1.58}$ | 50.82$_{\pm1.45}$ | 54.85$_{\pm2.75}$ | 56.31$_{\pm1.38}$ | 66.51$_{\pm1.45}$ | 67.85$_{\pm1.51}$ |
| | ProGrad | 50.96$_{\pm4.35}$ | 54.58$_{\pm3.08}$ | 64.22$_{\pm2.68}$ | 71.10$_{\pm1.98}$ | 74.70$_{\pm1.14}$ | 78.84$_{\pm1.24}$ | 74.57$_{\pm1.47}$ |
| | BiomedCoOp | 50.52$_{\pm2.34}$ | 53.06$_{\pm3.72}$ | 57.29$_{\pm1.95}$ | 66.46$_{\pm1.48}$ | 72.43$_{\pm1.20}$ | 71.86$_{\pm1.22}$ | 72.22$_{\pm1.28}$ |
| | vMFCoOp (Ours) | 57.14$_{\pm2.99}$ | 59.44$_{\pm3.49}$ | 68.89$_{\pm2.28}$ | 73.44$_{\pm1.14}$ | 77.82$_{\pm1.11}$ | 81.42$_{\pm1.15}$ | 83.43$_{\pm1.10}$ |
| UKB PancreasMRI | MedCLIP | 42.36$_{\pm0.00}$ | 42.36$_{\pm0.00}$ | 42.36$_{\pm0.00}$ | 42.36$_{\pm0.00}$ | 42.36$_{\pm0.00}$ | 42.36$_{\pm0.00}$ | 42.36$_{\pm0.00}$ |
| | MedCLIP + Ensemble | 43.65$_{\pm0.00}$ | 43.65$_{\pm0.00}$ | 43.65$_{\pm0.00}$ | 43.65$_{\pm0.00}$ | 43.65$_{\pm0.00}$ | 43.65$_{\pm0.00}$ | 43.65$_{\pm0.00}$ |
| | CLIP-Adapter | 32.94$_{\pm3.45}$ | 32.61$_{\pm4.05}$ | 35.40$_{\pm3.65}$ | 33.80$_{\pm3.25}$ | 34.89$_{\pm2.95}$ | 36.40$_{\pm2.85}$ | 38.18$_{\pm2.87}$ |
| | Tip-Adapter | 38.00$_{\pm6.34}$ | 41.53$_{\pm7.22}$ | 48.17$_{\pm6.11}$ | 49.03$_{\pm5.05}$ | 49.12$_{\pm4.33}$ | 51.00$_{\pm3.32}$ | 50.38$_{\pm2.56}$ |
| | Tip-Adapter-F | 37.91$_{\pm7.45}$ | 42.66$_{\pm8.10}$ | 43.34$_{\pm7.92}$ | 45.39$_{\pm6.05}$ | 43.72$_{\pm5.47}$ | 46.86$_{\pm4.15}$ | 48.49$_{\pm3.67}$ |
| | Standard LP | 38.29$_{\pm8.21}$ | 41.22$_{\pm9.12}$ | 44.81$_{\pm8.45}$ | 45.56$_{\pm7.28}$ | 47.03$_{\pm6.55}$ | 52.18$_{\pm5.22}$ | 51.83$_{\pm4.37}$ |
| | LP++ | 37.13$_{\pm7.11}$ | 47.96$_{\pm8.38}$ | 53.01$_{\pm7.11}$ | 52.56$_{\pm6.41}$ | 53.91$_{\pm5.06}$ | 58.04$_{\pm4.20}$ | 58.69$_{\pm3.28}$ |
| | CoOp | 33.59$_{\pm6.90}$ | 39.95$_{\pm7.40}$ | 46.50$_{\pm6.05}$ | 49.69$_{\pm5.05}$ | 54.31$_{\pm4.33}$ | 59.73$_{\pm3.15}$ | 60.29$_{\pm2.90}$ |
| | CoCoOp | 39.14$_{\pm7.02}$ | 42.61$_{\pm8.12}$ | 50.58$_{\pm7.15}$ | 53.76$_{\pm6.45}$ | 54.72$_{\pm5.28}$ | 57.65$_{\pm4.35}$ | 62.10$_{\pm3.72}$ |
| | KgCoOp | 42.94$_{\pm3.42}$ | 44.77$_{\pm4.15}$ | 47.73$_{\pm3.60}$ | 52.55$_{\pm4.05}$ | 54.00$_{\pm3.12}$ | 65.38$_{\pm2.48}$ | 68.23$_{\pm2.15}$ |
| | ProGrad | 45.02$_{\pm5.95}$ | 48.73$_{\pm6.98}$ | 56.15$_{\pm5.53}$ | 58.72$_{\pm4.56}$ | 60.48$_{\pm3.40}$ | 66.93$_{\pm2.21}$ | 65.52$_{\pm2.05}$ |
| | BiomedCoOp | 42.46$_{\pm2.65}$ | 48.26$_{\pm3.90}$ | 54.81$_{\pm2.10}$ | 63.96$_{\pm1.50}$ | 64.65$_{\pm1.30}$ | 64.59$_{\pm1.45}$ | 65.23$_{\pm1.52}$ |
| | vMFCoOp (Ours) | 50.42$_{\pm2.10}$ | 54.70$_{\pm1.80}$ | 66.81$_{\pm1.50}$ | 71.38$_{\pm1.32}$ | 71.97$_{\pm1.25}$ | 73.70$_{\pm1.28}$ | 73.26$_{\pm1.30}$ |
| Average | MedCLIP | 50.12$_{\pm0.00}$ | 50.12$_{\pm0.00}$ | 50.12$_{\pm0.00}$ | 50.12$_{\pm0.00}$ | 50.12$_{\pm0.00}$ | 50.12$_{\pm0.00}$ | 50.12$_{\pm0.00}$ |
| | MedCLIP + Ensemble | 56.37$_{\pm0.00}$ | 56.37$_{\pm0.00}$ | 56.37$_{\pm0.00}$ | 56.37$_{\pm0.00}$ | 56.37$_{\pm0.00}$ | 56.37$_{\pm0.00}$ | 56.37$_{\pm0.00}$ |
| | CLIP-Adapter | 42.13$_{\pm1.53}$ | 41.58$_{\pm2.81}$ | 43.98$_{\pm2.47}$ | 43.05$_{\pm3.52}$ | 45.12$_{\pm2.79}$ | 46.25$_{\pm1.82}$ | 47.98$_{\pm1.67}$ |
| | Tip-Adapter | 45.23$_{\pm5.12}$ | 49.45$_{\pm6.14}$ | 57.04$_{\pm5.23}$ | 58.13$_{\pm6.08}$ | 60.67$_{\pm3.14}$ | 60.58$_{\pm4.12}$ | 58.22$_{\pm4.05}$ |
| | Tip-Adapter-F | 47.11$_{\pm7.98}$ | 49.87$_{\pm5.23}$ | 54.45$_{\pm3.98}$ | 57.22$_{\pm2.76}$ | 58.39$_{\pm5.11}$ | 59.76$_{\pm4.02}$ | 58.88$_{\pm1.07}$ |
| | Standard LP | 46.37$_{\pm6.12}$ | 49.97$_{\pm6.05}$ | 55.21$_{\pm3.89}$ | 57.45$_{\pm7.89}$ | 60.33$_{\pm4.52}$ | 63.15$_{\pm3.98}$ | 61.47$_{\pm2.53}$ |
| | LP++ | 47.22$_{\pm7.52}$ | 54.87$_{\pm5.43}$ | 58.13$_{\pm3.47}$ | 59.44$_{\pm5.45}$ | 63.26$_{\pm2.98}$ | 65.38$_{\pm2.98}$ | 64.59$_{\pm2.98}$ |
| | CoOp | 45.28$_{\pm5.12}$ | 47.93$_{\pm3.98}$ | 52.11$_{\pm2.93}$ | 58.34$_{\pm2.12}$ | 65.22$_{\pm2.08}$ | 68.14$_{\pm1.53}$ | 67.28$_{\pm3.47}$ |
| | CoCoOp | 48.12$_{\pm3.98}$ | 49.14$_{\pm3.97}$ | 52.98$_{\pm4.87}$ | 59.07$_{\pm3.98}$ | 62.34$_{\pm2.98}$ | 62.87$_{\pm6.97}$ | 65.89$_{\pm3.98}$ |
| | KgCoOp | 53.37$_{\pm2.98}$ | 55.22$_{\pm2.99}$ | 59.21$_{\pm3.98}$ | 61.11$_{\pm5.49}$ | 62.47$_{\pm6.37}$ | 72.52$_{\pm2.98}$ | 73.88$_{\pm1.97}$ |
| | ProGrad | 56.18$_{\pm4.57}$ | 57.34$_{\pm3.98}$ | 64.43$_{\pm3.57}$ | 69.22$_{\pm3.98}$ | 71.28$_{\pm4.43}$ | 75.49$_{\pm1.48}$ | 71.97$_{\pm3.98}$ |
| | BiomedCoOp | 54.27$_{\pm5.98}$ | 56.17$_{\pm4.43}$ | 61.22$_{\pm3.47}$ | 69.11$_{\pm2.47}$ | 72.14$_{\pm1.52}$ | 71.98$_{\pm3.43}$ | 71.92$_{\pm3.98}$ |
| | vMFCoOp (Ours) | 59.32$_{\pm2.98}$ | 60.54$_{\pm2.53}$ | 70.12$_{\pm1.47}$ | 74.38$_{\pm1.18}$ | 77.11$_{\pm0.98}$ | 79.24$_{\pm0.98}$ | 80.17$_{\pm0.77}$ |

Table A3: (13–14) Comparative classification accuracy (%) of vMFCoOp and competing methods on the final two of 14 benchmark datasets under the few-shot setting. All experiments in this Table S2 follow the Best Performance configuration using `Qwen-2.5` and `MedCLIP`.

| Dataset | Method | $K=1$ | $K=2$ | $K=4$ | $K=8$ | $K=16$ | $K=32$ | $K=64$ |
|---|---|---|---|---|---|---|---|---|
| | Biomedical CLIPs | 61.22 | | | | | | |
| | Biomedical CLIPs + Ensemble | 65.14 | | | | | | |
| | CLIP-Adapter | $52.93_{\pm 1.64}$ | $54.50_{\pm 3.24}$ | $55.47_{\pm 2.87}$ | $54.49_{\pm 4.45}$ | $57.73_{\pm 3.83}$ | $58.45_{\pm 3.37}$ | $60.91_{\pm 2.96}$ |
| | Tip-Adapter | $61.78_{\pm 4.11}$ | $64.53_{\pm 2.60}$ | $74.76_{\pm 2.09}$ | $69.70_{\pm 3.71}$ | $74.53_{\pm 1.16}$ | $75.97_{\pm 1.30}$ | $76.07_{\pm 1.68}$ |
| | Tip-Adapter-F | $56.10_{\pm 4.29}$ | $59.85_{\pm 4.68}$ | $73.19_{\pm -0.47}$ | $70.99_{\pm 1.37}$ | $72.42_{\pm 4.03}$ | $75.79_{\pm 3.46}$ | $75.80_{\pm 0.91}$ |
| | Standard LP | $61.20_{\pm 3.22}$ | $69.20_{\pm 4.06}$ | $71.27_{\pm 0.48}$ | $68.67_{\pm 6.06}$ | $74.41_{\pm 3.89}$ | $80.15_{\pm 2.88}$ | $79.86_{\pm 2.62}$ |
| BTMRI | LP++ | $68.16_{\pm 6.05}$ | $78.35_{\pm 4.80}$ | $78.88_{\pm -1.36}$ | $77.06_{\pm 2.23}$ | $82.80_{\pm 1.48}$ | $85.00_{\pm 1.09}$ | $86.24_{\pm 1.89}$ |
| | CoOp | $60.10_{\pm 2.86}$ | $62.28_{\pm 4.47}$ | $66.57_{\pm 1.02}$ | $71.45_{\pm -0.11}$ | $78.01_{\pm 0.88}$ | $83.03_{\pm 0.60}$ | $80.41_{\pm 3.21}$ |
| | CoCoOp | $59.27_{\pm 2.80}$ | $62.17_{\pm 2.30}$ | $65.36_{\pm 4.85}$ | $68.33_{\pm 4.87}$ | $74.93_{\pm 1.37}$ | $76.27_{\pm 5.12}$ | $79.09_{\pm 3.28}$ |
| | KgCoOp | $61.73_{\pm 3.63}$ | $68.69_{\pm 5.11}$ | $73.50_{\pm 2.93}$ | $73.47_{\pm 4.49}$ | $74.68_{\pm 7.90}$ | $85.27_{\pm 4.65}$ | $84.00_{\pm 3.75}$ |
| | ProGrad | $72.80_{\pm 1.92}$ | $73.79_{\pm 3.31}$ | $79.48_{\pm 5.24}$ | $82.35_{\pm 3.06}$ | $85.91_{\pm 3.47}$ | $88.45_{\pm 0.39}$ | $87.91_{\pm 2.87}$ |
| | BiomedCoOp | $65.15_{\pm 4.67}$ | $71.10_{\pm 4.87}$ | $78.14_{\pm 4.77}$ | $79.54_{\pm 1.80}$ | $81.90_{\pm 0.96}$ | $83.02_{\pm 2.46}$ | $82.12_{\pm 3.56}$ |
| | vMFCoOp (Ours) | $64.67_{\pm 3.85}$ | $69.29_{\pm 4.72}$ | $80.22_{\pm 3.53}$ | $80.96_{\pm 1.48}$ | $84.98_{\pm 0.76}$ | $85.82_{\pm 0.71}$ | $86.29_{\pm 1.23}$ |
| | Biomedical CLIPs | 65.18 | | | | | | |
| | Biomedical CLIPs + Ensemble | 64.09 | | | | | | |
| | CLIP-Adapter | $58.66_{\pm 1.67}$ | $58.94_{\pm 3.42}$ | $61.07_{\pm 3.21}$ | $59.70_{\pm 1.98}$ | $61.20_{\pm 2.34}$ | $62.44_{\pm 1.68}$ | $65.37_{\pm 1.30}$ |
| | Tip-Adapter | $58.57_{\pm 3.12}$ | $59.71_{\pm 2.37}$ | $58.90_{\pm 1.81}$ | $53.08_{\pm 10.79}$ | $65.80_{\pm 5.15}$ | $67.19_{\pm 5.33}$ | $67.07_{\pm 5.67}$ |
| | Tip-Adapter-F | $59.22_{\pm 4.12}$ | $55.55_{\pm 5.87}$ | $62.12_{\pm 4.52}$ | $61.87_{\pm 1.85}$ | $63.36_{\pm 3.31}$ | $68.66_{\pm 2.48}$ | $68.63_{\pm -0.28}$ |
| | Standard LP | $50.79_{\pm 9.54}$ | $45.34_{\pm 5.00}$ | $49.88_{\pm 5.31}$ | $57.76_{\pm 9.19}$ | $62.48_{\pm 3.19}$ | $68.94_{\pm 2.08}$ | $68.43_{\pm 1.68}$ |
| BUSI | LP++ | $54.86_{\pm 5.79}$ | $63.15_{\pm 1.77}$ | $64.85_{\pm 0.47}$ | $67.15_{\pm 3.20}$ | $71.83_{\pm 1.77}$ | $75.23_{\pm 1.35}$ | $76.47_{\pm 1.99}$ |
| | CoOp | $45.81_{\pm 2.44}$ | $48.09_{\pm 2.40}$ | $53.34_{\pm 2.06}$ | $57.37_{\pm 3.92}$ | $65.93_{\pm 2.26}$ | $71.44_{\pm 2.28}$ | $68.78_{\pm 4.88}$ |
| | CoCoOp | $52.93_{\pm 2.59}$ | $48.37_{\pm 1.31}$ | $58.64_{\pm 2.32}$ | $64.00_{\pm 4.13}$ | $68.46_{\pm 0.98}$ | $69.94_{\pm 4.73}$ | $72.53_{\pm 2.71}$ |
| | KgCoOp | $52.96_{\pm 7.14}$ | $55.04_{\pm 2.94}$ | $61.02_{\pm 4.84}$ | $62.59_{\pm 5.68}$ | $64.88_{\pm 6.60}$ | $75.93_{\pm 3.53}$ | $74.33_{\pm 2.63}$ |
| | ProGrad | $52.64_{\pm 3.99}$ | $52.73_{\pm 7.47}$ | $66.71_{\pm 7.49}$ | $68.76_{\pm 5.53}$ | $75.12_{\pm 5.03}$ | $77.76_{\pm 1.81}$ | $77.43_{\pm 4.30}$ |
| | BiomedCoOp | $51.27_{\pm 4.63}$ | $51.87_{\pm 8.01}$ | $61.20_{\pm 2.29}$ | $65.66_{\pm 4.27}$ | $69.97_{\pm 2.01}$ | $71.84_{\pm 3.42}$ | $71.13_{\pm 4.53}$ |
| | vMFCoOp (Ours) | $52.11_{\pm 3.86}$ | $51.13_{\pm 7.76}$ | $63.36_{\pm 0.88}$ | $66.64_{\pm 3.94}$ | $73.99_{\pm 1.70}$ | $74.59_{\pm 1.66}$ | $75.04_{\pm 2.12}$ |
| | Biomedical CLIPs | 47.93 | | | | | | |
| | Biomedical CLIPs + Ensemble | 71.79 | | | | | | |
| | CLIP-Adapter | $46.54_{\pm -0.68}$ | $40.25_{\pm 0.60}$ | $44.67_{\pm 2.59}$ | $45.39_{\pm 1.75}$ | $46.63_{\pm 1.56}$ | $48.83_{\pm 0.85}$ | $51.53_{\pm 0.51}$ |
| | Tip-Adapter | $57.29_{\pm 8.41}$ | $56.04_{\pm 4.91}$ | $62.70_{\pm 10.59}$ | $63.03_{\pm 5.86}$ | $70.48_{\pm 1.02}$ | $70.19_{\pm 1.70}$ | $70.18_{\pm 2.28}$ |
| | Tip-Adapter-F | $51.45_{\pm 18.89}$ | $52.30_{\pm 6.58}$ | $66.04_{\pm 2.00}$ | $62.15_{\pm 3.59}$ | $68.59_{\pm 5.10}$ | $71.28_{\pm 4.46}$ | $71.45_{\pm 1.88}$ |
| | Standard LP | $48.59_{\pm 9.54}$ | $44.80_{\pm 14.86}$ | $55.43_{\pm 10.86}$ | $59.79_{\pm 8.83}$ | $66.24_{\pm 3.33}$ | $71.10_{\pm 2.37}$ | $70.76_{\pm 2.05}$ |
| COVID-QU-Ex | LP++ | $49.30_{\pm 11.08}$ | $62.98_{\pm 13.96}$ | $65.64_{\pm 6.50}$ | $66.02_{\pm 9.19}$ | $73.66_{\pm 1.26}$ | $76.11_{\pm 1.01}$ | $77.14_{\pm 1.71}$ |
| | CoOp | $55.09_{\pm 13.34}$ | $52.19_{\pm 7.38}$ | $59.23_{\pm 4.87}$ | $66.94_{\pm 1.30}$ | $73.15_{\pm 0.61}$ | $77.57_{\pm 0.72}$ | $75.03_{\pm 3.50}$ |
| | CoCoOp | $69.16_{\pm 1.59}$ | $66.98_{\pm 1.19}$ | $61.32_{\pm 10.21}$ | $66.72_{\pm 3.70}$ | $71.93_{\pm 3.56}$ | $72.94_{\pm 7.43}$ | $75.33_{\pm 2.54}$ |
| | KgCoOp | $60.33_{\pm 9.26}$ | $53.16_{\pm 11.72}$ | $63.49_{\pm 8.93}$ | $70.22_{\pm 6.81}$ | $70.09_{\pm 8.55}$ | $80.61_{\pm 2.30}$ | $79.09_{\pm 1.50}$ |
| | ProGrad | $66.02_{\pm 11.21}$ | $66.98_{\pm 6.40}$ | $71.81_{\pm 3.36}$ | $78.46_{\pm 2.66}$ | $78.56_{\pm 3.64}$ | $80.61_{\pm 0.62}$ | $79.95_{\pm 3.03}$ |
| | BiomedCoOp | $72.18_{\pm 5.29}$ | $71.58_{\pm 2.31}$ | $74.33_{\pm 3.21}$ | $78.81_{\pm 3.20}$ | $78.50_{\pm 3.04}$ | $79.24_{\pm 4.79}$ | $78.23_{\pm 5.97}$ |
| | vMFCoOp (Ours) | $71.94_{\pm 4.49}$ | $70.01_{\pm 2.29}$ | $76.06_{\pm 2.03}$ | $79.37_{\pm 2.93}$ | $81.06_{\pm 2.92}$ | $81.76_{\pm 3.04}$ | $81.98_{\pm 0.60}$ |
| | Biomedical CLIPs | 47.18 | | | | | | |
| | Biomedical CLIPs + Ensemble | 61.25 | | | | | | |
| | CLIP-Adapter | $42.23_{\pm 1.56}$ | $36.49_{\pm 1.36}$ | $39.69_{\pm 1.40}$ | $40.53_{\pm 4.30}$ | $43.21_{\pm 1.51}$ | $44.56_{\pm 1.31}$ | $47.02_{\pm 1.01}$ |
| | Tip-Adapter | $38.58_{\pm 5.29}$ | $46.76_{\pm 7.05}$ | $52.40_{\pm 4.45}$ | $63.98_{\pm 8.81}$ | $71.18_{\pm 7.50}$ | $69.16_{\pm 7.40}$ | $67.98_{\pm 7.43}$ |
| | Tip-Adapter-F | $44.09_{\pm 8.55}$ | $55.76_{\pm 6.97}$ | $56.36_{\pm 7.66}$ | $68.78_{\pm 6.03}$ | $72.55_{\pm 5.10}$ | $78.53_{\pm 4.55}$ | $75.80_{\pm 1.88}$ |
| | Standard LP | $40.97_{\pm 4.22}$ | $55.14_{\pm 4.91}$ | $64.33_{\pm 5.03}$ | $68.50_{\pm 10.11}$ | $76.51_{\pm 6.75}$ | $79.33_{\pm 5.22}$ | $79.34_{\pm 4.88}$ |
| CTKIDNEY | LP++ | $58.35_{\pm 3.44}$ | $69.09_{\pm 2.91}$ | $67.98_{\pm 5.46}$ | $75.56_{\pm 8.63}$ | $80.77_{\pm 7.20}$ | $79.91_{\pm 6.39}$ | $80.24_{\pm 6.70}$ |
| | CoOp | $48.71_{\pm 7.54}$ | $55.09_{\pm 1.98}$ | $58.47_{\pm 1.05}$ | $67.39_{\pm 1.69}$ | $78.06_{\pm 1.07}$ | $80.93_{\pm 0.53}$ | $79.89_{\pm 2.90}$ |
| | CoCoOp | $46.22_{\pm 5.94}$ | $49.53_{\pm 7.99}$ | $58.48_{\pm 1.76}$ | $70.38_{\pm 2.10}$ | $74.43_{\pm 2.46}$ | $74.79_{\pm 5.90}$ | $78.14_{\pm 3.98}$ |
| | KgCoOp | $57.79_{\pm 1.24}$ | $60.00_{\pm 3.02}$ | $65.52_{\pm 6.02}$ | $72.99_{\pm 7.61}$ | $69.71_{\pm 7.20}$ | $80.39_{\pm 4.00}$ | $79.16_{\pm 2.90}$ |
| | ProGrad | $57.68_{\pm 8.07}$ | $65.11_{\pm 5.31}$ | $70.39_{\pm 2.16}$ | $82.43_{\pm 5.53}$ | $85.62_{\pm 4.86}$ | $83.97_{\pm 2.19}$ | $83.20_{\pm 4.05}$ |
| | BiomedCoOp | $55.33_{\pm 7.29}$ | $63.67_{\pm 6.16}$ | $67.82_{\pm 3.05}$ | $79.08_{\pm 3.70}$ | $81.83_{\pm 2.06}$ | $81.78_{\pm 3.54}$ | $80.81_{\pm 4.65}$ |
| | vMFCoOp (Ours) | $58.02_{\pm 6.60}$ | $64.76_{\pm 6.19}$ | $71.35_{\pm 1.94}$ | $81.40_{\pm 3.76}$ | $86.78_{\pm 2.13}$ | $88.76_{\pm 2.05}$ | $88.26_{\pm 0.50}$ |
| | Biomedical CLIPs | 43.39 | | | | | | |
| | Biomedical CLIPs + Ensemble | 58.70 | | | | | | |
| | CLIP-Adapter | $32.34_{\pm 3.99}$ | $33.48_{\pm 5.62}$ | $33.51_{\pm 3.00}$ | $31.62_{\pm 6.63}$ | $26.51_{\pm 3.41}$ | $27.54_{\pm 3.15}$ | $29.54_{\pm 3.09}$ |
| | Tip-Adapter | $35.28_{\pm 3.12}$ | $37.89_{\pm 12.35}$ | $45.78_{\pm 6.63}$ | $58.02_{\pm 5.87}$ | $60.85_{\pm 1.05}$ | $60.50_{\pm 1.73}$ | $60.51_{\pm 1.86}$ |
| | Tip-Adapter-F | $36.64_{\pm 17.13}$ | $36.88_{\pm 3.04}$ | $47.17_{\pm 2.68}$ | $35.80_{\pm 1.63}$ | $47.12_{\pm 6.44}$ | $50.26_{\pm 5.46}$ | $49.66_{\pm 2.52}$ |
| | Standard LP | $29.31_{\pm 11.79}$ | $35.21_{\pm 8.88}$ | $45.45_{\pm 6.24}$ | $44.75_{\pm 6.11}$ | $48.30_{\pm 4.61}$ | $53.91_{\pm 3.60}$ | $52.34_{\pm 2.95}$ |
| DermaMNIST | LP++ | $29.84_{\pm 4.20}$ | $35.22_{\pm 10.59}$ | $38.87_{\pm 6.09}$ | $45.36_{\pm 3.51}$ | $52.94_{\pm 2.12}$ | $54.63_{\pm 1.70}$ | $55.17_{\pm 2.28}$ |
| | CoOp | $22.42_{\pm 8.14}$ | $32.65_{\pm 5.27}$ | $38.21_{\pm 4.63}$ | $37.94_{\pm 3.98}$ | $47.02_{\pm 1.44}$ | $51.46_{\pm 1.33}$ | $47.99_{\pm 3.99}$ |
| | CoCoOp | $24.45_{\pm 3.17}$ | $23.18_{\pm 2.27}$ | $23.32_{\pm 5.75}$ | $38.01_{\pm 2.65}$ | $39.38_{\pm 5.98}$ | $39.89_{\pm 9.43}$ | $42.08_{\pm 7.13}$ |
| | KgCoOp | $25.90_{\pm 10.34}$ | $29.41_{\pm 4.08}$ | $33.34_{\pm 8.21}$ | $33.30_{\pm 7.96}$ | $32.39_{\pm 6.66}$ | $42.13_{\pm 3.36}$ | $40.23_{\pm 2.48}$ |
| | ProGrad | $39.43_{\pm 10.14}$ | $40.43_{\pm 6.54}$ | $47.51_{\pm 10.53}$ | $54.24_{\pm 3.57}$ | $49.62_{\pm 7.23}$ | $52.56_{\pm 4.11}$ | $51.63_{\pm 6.40}$ |
| | BiomedCoOp | $58.51_{\pm 7.22}$ | $57.46_{\pm 2.18}$ | $63.48_{\pm 3.09}$ | $63.56_{\pm 3.39}$ | $63.65_{\pm 0.98}$ | $64.44_{\pm 2.65}$ | $63.23_{\pm 3.73}$ |
| | vMFCoOp (Ours) | $57.80_{\pm 6.73}$ | $56.09_{\pm 2.05}$ | $63.78_{\pm 1.61}$ | $64.52_{\pm 3.16}$ | $65.21_{\pm 1.43}$ | $65.84_{\pm 1.27}$ | $65.98_{\pm 1.78}$ |
| | Biomedical CLIPs | 58.97 | | | | | | |
| | Biomedical CLIPs + Ensemble | 61.84 | | | | | | |
| | CLIP-Adapter | $49.70_{\pm 1.53}$ | $51.45_{\pm 3.28}$ | $51.41_{\pm 3.04}$ | $50.95_{\pm 4.46}$ | $52.22_{\pm 4.21}$ | $53.03_{\pm 0.77}$ | $55.72_{\pm 0.38}$ |
| | Tip-Adapter | $50.65_{\pm 2.94}$ | $57.81_{\pm 4.09}$ | $67.25_{\pm 2.37}$ | $64.22_{\pm 1.77}$ | $69.41_{\pm 1.18}$ | $69.72_{\pm 1.80}$ | $69.64_{\pm 2.10}$ |
| | Tip-Adapter-F | $57.09_{\pm 5.95}$ | $63.76_{\pm 2.22}$ | $67.20_{\pm 0.13}$ | $68.16_{\pm 3.48}$ | $71.46_{\pm 3.17}$ | $75.34_{\pm 2.57}$ | $75.50_{\pm -0.24}$ |
| | Standard LP | $52.88_{\pm 0.73}$ | $58.67_{\pm 2.60}$ | $68.15_{\pm 0.70}$ | $70.29_{\pm 6.71}$ | $72.28_{\pm 5.33}$ | $75.09_{\pm 4.16}$ | $74.73_{\pm 0.79}$ |
| Kvasir | LP++ | $60.16_{\pm 3.89}$ | $68.81_{\pm 2.67}$ | $72.97_{\pm 1.25}$ | $73.22_{\pm 3.67}$ | $75.74_{\pm 1.28}$ | $77.98_{\pm 0.87}$ | $78.95_{\pm 1.48}$ |
| | CoOp | $54.26_{\pm 0.98}$ | $60.90_{\pm 0.85}$ | $62.47_{\pm 2.07}$ | $69.19_{\pm -0.62}$ | $74.54_{\pm 0.31}$ | $77.81_{\pm 0.24}$ | $75.72_{\pm 2.83}$ |
| | CoCoOp | $59.11_{\pm 2.16}$ | $62.68_{\pm 1.93}$ | $66.37_{\pm 1.83}$ | $69.50_{\pm 2.12}$ | $73.11_{\pm 1.94}$ | $73.77_{\pm 5.60}$ | $76.04_{\pm 3.55}$ |
| | KgCoOp | $60.91_{\pm 2.27}$ | $66.36_{\pm 1.64}$ | $68.12_{\pm 4.01}$ | $66.76_{\pm 5.29}$ | $66.72_{\pm 5.94}$ | $77.49_{\pm 2.36}$ | $75.85_{\pm 1.52}$ |
| | ProGrad | $65.31_{\pm 3.18}$ | $66.66_{\pm 3.99}$ | $72.99_{\pm 3.59}$ | $78.42_{\pm 2.90}$ | $81.03_{\pm 6.32}$ | $81.98_{\pm 0.29}$ | $81.29_{\pm 2.73}$ |
| | BiomedCoOp | $64.21_{\pm 4.87}$ | $67.57_{\pm 3.51}$ | $75.60_{\pm 2.48}$ | $78.99_{\pm 3.24}$ | $77.90_{\pm 1.00}$ | $78.64_{\pm 2.44}$ | $78.11_{\pm 3.57}$ |
| | vMFCoOp (Ours) | $63.98_{\pm 4.09}$ | $67.75_{\pm 3.38}$ | $78.10_{\pm 0.93}$ | $80.17_{\pm 2.92}$ | $81.45_{\pm 0.81}$ | $81.01_{\pm 0.76}$ | $81.35_{\pm 1.34}$ |

Table A4: (1–6) Comparative classification accuracy (%) of vMFCoOp and competing methods on datasets 1–6 under the few-shot setting. Results are averaged over all 16 LLM–BiomedCLIP configurations (4 LLMs × 4 CLIPs).

| Dataset | Method | $K=1$ | $K=2$ | $K=4$ | $K=8$ | $K=16$ | $K=32$ | $K=64$ |
|---|---|---|---|---|---|---|---|---|
| CHMNIST | Biomedical CLIPs | | | | 40.71 | | | |
| | Biomedical CLIPs + Ensemble | | | | 39.63 | | | |
| | CLIP-Adapter | $33.21_{\pm 1.77}$ | $34.32_{\pm 3.44}$ | $37.04_{\pm 3.00}$ | $38.43_{\pm 1.90}$ | $44.28_{\pm 2.54}$ | $44.74_{\pm 1.80}$ | $46.89_{\pm 1.20}$ |
| | Tip-Adapter | $47.32_{\pm 10.10}$ | $64.81_{\pm 2.22}$ | $74.35_{\pm 1.66}$ | $71.23_{\pm 2.14}$ | $78.38_{\pm 1.15}$ | $78.51_{\pm 1.70}$ | $77.67_{\pm 1.97}$ |
| | Tip-Adapter-F | $54.92_{\pm 5.23}$ | $62.28_{\pm 3.70}$ | $73.25_{\pm 0.59}$ | $71.70_{\pm 1.71}$ | $76.51_{\pm 4.59}$ | $79.46_{\pm 3.40}$ | $79.03_{\pm 0.60}$ |
| | Standard LP | $62.98_{\pm 1.09}$ | $67.17_{\pm 2.33}$ | $72.95_{\pm 0.49}$ | $73.24_{\pm 6.09}$ | $78.13_{\pm 3.39}$ | $83.24_{\pm 2.25}$ | $82.23_{\pm 1.83}$ |
| | LP++ | $65.52_{\pm 6.91}$ | $72.28_{\pm 0.79}$ | $76.97_{\pm 3.82}$ | $77.25_{\pm 4.86}$ | $82.64_{\pm 1.75}$ | $84.73_{\pm 1.30}$ | $85.25_{\pm 1.84}$ |
| | CoOp | $59.34_{\pm 3.69}$ | $58.71_{\pm 0.82}$ | $65.61_{\pm 0.78}$ | $71.57_{\pm 1.82}$ | $79.93_{\pm 0.39}$ | $83.74_{\pm 0.18}$ | $80.83_{\pm 2.83}$ |
| | CoCoOp | $54.86_{\pm 3.46}$ | $55.20_{\pm 2.02}$ | $62.42_{\pm 2.64}$ | $69.60_{\pm 1.85}$ | $74.56_{\pm 3.43}$ | $75.69_{\pm 7.28}$ | $77.83_{\pm 5.36}$ |
| | KgCoOp | $62.96_{\pm 4.22}$ | $64.11_{\pm 1.12}$ | $72.04_{\pm 1.66}$ | $69.19_{\pm 6.58}$ | $72.67_{\pm 5.92}$ | $82.88_{\pm 2.23}$ | $81.03_{\pm 1.48}$ |
| | ProGrad | $70.71_{\pm 5.74}$ | $68.03_{\pm 1.92}$ | $77.91_{\pm 1.66}$ | $79.66_{\pm 4.93}$ | $83.12_{\pm 3.93}$ | $84.81_{\pm 0.96}$ | $83.93_{\pm 3.25}$ |
| | BiomedCoOp | $65.36_{\pm 5.56}$ | $65.68_{\pm 2.38}$ | $77.83_{\pm 2.89}$ | $81.81_{\pm 0.97}$ | $83.35_{\pm 1.88}$ | $83.39_{\pm 3.07}$ | $82.08_{\pm 4.23}$ |
| | vMFCoOp (Ours) | $64.92_{\pm 4.78}$ | $63.49_{\pm 2.20}$ | $79.26_{\pm 1.66}$ | $81.57_{\pm 0.61}$ | $85.21_{\pm 1.68}$ | $84.79_{\pm 1.17}$ | $84.63_{\pm 1.78}$ |
| LC25000 | Biomedical CLIPs | | | | 55.03 | | | |
| | Biomedical CLIPs + Ensemble | | | | 65.63 | | | |
| | CLIP-Adapter | $51.68_{\pm 1.27}$ | $51.52_{\pm 2.42}$ | $51.64_{\pm 1.04}$ | $54.00_{\pm 4.00}$ | $54.20_{\pm 1.34}$ | $55.17_{\pm 0.82}$ | $57.57_{\pm 0.43}$ |
| | Tip-Adapter | $70.85_{\pm 4.67}$ | $70.23_{\pm 7.07}$ | $82.33_{\pm 4.20}$ | $83.88_{\pm 2.24}$ | $85.50_{\pm 3.30}$ | $85.82_{\pm 3.88}$ | $85.72_{\pm 4.21}$ |
| | Tip-Adapter-F | $71.47_{\pm 6.11}$ | $70.25_{\pm 5.95}$ | $76.82_{\pm 7.83}$ | $82.85_{\pm 1.81}$ | $83.81_{\pm 3.04}$ | $87.62_{\pm 2.43}$ | $87.23_{\pm -0.30}$ |
| | Standard LP | $74.10_{\pm 1.54}$ | $75.78_{\pm 5.93}$ | $81.90_{\pm 1.44}$ | $81.84_{\pm 6.39}$ | $85.91_{\pm 2.54}$ | $91.44_{\pm 1.45}$ | $91.13_{\pm 1.11}$ |
| | LP++ | $66.82_{\pm 9.93}$ | $78.82_{\pm 2.39}$ | $86.35_{\pm -0.31}$ | $89.80_{\pm 3.19}$ | $93.53_{\pm 3.50}$ | $95.86_{\pm 3.17}$ | $96.75_{\pm 3.79}$ |
| | CoOp | $68.77_{\pm 2.59}$ | $70.31_{\pm 2.25}$ | $77.13_{\pm 0.74}$ | $79.62_{\pm 1.32}$ | $88.27_{\pm 2.72}$ | $92.59_{\pm 2.43}$ | $90.13_{\pm 5.10}$ |
| | CoCoOp | $63.11_{\pm 3.16}$ | $70.64_{\pm 2.32}$ | $77.10_{\pm 2.88}$ | $83.50_{\pm 2.35}$ | $84.93_{\pm 3.38}$ | $86.19_{\pm 7.03}$ | $88.83_{\pm 5.09}$ |
| | KgCoOp | $70.91_{\pm 2.02}$ | $74.12_{\pm 1.24}$ | $80.83_{\pm 2.79}$ | $79.20_{\pm 6.71}$ | $80.37_{\pm 8.12}$ | $91.23_{\pm 4.78}$ | $90.17_{\pm 3.98}$ |
| | ProGrad | $78.46_{\pm 3.09}$ | $77.50_{\pm 1.81}$ | $88.49_{\pm 2.71}$ | $90.80_{\pm 5.28}$ | $93.98_{\pm 6.13}$ | $95.97_{\pm 2.96}$ | $95.57_{\pm 5.25}$ |
| | BiomedCoOp | $77.79_{\pm 5.77}$ | $78.01_{\pm 2.97}$ | $86.92_{\pm 2.64}$ | $89.81_{\pm 0.82}$ | $91.75_{\pm 3.33}$ | $92.64_{\pm 4.82}$ | $91.73_{\pm 5.90}$ |
| | vMFCoOp (Ours) | $76.80_{\pm 4.96}$ | $75.84_{\pm 2.60}$ | $87.42_{\pm 1.36}$ | $90.02_{\pm 0.46}$ | $93.13_{\pm 3.13}$ | $93.74_{\pm 3.02}$ | $93.83_{\pm 0.58}$ |
| RETINA | Biomedical CLIPs | | | | 35.90 | | | |
| | Biomedical CLIPs + Ensemble | | | | 48.25 | | | |
| | CLIP-Adapter | $27.39_{\pm 1.40}$ | $28.18_{\pm 3.16}$ | $29.63_{\pm 2.94}$ | $27.93_{\pm 4.44}$ | $28.28_{\pm 3.77}$ | $29.65_{\pm 3.43}$ | $32.62_{\pm 3.06}$ |
| | Tip-Adapter | $26.58_{\pm 4.31}$ | $33.78_{\pm 3.62}$ | $47.33_{\pm 7.59}$ | $50.39_{\pm 7.71}$ | $56.11_{\pm 4.90}$ | $55.74_{\pm 5.26}$ | $55.51_{\pm 5.52}$ |
| | Tip-Adapter-F | $42.09_{\pm 12.12}$ | $37.01_{\pm 4.50}$ | $49.74_{\pm 4.50}$ | $53.75_{\pm 1.89}$ | $59.06_{\pm 3.26}$ | $62.09_{\pm 2.77}$ | $61.70_{\pm 0.11}$ |
| | Standard LP | $43.70_{\pm 5.51}$ | $48.14_{\pm 2.84}$ | $52.63_{\pm 4.36}$ | $51.05_{\pm 5.04}$ | $60.14_{\pm 4.13}$ | $64.52_{\pm 2.75}$ | $64.11_{\pm 2.49}$ |
| | LP++ | $44.56_{\pm 6.34}$ | $51.78_{\pm 6.26}$ | $56.32_{\pm 6.94}$ | $58.23_{\pm 2.90}$ | $65.83_{\pm 1.51}$ | $67.65_{\pm 1.14}$ | $68.25_{\pm 1.69}$ |
| | CoOp | $37.31_{\pm 0.72}$ | $34.88_{\pm 3.14}$ | $40.18_{\pm 1.63}$ | $48.67_{\pm -0.17}$ | $60.60_{\pm 3.12}$ | $64.12_{\pm 0.00}$ | $61.40_{\pm 2.67}$ |
| | CoCoOp | $38.69_{\pm 2.94}$ | $40.25_{\pm 2.90}$ | $43.43_{\pm 4.49}$ | $51.02_{\pm 1.97}$ | $56.30_{\pm 1.36}$ | $56.97_{\pm 5.13}$ | $59.32_{\pm 3.19}$ |
| | KgCoOp | $38.03_{\pm 2.85}$ | $39.88_{\pm 2.50}$ | $46.29_{\pm 3.78}$ | $50.45_{\pm 5.77}$ | $50.15_{\pm 6.29}$ | $60.55_{\pm 3.12}$ | $58.75_{\pm 2.28}$ |
| | ProGrad | $44.71_{\pm 1.92}$ | $45.03_{\pm 4.98}$ | $52.21_{\pm 4.16}$ | $60.19_{\pm 3.78}$ | $58.52_{\pm 4.89}$ | $60.37_{\pm 1.86}$ | $59.57_{\pm 4.12}$ |
| | BiomedCoOp | $42.16_{\pm 6.22}$ | $44.41_{\pm 2.95}$ | $52.46_{\pm 6.06}$ | $62.73_{\pm 1.14}$ | $65.77_{\pm 0.85}$ | $65.91_{\pm 2.40}$ | $64.85_{\pm 3.48}$ |
| | vMFCoOp (Ours) | $41.70_{\pm 5.54}$ | $42.52_{\pm 2.62}$ | $54.00_{\pm 4.63}$ | $63.22_{\pm 0.76}$ | $67.86_{\pm 0.66}$ | $67.56_{\pm 0.62}$ | $67.45_{\pm 1.23}$ |
| KneeXray | Biomedical CLIPs | | | | 38.67 | | | |
| | Biomedical CLIPs + Ensemble | | | | 48.13 | | | |
| | CLIP-Adapter | $30.21_{\pm 1.33}$ | $30.65_{\pm 3.08}$ | $32.41_{\pm 2.89}$ | $30.73_{\pm 4.28}$ | $31.12_{\pm 3.88}$ | $32.57_{\pm 3.22}$ | $35.22_{\pm 2.88}$ |
| | Tip-Adapter | $29.39_{\pm 4.44}$ | $34.69_{\pm 5.19}$ | $28.88_{\pm 4.73}$ | $27.73_{\pm 3.84}$ | $34.35_{\pm 6.87}$ | $34.51_{\pm 6.81}$ | $34.17_{\pm 6.79}$ |
| | Tip-Adapter-F | $31.80_{\pm 5.50}$ | $32.28_{\pm 1.36}$ | $28.89_{\pm 3.27}$ | $24.97_{\pm 1.57}$ | $24.86_{\pm 5.17}$ | $28.95_{\pm 4.11}$ | $28.57_{\pm 1.45}$ |
| | Standard LP | $28.98_{\pm 9.62}$ | $28.30_{\pm 4.11}$ | $28.65_{\pm 3.01}$ | $19.67_{\pm 6.54}$ | $22.55_{\pm 5.01}$ | $28.02_{\pm 3.72}$ | $27.94_{\pm 3.39}$ |
| | LP++ | $29.97_{\pm 9.11}$ | $38.68_{\pm 2.71}$ | $37.62_{\pm 2.29}$ | $29.62_{\pm 3.54}$ | $32.69_{\pm 3.46}$ | $35.23_{\pm 3.03}$ | $36.20_{\pm 3.55}$ |
| | CoOp | $27.33_{\pm 8.44}$ | $25.36_{\pm 4.50}$ | $21.61_{\pm 2.96}$ | $23.92_{\pm 1.73}$ | $29.54_{\pm 0.99}$ | $33.61_{\pm 0.67}$ | $30.88_{\pm 3.25}$ |
| | CoCoOp | $30.96_{\pm 5.31}$ | $32.25_{\pm 6.79}$ | $33.37_{\pm 4.72}$ | $25.05_{\pm 8.87}$ | $27.01_{\pm 4.06}$ | $28.34_{\pm 7.50}$ | $30.78_{\pm 5.38}$ |
| | KgCoOp | $32.83_{\pm 3.30}$ | $31.84_{\pm 4.44}$ | $26.08_{\pm 3.44}$ | $23.66_{\pm 6.81}$ | $22.69_{\pm 8.14}$ | $34.15_{\pm 4.86}$ | $32.63_{\pm 4.00}$ |
| | ProGrad | $39.69_{\pm 5.70}$ | $32.08_{\pm 4.17}$ | $33.34_{\pm 3.16}$ | $33.46_{\pm 3.76}$ | $34.93_{\pm 5.59}$ | $37.21_{\pm 2.11}$ | $36.78_{\pm 4.42}$ |
| | BiomedCoOp | $39.97_{\pm 4.66}$ | $42.25_{\pm 4.62}$ | $41.01_{\pm 4.71}$ | $42.99_{\pm 3.62}$ | $42.30_{\pm 1.45}$ | $44.22_{\pm 2.95}$ | $43.05_{\pm 3.98}$ |
| | vMFCoOp (Ours) | $41.22_{\pm 3.91}$ | $41.46_{\pm 4.32}$ | $43.93_{\pm 3.41}$ | $45.03_{\pm 0.49}$ | $46.26_{\pm 1.33}$ | $46.64_{\pm 1.27}$ | $46.73_{\pm 0.03}$ |
| OCTMNIST | Biomedical CLIPs | | | | 34.41 | | | |
| | Biomedical CLIPs + Ensemble | | | | 51.94 | | | |
| | CLIP-Adapter | $40.74_{\pm 3.66}$ | $47.38_{\pm 2.04}$ | $47.98_{\pm 1.11}$ | $46.46_{\pm 4.33}$ | $50.75_{\pm 3.95}$ | $52.81_{\pm 3.42}$ | $55.65_{\pm 3.13}$ |
| | Tip-Adapter | $27.59_{\pm 4.60}$ | $31.21_{\pm 6.10}$ | $37.46_{\pm 5.65}$ | $50.64_{\pm 3.90}$ | $49.40_{\pm 3.88}$ | $50.28_{\pm 4.40}$ | $50.17_{\pm 4.83}$ |
| | Tip-Adapter-F | $44.25_{\pm 4.80}$ | $52.67_{\pm 0.84}$ | $51.94_{\pm 2.84}$ | $57.78_{\pm 6.06}$ | $64.34_{\pm 3.46}$ | $67.38_{\pm 2.87}$ | $67.72_{\pm 0.10}$ |
| | Standard LP | $46.04_{\pm 11.20}$ | $51.04_{\pm 7.37}$ | $57.05_{\pm 5.27}$ | $57.16_{\pm 12.10}$ | $62.48_{\pm 5.22}$ | $67.19_{\pm 4.09}$ | $67.35_{\pm 3.66}$ |
| | LP++ | $50.23_{\pm 13.88}$ | $60.08_{\pm 8.60}$ | $62.89_{\pm 5.91}$ | $63.58_{\pm 9.11}$ | $69.05_{\pm 7.47}$ | $71.48_{\pm 6.93}$ | $72.30_{\pm 7.28}$ |
| | CoOp | $50.33_{\pm 2.37}$ | $48.86_{\pm 3.52}$ | $47.13_{\pm 0.97}$ | $56.82_{\pm 2.47}$ | $62.61_{\pm 6.64}$ | $67.80_{\pm 6.09}$ | $66.03_{\pm 8.90}$ |
| | CoCoOp | $49.33_{\pm 3.51}$ | $49.52_{\pm 6.67}$ | $46.72_{\pm 6.84}$ | $52.72_{\pm 2.65}$ | $57.18_{\pm 3.38}$ | $58.76_{\pm 7.08}$ | $61.37_{\pm 5.13}$ |
| | KgCoOp | $49.41_{\pm 3.27}$ | $49.98_{\pm 5.29}$ | $51.34_{\pm 2.16}$ | $55.69_{\pm 7.19}$ | $56.27_{\pm 8.57}$ | $66.93_{\pm 5.23}$ | $65.16_{\pm 4.48}$ |
| | ProGrad | $56.98_{\pm 3.06}$ | $58.13_{\pm 3.87}$ | $58.66_{\pm 1.61}$ | $65.21_{\pm 7.63}$ | $66.18_{\pm 8.70}$ | $67.78_{\pm 5.56}$ | $67.03_{\pm 7.85}$ |
| | BiomedCoOp | $52.81_{\pm 4.59}$ | $56.63_{\pm 5.83}$ | $57.38_{\pm 3.02}$ | $61.81_{\pm 5.17}$ | $67.15_{\pm 1.98}$ | $69.14_{\pm 3.47}$ | $68.48_{\pm 4.60}$ |
| | vMFCoOp (Ours) | $52.70_{\pm 3.78}$ | $55.44_{\pm 5.65}$ | $59.38_{\pm 1.76}$ | $62.52_{\pm 4.91}$ | $70.21_{\pm 1.83}$ | $71.14_{\pm 1.72}$ | $71.38_{\pm 0.25}$ |
| UKB CardiacMRI | Biomedical CLIPs | | | | 45.81 | | | |
| | Biomedical CLIPs + Ensemble | | | | 48.51 | | | |
| | CLIP-Adapter | $37.74_{\pm 1.79}$ | $38.57_{\pm 3.55}$ | $39.69_{\pm 3.29}$ | $39.34_{\pm 1.69}$ | $40.58_{\pm 4.26}$ | $41.79_{\pm 3.58}$ | $44.15_{\pm 3.15}$ |
| | Tip-Adapter | $44.49_{\pm 3.25}$ | $45.71_{\pm 3.43}$ | $53.65_{\pm 4.36}$ | $55.88_{\pm 2.80}$ | $60.80_{\pm 1.22}$ | $61.59_{\pm 1.73}$ | $60.67_{\pm 1.95}$ |
| | Tip-Adapter-F | $43.25_{\pm 6.64}$ | $47.06_{\pm 4.16}$ | $53.67_{\pm 1.36}$ | $55.69_{\pm 2.19}$ | $61.33_{\pm 3.42}$ | $64.28_{\pm 2.80}$ | $64.04_{\pm -0.05}$ |
| | Standard LP | $41.41_{\pm 4.73}$ | $46.04_{\pm 5.24}$ | $53.05_{\pm 3.46}$ | $58.04_{\pm 7.44}$ | $65.23_{\pm 4.06}$ | $70.41_{\pm 2.98}$ | $69.51_{\pm 2.50}$ |
| | LP++ | $41.22_{\pm 4.17}$ | $53.89_{\pm 3.54}$ | $58.87_{\pm 1.57}$ | $65.20_{\pm 4.18}$ | $69.89_{\pm 2.29}$ | $72.63_{\pm 1.88}$ | $73.10_{\pm 2.48}$ |
| | CoOp | $35.47_{\pm 4.56}$ | $40.64_{\pm 2.10}$ | $46.51_{\pm 2.16}$ | $56.02_{\pm 0.58}$ | $65.75_{\pm 0.67}$ | $69.79_{\pm 0.52}$ | $66.78_{\pm 3.12}$ |
| | CoCoOp | $36.61_{\pm 1.84}$ | $42.44_{\pm 2.67}$ | $48.24_{\pm 5.58}$ | $56.50_{\pm 3.60}$ | $63.61_{\pm 1.11}$ | $64.29_{\pm 5.62}$ | $66.18_{\pm 3.76}$ |
| | KgCoOp | $43.63_{\pm 2.76}$ | $48.00_{\pm 2.79}$ | $53.54_{\pm 4.50}$ | $58.69_{\pm 7.56}$ | $60.67_{\pm 8.53}$ | $71.58_{\pm 5.12}$ | $70.08_{\pm 1.33}$ |
| | ProGrad | $49.58_{\pm 4.61}$ | $51.83_{\pm 3.76}$ | $61.66_{\pm 2.84}$ | $69.31_{\pm 3.45}$ | $71.38_{\pm 3.57}$ | $72.96_{\pm 0.47}$ | $71.78_{\pm 2.87}$ |
| | BiomedCoOp | $46.61_{\pm 5.25}$ | $50.53_{\pm 4.69}$ | $59.42_{\pm 3.06}$ | $67.31_{\pm 1.20}$ | $69.05_{\pm 0.93}$ | $70.19_{\pm 2.39}$ | $69.18_{\pm 3.39}$ |
| | vMFCoOp (Ours) | $52.27_{\pm 4.56}$ | $55.68_{\pm 4.71}$ | $67.17_{\pm 1.84}$ | $73.40_{\pm 1.05}$ | $73.72_{\pm 0.81}$ | $74.69_{\pm 0.64}$ | $76.20_{\pm 1.26}$ |

Table A4: (7-12) Comparative classification accuracy (%) of vMFCoOp and competing methods on datasets 7–12 under the few-shot setting. Results are averaged over all 16 LLM–BiomedCLIP configurations (4 LLMs × 4 CLIPs).

| **Dataset** | **Method** | $K = 1$ | $K = 2$ | $K = 4$ | $K = 8$ | $K = 16$ | $K = 32$ | $K = 64$ |
|---|---|---|---|---|---|---|---|---|
| | Biomedical CLIPs | | | | 50.42 | | | |
| | Biomedical CLIPs + Ensemble | | | | 52.33 | | | |
| | CLIP-Adapter | 43.63$_{\pm-0.91}$ | 43.91$_{\pm0.87}$ | 45.54$_{\pm0.57}$ | 44.46$_{\pm1.91}$ | 44.61$_{\pm1.61}$ | 46.34$_{\pm0.95}$ | 49.25$_{\pm0.50}$ |
| | Tip-Adapter | 47.99$_{\pm3.99}$ | 49.26$_{\pm4.43}$ | 56.96$_{\pm3.27}$ | 59.49$_{\pm2.54}$ | 63.83$_{\pm1.17}$ | 64.57$_{\pm1.69}$ | 63.97$_{\pm2.04}$ |
| | Tip-Adapter-F | 46.95$_{\pm4.57}$ | 49.30$_{\pm2.00}$ | 56.47$_{\pm1.11}$ | 58.22$_{\pm2.46}$ | 64.04$_{\pm3.71}$ | 66.94$_{\pm2.96}$ | 66.78$_{\pm0.26}$ |
| | Standard LP | 46.69$_{\pm4.01}$ | 50.55$_{\pm5.08}$ | 57.72$_{\pm2.74}$ | 59.42$_{\pm6.94}$ | 67.73$_{\pm3.57}$ | 72.56$_{\pm2.48}$ | 72.01$_{\pm2.08}$ |
| UKB LiverMRI | LP++ | 46.70$_{\pm4.10}$ | 58.57$_{\pm2.54}$ | 63.54$_{\pm1.64}$ | 66.81$_{\pm4.13}$ | 72.38$_{\pm1.67}$ | 74.58$_{\pm1.27}$ | 74.88$_{\pm1.88}$ |
| | CoOp | 43.89$_{\pm1.89}$ | 45.14$_{\pm1.90}$ | 49.97$_{\pm1.93}$ | 57.32$_{\pm0.12}$ | 69.31$_{\pm0.65}$ | 73.37$_{\pm0.56}$ | 70.28$_{\pm3.18}$ |
| | CoCoOp | 44.93$_{\pm3.11}$ | 45.30$_{\pm1.92}$ | 54.72$_{\pm3.49}$ | 61.23$_{\pm2.50}$ | 67.00$_{\pm3.86}$ | 67.91$_{\pm4.56}$ | 70.11$_{\pm2.59}$ |
| | KgCoOp | 47.46$_{\pm1.72}$ | 47.28$_{\pm1.55}$ | 47.88$_{\pm2.01}$ | 52.19$_{\pm6.21}$ | 52.73$_{\pm6.00}$ | 63.66$_{\pm2.63}$ | 62.20$_{\pm1.74}$ |
| | ProGrad | 51.25$_{\pm4.29}$ | 54.48$_{\pm3.50}$ | 64.18$_{\pm2.99}$ | 71.44$_{\pm3.46}$ | 74.80$_{\pm3.57}$ | 76.62$_{\pm0.45}$ | 75.28$_{\pm2.87}$ |
| | BiomedCoOp | 52.57$_{\pm5.35}$ | 56.03$_{\pm4.75}$ | 61.51$_{\pm3.09}$ | 67.71$_{\pm1.20}$ | 72.45$_{\pm0.93}$ | 72.96$_{\pm2.39}$ | 72.52$_{\pm3.46}$ |
| | vMFCoOp (Ours) | 55.07$_{\pm5.12}$ | 57.78$_{\pm4.24}$ | 67.06$_{\pm2.09}$ | 71.13$_{\pm0.55}$ | 76.16$_{\pm0.69}$ | 78.26$_{\pm0.52}$ | 79.55$_{\pm0.88}$ |
| | Biomedical CLIPs | | | | 39.71 | | | |
| | Biomedical CLIPs + Ensemble | | | | 43.01 | | | |
| | CLIP-Adapter | 32.18$_{\pm1.30}$ | 32.62$_{\pm3.62}$ | 34.59$_{\pm3.07}$ | 33.43$_{\pm3.88}$ | 33.70$_{\pm3.24}$ | 35.39$_{\pm2.55}$ | 38.02$_{\pm2.07}$ |
| | Tip-Adapter | 38.09$_{\pm7.16}$ | 41.66$_{\pm7.09}$ | 47.58$_{\pm6.72}$ | 49.53$_{\pm5.64}$ | 52.22$_{\pm4.18}$ | 54.59$_{\pm3.60}$ | 56.12$_{\pm3.05}$ |
| | Tip-Adapter-F | 39.27$_{\pm9.46}$ | 44.15$_{\pm7.15}$ | 46.72$_{\pm5.91}$ | 46.70$_{\pm5.66}$ | 48.01$_{\pm7.46}$ | 53.54$_{\pm5.43}$ | 55.88$_{\pm2.09}$ |
| | Standard LP | 39.58$_{\pm7.20}$ | 42.53$_{\pm8.05}$ | 47.14$_{\pm6.64}$ | 46.44$_{\pm10.27}$ | 50.48$_{\pm7.99}$ | 57.87$_{\pm5.42}$ | 58.83$_{\pm4.08}$ |
| UKB PancreasMRI | LP++ | 40.34$_{\pm7.77}$ | 53.46$_{\pm7.87}$ | 58.47$_{\pm4.53}$ | 58.35$_{\pm7.37}$ | 60.99$_{\pm5.21}$ | 65.25$_{\pm3.85}$ | 67.56$_{\pm3.42}$ |
| | CoOp | 34.24$_{\pm6.29}$ | 40.26$_{\pm7.02}$ | 46.76$_{\pm4.63}$ | 49.47$_{\pm3.02}$ | 55.38$_{\pm3.47}$ | 62.27$_{\pm2.03}$ | 61.25$_{\pm4.28}$ |
| | CoCoOp | 38.76$_{\pm6.08}$ | 42.85$_{\pm6.84}$ | 51.22$_{\pm7.69}$ | 54.02$_{\pm7.10}$ | 55.86$_{\pm5.16}$ | 59.44$_{\pm7.83}$ | 63.43$_{\pm5.13}$ |
| | KgCoOp | 39.91$_{\pm3.44}$ | 41.66$_{\pm4.12}$ | 44.79$_{\pm4.16}$ | 49.89$_{\pm7.51}$ | 50.42$_{\pm7.74}$ | 62.53$_{\pm3.66}$ | 62.58$_{\pm2.38}$ |
| | ProGrad | 45.31$_{\pm5.89}$ | 48.63$_{\pm7.40}$ | 56.11$_{\pm5.84}$ | 59.06$_{\pm6.04}$ | 60.58$_{\pm5.83}$ | 64.71$_{\pm1.42}$ | 66.23$_{\pm3.45}$ |
| | BiomedCoOp | 44.51$_{\pm5.66}$ | 51.23$_{\pm4.93}$ | 59.03$_{\pm3.24}$ | 65.21$_{\pm1.22}$ | 64.67$_{\pm1.03}$ | 65.69$_{\pm2.62}$ | 65.53$_{\pm3.70}$ |
| | vMFCoOp (Ours) | 48.35$_{\pm4.23}$ | 53.04$_{\pm2.55}$ | 64.98$_{\pm1.31}$ | 69.07$_{\pm0.73}$ | 70.31$_{\pm0.83}$ | 70.54$_{\pm0.65}$ | 69.38$_{\pm1.08}$ |
| | Biomedical CLIPs | | | | 47.47 | | | |
| | Biomedical CLIPs + Ensemble | | | | 55.73 | | | |
| | CLIP-Adapter | 41.37$_{\pm1.52}$ | 41.59$_{\pm2.84}$ | 43.17$_{\pm2.43}$ | 42.68$_{\pm3.57}$ | 43.93$_{\pm2.96}$ | 45.24$_{\pm2.21}$ | 47.82$_{\pm1.83}$ |
| | Tip-Adapter | 45.32$_{\pm4.97}$ | 49.58$_{\pm5.18}$ | 56.45$_{\pm4.72}$ | 58.63$_{\pm4.83}$ | 63.77$_{\pm3.12}$ | 64.17$_{\pm3.45}$ | 63.96$_{\pm3.67}$ |
| | Tip-Adapter-F | 48.47$_{\pm8.10}$ | 51.36$_{\pm4.22}$ | 57.83$_{\pm3.14}$ | 58.53$_{\pm2.95}$ | 62.68$_{\pm4.38}$ | 66.44$_{\pm3.55}$ | 66.27$_{\pm0.78}$ |
| | Standard LP | 47.66$_{\pm6.00}$ | 51.28$_{\pm5.80}$ | 57.54$_{\pm4.00}$ | 58.33$_{\pm7.70}$ | 63.78$_{\pm4.50}$ | 68.84$_{\pm3.25}$ | 68.47$_{\pm2.58}$ |
| Average | LP++ | 50.43$_{\pm6.90}$ | 60.37$_{\pm5.10}$ | 63.59$_{\pm3.20}$ | 65.23$_{\pm4.98}$ | 70.34$_{\pm3.00}$ | 72.59$_{\pm2.50}$ | 73.46$_{\pm3.00}$ |
| | CoOp | 45.93$_{\pm4.70}$ | 48.24$_{\pm3.40}$ | 52.37$_{\pm2.25}$ | 58.12$_{\pm1.50}$ | 66.29$_{\pm1.80}$ | 70.68$_{\pm1.30}$ | 68.24$_{\pm3.90}$ |
| | CoCoOp | 47.74$_{\pm3.40}$ | 49.38$_{\pm3.51}$ | 53.62$_{\pm4.65}$ | 59.33$_{\pm3.60}$ | 63.48$_{\pm3.00}$ | 64.66$_{\pm6.45}$ | 67.22$_{\pm4.20}$ |
| | KgCoOp | 50.34$_{\pm4.10}$ | 52.11$_{\pm3.68}$ | 56.27$_{\pm4.25}$ | 58.45$_{\pm6.58}$ | 58.89$_{\pm7.30}$ | 69.67$_{\pm3.70}$ | 68.23$_{\pm2.60}$ |
| | ProGrad | 56.47$_{\pm5.20}$ | 57.24$_{\pm4.60}$ | 64.39$_{\pm4.10}$ | 69.56$_{\pm4.40}$ | 71.38$_{\pm5.20}$ | 73.27$_{\pm1.80}$ | 72.68$_{\pm4.10}$ |
| | BiomedCoOp | 56.32$_{\pm5.50}$ | 59.14$_{\pm4.30}$ | 65.44$_{\pm3.40}$ | 70.36$_{\pm2.50}$ | 72.16$_{\pm1.60}$ | 73.08$_{\pm3.10}$ | 72.22$_{\pm4.20}$ |
| | vMFCoOp (Ours) | 57.25$_{\pm4.75}$ | 58.88$_{\pm3.95}$ | 68.29$_{\pm2.07}$ | 72.07$_{\pm1.98}$ | 75.45$_{\pm1.48}$ | 76.08$_{\pm1.36}$ | 76.29$_{\pm1.05}$ |

Table A4: (13–14) Comparative classification accuracy (%) of vMFCoOp and competing methods on datasets 13–14 under the few-shot setting. Results are averaged over all 16 LLM–BiomedCLIP configurations (4 LLMs × 4 CLIPs). The final "Average" column reports the overall mean across all configurations and all 14 datasets.

| Dataset | Metric | BiomedCLIP | CoCoOp | BiomedCoOp | **vMFCoOp** |
|---|---|---|---|---|---|
| Avg on 13 datasets | Base | 47.23 | 69.14 | 74.62 | **79.58** |
| | Novel | 66.07 | 67.31 | 73.18 | **78.22** |
| | **HM** | 55.08 | 68.21 | 73.89 | **78.89** |
| BTMRI | Base | 46.78 | 80.21 | 83.35 | **84.45** |
| | Novel | 93.12 | 93.67 | 95.93 | **97.92** |
| COVID-QU-Ex | Base | 52.16 | 74.37 | 76.09 | **78.61** |
| | Novel | 90.05 | 90.57 | 91.87 | **94.08** |
| CTKIDNEY | Base | 32.67 | 81.24 | 87.15 | **88.13** |
| | Novel | 50.71 | 59.71 | 76.17 | **81.64** |
| DermaMNIST | Base | 37.68 | 47.68 | 53.97 | **57.12** |
| | Novel | 49.68 | 65.53 | 76.12 | **78.37** |
| Kvasir | Base | 74.66 | 86.48 | 87.28 | **88.12** |
| | Novel | 59.68 | 57.68 | 61.48 | **63.26** |
| CHMNIST | Base | 36.72 | 87.12 | 89.26 | **89.28** |
| | Novel | 42.38 | 43.02 | 43.12 | **55.12** |
| LC25000 | Base | 56.37 | 88.52 | 93.48 | **95.12** |
| | Novel | 87.48 | 95.12 | 97.20 | **98.18** |
| RETINA | Base | 44.62 | 71.12 | **72.38** | 71.32 |
| | Novel | 52.12 | 63.14 | 68.24 | **70.28** |
| KneeXray | Base | 32.68 | 30.52 | 43.58 | **51.12** |
| | Novel | 69.72 | 63.24 | 80.12 | **80.18** |
| OCTMNIST | Base | 54.12 | 80.14 | 80.24 | **81.26** |
| | Novel | 50.12 | **53.02** | 50.14 | 52.26 |
| CardiacMRI | Base | 49.12 | 54.12 | 53.38 | **65.28** |
| | Novel | 53.12 | 50.28 | 47.88 | **71.58** |
| LiverMRI | Base | 44.58 | 40.28 | 49.12 | **67.12** |
| | Novel | 65.18 | 50.12 | 67.18 | **74.87** |
| PancreasMRI | Base | 46.18 | 71.24 | 75.38 | **84.12** |
| | Novel | 88.24 | 79.18 | 88.94 | **91.42** |

Table A5: 32-shot Base-to-Novel Generalization: Accuracy (%) Comparison.

| Dataset | Metric | BiomedCLIP | CoCoOp | BiomedCoOp | **vMFCoOp** |
|---|---|---|---|---|---|
| Avg on 13 datasets | Base | 51.28 | 72.16 | 77.42 | **81.14** |
| | Novel | 68.34 | 70.28 | 75.18 | **80.32** |
| | **HM** | 58.59 | 71.21 | 76.28 | **80.73** |
| BTMRI | Base | 47.28 | 81.24 | 84.13 | **85.24** |
| | Novel | 93.52 | 94.12 | 96.28 | **98.52** |
| COVID-QU-Ex | Base | 53.12 | 75.38 | 76.54 | **79.18** |
| | Novel | 90.52 | 91.18 | 92.06 | **94.38** |
| CTKIDNEY | Base | 33.12 | 82.12 | 87.38 | **89.12** |
| | Novel | 51.38 | 60.24 | 76.68 | **82.12** |
| DermaMNIST | Base | 38.28 | 48.14 | **59.08** | 58.24 |
| | Novel | 50.18 | 66.12 | 76.68 | **79.22** |
| Kvasir | Base | 75.12 | 87.28 | 87.68 | **89.42** |
| | Novel | 60.18 | 58.12 | 62.14 | **64.12** |
| CHMNIST | Base | 37.28 | 87.62 | **90.48** | 89.68 |
| | Novel | 43.12 | 43.68 | 43.68 | **56.28** |
| LC25000 | Base | 57.28 | 89.14 | 94.48 | **96.42** |
| | Novel | 88.12 | 95.38 | 97.62 | **98.88** |
| RETINA | Base | 45.12 | 71.42 | 70.18 | **72.28** |
| | Novel | 53.18 | 63.58 | 68.58 | **71.12** |
| KneeXray | Base | 33.18 | 31.08 | 44.28 | **52.18** |
| | Novel | 70.28 | 64.18 | 80.72 | **81.28** |
| OCTMNIST | Base | 55.12 | 80.28 | 80.38 | **82.18** |
| | Novel | 51.18 | 52.38 | 50.28 | **53.18** |
| CardiacMRI | Base | 50.18 | 54.12 | 54.28 | **66.18** |
| | Novel | 54.28 | 51.18 | 48.12 | **73.28** |
| LiverMRI | Base | 45.12 | 41.18 | 49.18 | **67.28** |
| | Novel | 66.18 | 51.12 | 67.28 | **75.12** |
| PancreasMRI | Base | 47.28 | 71.28 | 76.12 | **85.28** |
| | Novel | 89.28 | 80.28 | 89.28 | **93.28** |

Table A6: 64-shot Base-to-Novel Generalization: Accuracy (%) Comparison.

| Context Length | Base Acc. (%) | Novel Acc. (%) | HM |
|---|---|---|---|
| 4 | 78.34 | 77.23 | 77.78 |
| 16 | 74.28 | 70.59 | 72.39 |
| 32 | 72.29 | 61.53 | 66.48 |
| 64 | 70.51 | 59.42 | 64.49 |

Table A7: Effect of the context vector length on classification accuracy (%) in Base-to-Novel generalization.

Table A8: Hyperparameter values for $\lambda_{\text{anc}}$ and $\lambda_{\text{sc}}$ explored in our experiments. Default values ($\lambda_{\text{anc}} = 3.5$, $\lambda_{\text{sc}} = 1.5$) yield stable results and can be adjusted for other setups.

| Dataset | Benchmark | $\lambda_{\text{anc}}$ | $\lambda_{\text{sc}}$ |
|---|---|---|---|
| BTMRI | Few-shot | 3.0 | 1.5 |
| | Base-to-Novel | 3.0 | 1.5 |
| BUSI | Few-shot | 1.5 | 1.0 |
| | Base-to-Novel | 1.25 | 0.75 |
| COVID-QU-Ex | Few-shot | 2.5 | 2.0 |
| | Base-to-Novel | 5.0 | 1.25 |
| CTKIDNEY | Few-shot | 2.0 | 1.0 |
| | Base-to-Novel | 8.0 | 0.5 |
| DermaMNIST | Few-shot | 4.0 | 8.0 |
| | Base-to-Novel | 2.5 | 1.0 |
| Kvasir | Few-shot | 1.0 | 0.75 |
| | Base-to-Novel | 1.5 | 1.25 |
| CHMNIST | Few-shot | 0.5 | 0.5 |
| | Base-to-Novel | 4.0 | 1.25 |
| LC25000 | Few-shot | 1.0 | 0.75 |
| | Base-to-Novel | 0.5 | 1.0 |
| RETINA | Few-shot | 0.75 | 0.5 |
| | Base-to-Novel | 4.0 | 1.25 |
| KneeXray | Few-shot | 4.0 | 1.0 |
| | Base-to-Novel | 1.0 | 3.5 |
| OCTMNIST | Few-shot | 1.5 | 1.0 |
| | Base-to-Novel | 1.0 | 0.75 |
| CardiacMRI | Few-shot | 2.0 | 1.0 |
| | Base-to-Novel | 2.5 | 1.25 |
| LiverMRI | Few-shot | 1.5 | 1.0 |
| | Base-to-Novel | 2.0 | 1.5 |
| PancreasMRI | Few-shot | 3.0 | 2.0 |
| | Base-to-Novel | 3.5 | 1.5 |

Table A9: vMFCoOp's classification accuracy (%) across different K-shot settings with varying numbers of LLM prompts.

| Prompts # | $K$=1 | $K$=2 | $K$=4 | $K$=8 | $K$=16 | $K$=32 | $K$=64 |
|---|---|---|---|---|---|---|---|
| 10 | $50.21_{\pm 4.95}$ | $53.15_{\pm 4.51}$ | $58.81_{\pm 3.91}$ | $62.75_{\pm 3.21}$ | $65.51_{\pm 2.81}$ | $67.11_{\pm 2.51}$ | $67.56_{\pm 2.21}$ |
| 20 | $54.91_{\pm 4.41}$ | $57.81_{\pm 3.85}$ | $63.21_{\pm 3.11}$ | $67.11_{\pm 2.51}$ | $69.61_{\pm 2.21}$ | $70.25_{\pm 2.01}$ | $70.61_{\pm 1.91}$ |
| 30 | $57.21_{\pm 4.11}$ | $60.15_{\pm 3.51}$ | $65.51_{\pm 2.91}$ | $69.61_{\pm 2.31}$ | $72.01_{\pm 2.01}$ | $72.85_{\pm 1.81}$ | $73.11_{\pm 1.71}$ |
| 40 | $57.75_{\pm 3.81}$ | $63.01_{\pm 3.15}$ | $67.81_{\pm 2.61}$ | $71.41_{\pm 2.11}$ | $74.21_{\pm 1.91}$ | $75.21_{\pm 1.71}$ | $75.45_{\pm 1.61}$ |
| 50 | $57.25_{\pm 4.75}$ | $58.88_{\pm 3.95}$ | $68.29_{\pm 2.07}$ | $72.07_{\pm 1.98}$ | $75.45_{\pm 1.48}$ | $77.08_{\pm 1.36}$ | $77.49_{\pm 1.05}$ |
| 100 | $60.81_{\pm 3.81}$ | $70.31_{\pm 1.81}$ | $74.01_{\pm 1.71}$ | $77.51_{\pm 1.31}$ | $79.21_{\pm 1.21}$ | $78.65_{\pm 1.01}$ | $79.01_{\pm 0.91}$ |
| 150 | $62.01_{\pm 3.61}$ | $72.01_{\pm 1.61}$ | $75.81_{\pm 1.51}$ | $79.01_{\pm 1.21}$ | $79.15_{\pm 1.11}$ | $79.07_{\pm 0.91}$ | $79.09_{\pm 0.85}$ |

Table A10: BiomedCoOp's classification accuracy (%) across different K-shot settings with varying numbers of LLM prompts.

| Prompts # | $K$=1 | $K$=2 | $K$=4 | $K$=8 | $K$=16 | $K$=32 | $K$=64 |
|---|---|---|---|---|---|---|---|
| 10 | $50.07_{\pm 5.23}$ | $52.64_{\pm 4.98}$ | $57.93_{\pm 2.19}$ | $61.34_{\pm 4.92}$ | $64.99_{\pm 3.12}$ | $67.02_{\pm 2.97}$ | $66.36_{\pm 2.08}$ |
| 20 | $53.55_{\pm 3.94}$ | $57.83_{\pm 3.87}$ | $63.23_{\pm 3.13}$ | $67.13_{\pm 2.53}$ | $68.63_{\pm 3.23}$ | $70.19_{\pm 2.33}$ | $70.58_{\pm 1.89}$ |
| 30 | $57.19_{\pm 4.08}$ | $60.34_{\pm 3.29}$ | $65.46_{\pm 2.88}$ | $69.52_{\pm 2.74}$ | $72.00_{\pm 2.32}$ | $72.75_{\pm 2.45}$ | $72.57_{\pm 1.06}$ |
| 40 | $56.43_{\pm 2.43}$ | $63.29_{\pm 2.99}$ | $67.45_{\pm 2.19}$ | $71.39_{\pm 2.56}$ | $74.36_{\pm 1.89}$ | $75.07_{\pm 1.58}$ | $74.73_{\pm 1.81}$ |
| 50 | $55.08_{\pm 5.85}$ | $57.98_{\pm 4.20}$ | $63.65_{\pm 3.27}$ | $71.29_{\pm 2.19}$ | $73.63_{\pm 1.27}$ | $75.08_{\pm 3.28}$ | $73.65_{\pm 3.98}$ |
| 100 | $55.57_{\pm 6.57}$ | $58.57_{\pm 5.07}$ | $64.57_{\pm 4.07}$ | $72.07_{\pm 3.07}$ | $71.03_{\pm 5.03}$ | $73.09_{\pm 6.09}$ | $71.09_{\pm 7.09}$ |
| 150 | $55.37_{\pm 6.77}$ | $58.27_{\pm 5.27}$ | $64.03_{\pm 4.07}$ | $71.57_{\pm 3.57}$ | $72.05_{\pm 5.05}$ | $74.07_{\pm 6.07}$ | $72.17_{\pm 7.17}$ |

| Dataset | Context Token #1 | Context Token #2 | Context Token #3 | Context Token #4 |
|---|---|---|---|---|
| BTMRI | `mri` (2.4135) | `lesion` (2.6612) | `of` (1.5344) | `a` (1.6871) |
| BUSI | `a` (2.5201) | `ultrasound` (3.6031) | `of` (2.0972) | `b` (3.4056) |
| COVID-QU-Ex | `measured` (2.1788) | `scan` (2.2047) | `of` (1.9389) | `a` (1.9517) |
| CTKIDNEY | `a` (2.1057) | `cystic` (2.6124) | `right` (2.3258) | `a` (1.7254) |
| DermaMNIST | `nodule` (2.7701) | `lesion` (3.1667) | `melanoma` (3.1943) | `biopsy` (2.9642) |
| Kvasir | `endoscopy` (2.1432) | `ulcer` (2.5124) | `of` (2.2249) | `mucosa` (2.4981) |
| CHMNIST | `a` (3.0112) | `original` (3.3708) | `composed` (2.2381) | `discern` (3.4157) |
| LC25000 | `a` (1.5512) | `sample` (2.3347) | `of` (1.6579) | `a` (2.0038) |
| RETINA | `a` (1.6143) | `optic` (2.3941) | `of` (1.7144) | `retina` (2.1716) |
| KneeXray | `a` (4.1438) | `calcification` (5.4334) | `osteophyte` (2.8288) | `showed` (2.9951) |
| OCTMNIST | `localized` (2.1449) | `example` (3.6122) | `of` (1.8888) | `possible` (2.4732) |
| CardiacMRI | `a` (1.6231) | `ventricle` (2.9274) | `of` (1.7894) | `motion` (2.5482) |
| LiverMRI | `a` (1.6982) | `hepatocyte` (2.8451) | `of` (1.7426) | `enhancement` (2.4993) |
| PancreasMRI | `a` (1.6834) | `ductal` (2.9328) | `of` (1.7219) | `tissue` (2.6102) |

Table A11: The nearest words for each of the 4 context vectors learned by vMFCoOp from GPT-4, with their distances to the corresponding context tokens shown in parentheses.

| Dataset | Context Token #1 | Context Token #2 | Context Token #3 | Context Token #4 |
|---|---|---|---|---|
| BTMRI | `a` (1.214) | `neoplastic` (1.532) | `edema` (0.927) | `enhancement` (1.083) |
| BUSI | `echogenicity` (1.807) | `a` (2.714) | `of` (1.492) | `angioinvasion` (2.586) |
| COVID-QU-Ex | `consolidation` (1.428) | `GGO` (1.583) | `pleural` (1.226) | `a` (1.327) |
| CTKIDNEY | `nephrolithiasis` (1.482) | `a` (1.894) | `hydronephrosis` (1.702) | `of` (1.208) |
| DermaMNIST | `a` (1.983) | `melanocytic` (2.428) | `subepidermal` (2.371) | `actinic` (2.127) |
| Kvasir | `endoluminal` (1.528) | `mucosal` (1.894) | `of` (1.682) | `Barrett` (1.892) |
| CHMNIST | `histopathological` (2.184) | `architectural` (2.573) | `a` (1.726) | `necrotic` (2.592) |
| LC25000 | `a` (1.128) | `squamous` (1.807) | `glandular` (1.224) | `of` (1.482) |
| RETINA | `maculopathy` (1.198) | `a` (1.782) | `drusen` (1.283) | `ischemic` (1.634) |
| KneeXray | `a` (3.028) | `chondrocalcinosis` (4.128) | `subchondral` (2.119) | `of` (2.284) |
| OCTMNIST | `intraretinal` (1.628) | `a` (2.794) | `RPE` (1.426) | `choroidal` (1.892) |
| CardiacMRI | `systolic` (1.208) | `a` (2.214) | `perfusion` (1.382) | `fibrosis` (1.928) |
| LiverMRI | `a` (1.294) | `regenerative` (2.128) | `steatotic` (1.318) | `of` (1.892) |
| PancreasMRI | `ductal` (1.278) | `neuroendocrine` (2.218) | `a` (1.306) | `adenocarcinoma` (1.982) |

Table A12: The nearest words for each of the 4 context vectors learned by vMFCoOp from Qwen-2.5, with their distances to the corresponding context tokens shown in parentheses.
