# Supplementary material for: vMFCoOp: Towards Equilibrium on a Unified Hyperspherical Manifold for Prompting Biomedical VLMs
Source: arXiv:2511.09540 ancillary file (2025-11-20)
Supplement: Supplementary file 2 [file Proofs_document.pdf]

# Theoretical Proofs for vMFCoOp: Towards Equilibrium on a Unified Hyperspherical Manifold for Prompting Biomedical VLMs

Minye Shao

## 1 von Mises–Fisher Distributions and Inverse Parameter Estimation

In this section, we recall the von Mises–Fisher (vMF) distribution on the unit hypersphere, derive its basic moment properties, and provide a principled maximum likelihood (ML) based inverse estimation procedure for its parameters. We then argue why vMF distributions are well aligned with the geometric structure of vision–language model (VLM) embeddings such as CLIP, and how the inverse estimation naturally yields semantic anchors on the hypersphere.

### 1.1 Preliminaries

**Definition 1. *Unit Hypersphere***

Let  $d \geq 2$ . The  $(d - 1)$ -dimensional unit hypersphere in  $\mathbb{R}^d$  is defined as:

$$\mathbb{S}^{d-1} := \{x \in \mathbb{R}^d : \|x\|_2 = 1\}.$$

Its surface area is given by:

$$|\mathbb{S}^{d-1}| = \frac{2\pi^{d/2}}{\Gamma(d/2)},$$

where  $\Gamma(\cdot)$  denotes the gamma function<sup>1</sup>, defined for  $x > 0$  as:

$$\Gamma(x) = \int_0^\infty t^{x-1} e^{-t} dt.$$

**Definition 2. *Modified Bessel function of the first kind***

For order  $\nu > -\frac{1}{2}$ , the modified Bessel function of the first kind  $I_\nu(\kappa) : \mathbb{R} \rightarrow \mathbb{R}$  is defined by the convergent series:

$$I_\nu(\kappa) = \sum_{m=0}^{\infty} \frac{1}{m! \Gamma(m + \nu + 1)} \left(\frac{\kappa}{2}\right)^{2m+\nu}, \quad \kappa \in \mathbb{R}.$$

---

<sup>1</sup>The Gamma function satisfies  $\Gamma(n) = (n - 1)!$  for integers  $n$ .

It admits the following integral representation:

$$I_\nu(\kappa) = \frac{(\kappa/2)^\nu}{\sqrt{\pi} \Gamma(\nu + 1/2)} \int_0^\pi e^{\kappa \cos \theta} (\sin \theta)^{2\nu} d\theta.$$

## 1.2 The von Mises–Fisher Distribution

**Definition 3. vMF Distribution** Let  $\mu \in \mathbb{S}^{d-1}$  be a unit vector (the mean direction) and  $\kappa \geq 0$  be a scalar (the concentration parameter). A random vector  $X$  on  $\mathbb{S}^{d-1}$  is said to follow a von Mises–Fisher (vMF) distribution with parameters  $(\mu, \kappa)$ , denoted  $X \sim \text{vMF}(\mu, \kappa)$ , if its density with respect to the surface measure on  $\mathbb{S}^{d-1}$  is:

$$f(x; \mu, \kappa) = C_d(\kappa) \exp(\kappa \mu^\top x), \quad x \in \mathbb{S}^{d-1},$$

where  $C_d(\kappa)$  is the normalizing constant ensuring  $\int_{\mathbb{S}^{d-1}} f(x; \mu, \kappa) d\sigma(x) = 1$ .

The vMF distribution is rotationally symmetric around  $\mu$ , and its mass becomes more concentrated around  $\mu$  as  $\kappa$  increases.

**Lemma 1. Closed-form expression of the Normalization Constant**

Let  $\nu := \frac{d}{2} - 1$ . The normalizing constant of the vMF distribution satisfies:

$$C_d(\kappa) = \frac{\kappa^\nu}{(2\pi)^{d/2} I_\nu(\kappa)}.$$

*Proof.* We compute:

$$Z_d(\kappa) := \int_{\mathbb{S}^{d-1}} e^{\kappa \mu^\top x} d\sigma(x), \quad C_d(\kappa) = \frac{1}{Z_d(\kappa)}.$$

By rotational symmetry we may, without loss of generality, set  $\mu = e_1 = (1, 0, \dots, 0)^\top$ , so that  $\mu^\top x = x_1$ . We parameterize  $x$  in hyperspherical coordinates as:

$$d\sigma(x) = (\sin \theta)^{d-2} d\theta d\omega,$$

where  $\theta \in [0, \pi]$  is the angle between  $x$  and  $e_1$ , and  $d\omega$  is the surface element on  $\mathbb{S}^{d-2}$ . Hence:

$$Z_d(\kappa) = \int_{\mathbb{S}^{d-1}} e^{\kappa x_1} d\sigma(x) = |\mathbb{S}^{d-2}| \int_0^\pi e^{\kappa \cos \theta} (\sin \theta)^{d-2} d\theta.$$

Let  $\nu = \frac{d}{2} - 1$ , so that  $d - 2 = 2\nu$ . By the integral representation of  $I_\nu(\kappa)$  we obtain:

$$\int_0^\pi e^{\kappa \cos \theta} (\sin \theta)^{d-2} d\theta = \frac{\sqrt{\pi} \Gamma(\nu + 1/2)}{(\kappa/2)^\nu} I_\nu(\kappa).$$

The surface area of  $\mathbb{S}^{d-2}$  is:

$$|\mathbb{S}^{d-2}| = \frac{2\pi^{(d-1)/2}}{\Gamma((d-1)/2)}.$$

Since  $\nu + \frac{1}{2} = \frac{d-1}{2}$ , we have:

$$|\mathbb{S}^{d-2}| \cdot \sqrt{\pi} \Gamma(\nu + 1/2) = \frac{2\pi^{(d-1)/2}}{\Gamma((d-1)/2)} \cdot \sqrt{\pi} \Gamma((d-1)/2) = 2\pi^{d/2}.$$

Combining the above,

$$Z_d(\kappa) = \frac{2\pi^{d/2}}{(\kappa/2)^\nu} I_\nu(\kappa) = 2\pi^{d/2} \cdot 2^\nu \kappa^{-\nu} I_\nu(\kappa) = 2^{\nu+1} \pi^{d/2} \kappa^{-\nu} I_\nu(\kappa).$$

Noting that  $\nu + 1 = d/2$  implies  $2^{\nu+1} \pi^{d/2} = (2\pi)^{d/2}$ , we obtain:

$$Z_d(\kappa) = (2\pi)^{d/2} \kappa^{-\nu} I_\nu(\kappa),$$

and hence:

$$C_d(\kappa) = \frac{1}{Z_d(\kappa)} = \frac{\kappa^\nu}{(2\pi)^{d/2} I_\nu(\kappa)}.$$

□

### 1.3 First Moment and Mean Direction

Define:

$$A_d(\kappa) := \frac{I_{d/2}(\kappa)}{I_{d/2-1}(\kappa)}.$$

**Proposition 1. Mean of a vMF random vector**

Let  $X \sim \text{vMF}(\mu, \kappa)$  on  $\mathbb{S}^{d-1}$ . Then:

$$\mathbb{E}[X] = A_d(\kappa) \mu,$$

so that  $\mu$  is the mean direction and  $\|\mathbb{E}[X]\|_2 = A_d(\kappa)$ .

*Proof.* By rotational symmetry of the vMF density around  $\mu$ , the vector  $\mathbb{E}[X]$  must be colinear with  $\mu$ , i.e., there exists a scalar  $\alpha(\kappa)$  such that:

$$\mathbb{E}[X] = \alpha(\kappa) \mu.$$

Let:

$$Z_d(\kappa) = \int_{\mathbb{S}^{d-1}} e^{\kappa \mu^\top x} d\sigma(x),$$

so that  $f(x; \mu, \kappa) = Z_d(\kappa)^{-1} e^{\kappa \mu^\top x}$ . Then:

$$\begin{aligned} \frac{\partial}{\partial \kappa} \log Z_d(\kappa) &= \frac{1}{Z_d(\kappa)} \int_{\mathbb{S}^{d-1}} (\mu^\top x) e^{\kappa \mu^\top x} d\sigma(x) \\ &= \int_{\mathbb{S}^{d-1}} (\mu^\top x) f(x; \mu, \kappa) d\sigma(x) \\ &= \mathbb{E}[\mu^\top X]. \end{aligned}$$

Since  $Z_d(\kappa) = 1/C_d(\kappa)$ , we have:

$$\log Z_d(\kappa) = -\log C_d(\kappa),$$

and hence:

$$\mathbb{E}[\mu^\top X] = \frac{\partial}{\partial \kappa} \log Z_d(\kappa) = -\frac{\partial}{\partial \kappa} \log C_d(\kappa).$$

From Lemma 1,

$$\log C_d(\kappa) = \left(\frac{d}{2} - 1\right) \log \kappa - \frac{d}{2} \log(2\pi) - \log I_{d/2-1}(\kappa).$$

Differentiating with respect to  $\kappa$  yields:

$$\frac{d}{d\kappa} \log C_d(\kappa) = \frac{d/2 - 1}{\kappa} - \frac{I'_{d/2-1}(\kappa)}{I_{d/2-1}(\kappa)}.$$

derivative of  $I_\nu$  satisfies:

$$I'_\nu(\kappa) = I_{\nu+1}(\kappa) + \frac{\nu}{\kappa} I_\nu(\kappa).$$

Taking  $\nu = d/2 - 1$  gives

$$I'_{d/2-1}(\kappa) = I_{d/2}(\kappa) + \frac{d/2 - 1}{\kappa} I_{d/2-1}(\kappa).$$

Substituting back, we obtain:

$$\frac{d}{d\kappa} \log C_d(\kappa) = -\frac{I_{d/2}(\kappa)}{I_{d/2-1}(\kappa)} = -A_d(\kappa).$$

Therefore:

$$\mathbb{E}[\mu^\top X] = -\frac{d}{d\kappa} \log C_d(\kappa) = A_d(\kappa).$$

On the other hand, using  $\mathbb{E}[X] = \alpha(\kappa)\mu$ , we have:

$$\mu^\top \mathbb{E}[X] = \alpha(\kappa) \mu^\top \mu = \alpha(\kappa),$$

so that  $\alpha(\kappa) = A_d(\kappa)$  and thus:

$$\mathbb{E}[X] = A_d(\kappa) \mu.$$

□

**Remark 1.** Proposition 1 shows that there is a one-to-one correspondence between the vMF parameters  $(\mu, \kappa)$  and the first moment:

$$(\mu, \kappa) \longleftrightarrow \left( \frac{\mathbb{E}[X]}{\|\mathbb{E}[X]\|_2}, \|\mathbb{E}[X]\|_2 \right),$$

where the direction of the mean vector determines  $\mu$  and its length determines  $\kappa$  through  $A_d(\kappa)$ . This is the basis of the inverse parameter estimation discussed below.

## 1.4 Maximum Likelihood and Inverse Estimation

Let  $x_1, \dots, x_n \in \mathbb{S}^{d-1}$  be i.i.d. samples from  $\text{vMF}(\mu, \kappa)$ . Define:

$$R := \sum_{i=1}^n x_i, \quad \bar{x} := \frac{1}{n}R, \quad \bar{R} := \|\bar{x}\|_2 = \frac{\|R\|_2}{n}.$$

### Log-likelihood

The likelihood of  $(\mu, \kappa)$  given  $\{x_i\}_{i=1}^n$  is:

$$L(\mu, \kappa) = \prod_{i=1}^n f(x_i; \mu, \kappa) = C_d(\kappa)^n \exp\left(\kappa \mu^\top \sum_{i=1}^n x_i\right).$$

The log-likelihood is:

$$\ell(\mu, \kappa) = \log L(\mu, \kappa) = n \log C_d(\kappa) + \kappa \mu^\top R, \quad \text{subject to } \|\mu\|_2 = 1.$$

### Proposition 2. MLE of the mean direction on the hypersphere

For fixed  $\kappa \geq 0$ , the maximizer of  $\ell(\mu, \kappa)$  under the constraint  $\|\mu\|_2 = 1$  is:

$$\hat{\mu} = \frac{R}{\|R\|_2} = \frac{\bar{x}}{\|\bar{x}\|_2}.$$

*Proof.* For fixed  $\kappa \geq 0$ , the log-likelihood

$$\ell(\mu, \kappa) = n \log C_d(\kappa) + \kappa \mu^\top R$$

differs from  $\kappa \mu^\top R$  only by an additive constant with respect to  $\mu$ . Indeed, the term  $n \log C_d(\kappa)$  does not depend on  $\mu$ , and therefore

$$\ell(\mu, \kappa) = \kappa \mu^\top R + \text{constant}.$$

Thus we maximize

$$\mu \mapsto \kappa \mu^\top R \quad \text{subject to } \|\mu\|_2 = 1.$$

This is a linear functional on the unit sphere, which attains its maximum when  $\mu$  is aligned with  $R$ . Formally, consider the Lagrangian:

$$\mathcal{L}(\mu, \lambda) = \kappa \mu^\top R + \lambda(\mu^\top \mu - 1).$$

Taking derivatives with respect to  $\mu$  and setting them to zero gives:

$$\nabla_\mu \mathcal{L} = \kappa R + 2\lambda \mu = 0 \quad \Rightarrow \quad \mu \parallel R.$$

Imposing the unit-norm constraint  $\|\mu\|_2 = 1$  yields:

$$\mu = \pm \frac{R}{\|R\|_2}.$$

Since  $\kappa \geq 0$  and the log-likelihood is proportional to  $\kappa \mu^\top R$ , the maximum is achieved when  $\mu$  is in the same direction as  $R$ , i.e.,

$$\hat{\mu} = \frac{R}{\|R\|_2}.$$

□

**Proposition 3. MLE equation for the Concentration on the Hypersphere**

*Substituting  $\hat{\mu} = R/\|R\|_2$  into the log-likelihood and maximizing with respect to  $\kappa$  leads to the first-order condition*

$$A_d(\hat{\kappa}) = \bar{R}, \quad A_d(\kappa) = \frac{I_{d/2}(\kappa)}{I_{d/2-1}(\kappa)}.$$

*Proof.* Using Proposition 2, we obtain:

$$\ell(\hat{\mu}, \kappa) = n \log C_d(\kappa) + \kappa \hat{\mu}^\top R = n \log C_d(\kappa) + \kappa \|R\|_2.$$

Differentiating with respect to  $\kappa$  gives:

$$\frac{\partial}{\partial \kappa} \ell(\hat{\mu}, \kappa) = n \frac{d}{d\kappa} \log C_d(\kappa) + \|R\|_2.$$

From Proposition 1 we know

$$\frac{d}{d\kappa} \log C_d(\kappa) = -A_d(\kappa),$$

hence:

$$\frac{\partial}{\partial \kappa} \ell(\hat{\mu}, \kappa) = n(-A_d(\kappa)) + \|R\|_2 = n(-A_d(\kappa) + \bar{R}).$$

Setting the derivative to zero yields the MLE equation:

$$-A_d(\hat{\kappa}) + \bar{R} = 0 \quad \Leftrightarrow \quad A_d(\hat{\kappa}) = \bar{R}.$$

□

**Remark 2. Inverse estimation of  $(\mu, \kappa)$**

*Propositions 2 and 3 show that the ML estimation of the vMF parameters  $(\mu, \kappa)$  from samples  $\{x_i\}$  proceeds by:*

1. *Computing the sample mean direction:*

$$\hat{\mu} = \frac{\bar{x}}{\|\bar{x}\|_2}, \quad \bar{x} = \frac{1}{n} \sum_{i=1}^n x_i;$$

2. Computing the sample resultant length:

$$\bar{R} = \|\bar{x}\|_2;$$

3. Solving the scalar equation:

$$A_d(\hat{\kappa}) = \bar{R}$$

for  $\hat{\kappa}$  (numerically or using standard approximations).

Thus, the inverse estimation ( $\bar{x} \mapsto (\hat{\mu}, \hat{\kappa})$ ) is determined purely by the first-order statistics of the samples: the direction of the sample mean and its norm.

## 1.5 Connection to VLM Embeddings

We now explain why the vMF model is well aligned with the representation geometry of vision–language models such as CLIP, and why the inverse estimation procedure above provides a principled way to recover *semantic anchors* from their embeddings.

### Fact 1. Spherical geometry of CLIP embeddings

In CLIP and related VLMs, both image and text encoders produce feature vectors  $z \in \mathbb{R}^d$ , which are typically  $L^2$ -normalized before computing similarities:

$$x = \frac{z}{\|z\|_2} \in \mathbb{S}^{d-1}.$$

The similarity between two embeddings  $x_i, x_j$  is given by their inner product (or cosine similarity)

$$\text{sim}(x_i, x_j) = x_i^\top x_j = \cos \angle(x_i, x_j),$$

so that the representation space is naturally the unit hypersphere  $\mathbb{S}^{d-1}$ .

**Assumption 1** (Class-conditional vMF model for CLIP text embeddings). Consider a semantic class  $c$  and a collection of textual prompts  $\{p_{c,j}\}_{j=1}^{n_p}$  associated with it. Let

$$t_{c,j} \in \mathbb{S}^{d-1}, \quad j = 1, \dots, n_p,$$

denote the corresponding  $L^2$ -normalized CLIP text embeddings. We assume that, for each class  $c$ , the embeddings  $\{t_{c,j}\}$  are approximately unimodal and isotropically concentrated around some mean direction  $\mu_c \in \mathbb{S}^{d-1}$ , and can be modelled as

$$t_{c,j} \sim \text{vMF}(\mu_c, \kappa_c), \quad j = 1, \dots, n_p,$$

for some concentration parameter  $\kappa_c \geq 0$ .

Under this assumption,  $(\mu_c, \kappa_c)$  can be interpreted as a *semantic anchor* (direction) and a *semantic confidence* (concentration) for class  $c$  on the hypersphere.

**Proposition 4. Consistency of inverse vMF estimation for semantic anchors**

Under Assumption 1, define

$$\bar{t}_c = \frac{1}{n_p} \sum_{j=1}^{n_p} t_{c,j}, \quad R_{L,c} = \|\bar{t}_c\|_2.$$

Let  $(\hat{\mu}_c, \hat{\kappa}_c)$  be the maximum likelihood estimates obtained from  $\{t_{c,j}\}$  via

$$\hat{\mu}_c = \frac{\bar{t}_c}{\|\bar{t}_c\|_2}, \quad A_d(\hat{\kappa}_c) = R_{L,c}.$$

Then, as  $n_p \rightarrow \infty$ ,

$$\hat{\mu}_c \rightarrow \mu_c, \quad \hat{\kappa}_c \rightarrow \kappa_c$$

in probability; that is,  $(\hat{\mu}_c, \hat{\kappa}_c)$  consistently recover the underlying class-conditional semantic anchor and concentration.

*Proof sketch.* By Assumption 1 and Proposition 1, we have

$$\mathbb{E}[t_{c,j}] = A_d(\kappa_c) \mu_c.$$

By the law of large numbers,  $\bar{t}_c \rightarrow \mathbb{E}[t_{c,j}]$  in probability as  $n_p \rightarrow \infty$ . Therefore:

$$\frac{\bar{t}_c}{\|\bar{t}_c\|_2} \rightarrow \mu_c, \quad \|\bar{t}_c\|_2 \rightarrow A_d(\kappa_c).$$

Using the strict monotonicity of  $A_d(\kappa)$  in  $\kappa \geq 0$ , the equation  $A_d(\hat{\kappa}_c) = R_{L,c}$  implies  $\hat{\kappa}_c \rightarrow \kappa_c$ . Hence  $(\hat{\mu}_c, \hat{\kappa}_c)$  are consistent estimators of  $(\mu_c, \kappa_c)$ .  $\square$

**Remark 3. Rationale for inverse vMF estimation in VLMs**

Combining Fact 1, Assumption 1, and Propositions 2, 3, and 4, we obtain the following conceptual picture:

- CLIP/VLM embeddings live on the unit hypersphere, and cosine similarity corresponds to geodesic similarity on  $\mathbb{S}^{d-1}$ .
- For each semantic class  $c$ , its text embeddings form a concentrated, approximately unimodal cluster on  $\mathbb{S}^{d-1}$ , naturally modeled by a vMF distribution.
- The vMF parameters  $(\mu_c, \kappa_c)$  can be inversely estimated from the first-order statistics of the CLIP embeddings via maximum likelihood.
- The estimated  $\hat{\mu}_c$  serves as a semantic anchor on the sphere, while  $\hat{\kappa}_c$  quantifies the intrinsic semantic concentration/uncertainty of the class in the CLIP representation space.

In summary, this provides a mathematically rigorous justification for treating vMF-based inverse estimation as a principled mechanism to extract and model semantic anchor fields from VLM embeddings.



## 2 Unified Semantic Anchors and Hyperspherical Manifold Constraints

In this section we build on the vMF modeling and inverse estimation results established in Section 1 to justify the three key constraints used in vMFCoOp. We show that (1) the proposed unified semantic anchors arise from a principled fusion of vMF factors, (2) the Semantic Anchor Loss is geometrically equivalent to an angular alignment objective on the unit hypersphere, and (3) the Spherical Contrastive Loss implements a supervised angular margin on the same hyperspherical manifold. Throughout this section we retain the notation of Section 1 and assume all feature vectors have been  $\ell_2$ -normalized to lie on the unit hypersphere  $\mathbb{S}^{d-1} = \{x \in \mathbb{R}^d : \|x\|_2 = 1\}$ .

### 2.1 Product of vMF Factors and Unified Semantic Anchors

Recall that Section 1 modeled CLIP text embeddings and LLM-generated prompt embeddings as vMF-distributed directional data on  $\mathbb{S}^{d-1}$ , and used maximum likelihood estimation (MLE) to obtain consistent estimators of the corresponding mean directions and concentrations. Concretely, we consider:

- A *CLIP semantic anchor field* modeled as  $w \sim \text{vMF}(\mu_C, \kappa_C)$ , where  $\mu_C \in \mathbb{S}^{d-1}$  is the global semantic direction of the CLIP vocabulary and  $\kappa_C \geq 0$  encodes its concentration.
- For each class  $c$ , an *LLM semantic prototype field* modeled as  $t_{c,j} \sim \text{vMF}(\mu_{L,c}, \kappa_{L,c})$ , where  $\mu_{L,c} \in \mathbb{S}^{d-1}$  is the class-conditional semantic prototype direction and  $\kappa_{L,c} \geq 0$  its concentration.

The following proposition formalizes the “product closure” of vMF factors and provides the analytical basis for fusing these two semantic fields.

**Proposition 5. *Product/fusion of vMF factors***

Let  $x \in \mathbb{S}^{d-1}$  and consider two vMF-shaped factors:

$$p_C(x) \propto \exp(\kappa_C \mu_C^\top x), \quad p_{L,c}(x) \propto \exp(\kappa_{L,c} \mu_{L,c}^\top x),$$

where  $\mu_C, \mu_{L,c} \in \mathbb{S}^{d-1}$  and  $\kappa_C, \kappa_{L,c} \geq 0$ . Then their product is again of vMF form:

$$p_C(x) p_{L,c}(x) \propto \exp((\kappa_C \mu_C + \kappa_{L,c} \mu_{L,c})^\top x) = \exp(\kappa_c^* \mu_c^{*\top} x),$$

where

$$m_c := \kappa_C \mu_C + \kappa_{L,c} \mu_{L,c}, \quad \kappa_c^* := \|m_c\|_2, \quad \mu_c^* := \frac{m_c}{\|m_c\|_2}.$$

In particular, if  $m_c \neq 0$  then  $\mu_c^* \in \mathbb{S}^{d-1}$  and  $\kappa_c^* \geq 0$ , and the product distribution belongs to the  $\text{vMF}(\mu_c^*, \kappa_c^*)$  family up to a normalizing constant.

*Proof.* By direct expansion,

$$p_C(x) p_{L,c}(x) \propto \exp(\kappa_C \mu_C^\top x) \exp(\kappa_{L,c} \mu_{L,c}^\top x) = \exp((\kappa_C \mu_C + \kappa_{L,c} \mu_{L,c})^\top x).$$

Define  $m_c = \kappa_C \mu_C + \kappa_{L,c} \mu_{L,c}$ . If  $m_c = 0$ , the product is constant in  $x$  and corresponds to the uniform distribution on  $\mathbb{S}^{d-1}$ , i.e.,  $\kappa_c^* = 0$ . Otherwise, set

$$\kappa_c^* = \|m_c\|_2, \quad \mu_c^* = \frac{m_c}{\|m_c\|_2}.$$

Then  $\mu_c^* \in \mathbb{S}^{d-1}$  and

$$(\kappa_C \mu_C + \kappa_{L,c} \mu_{L,c})^\top x = m_c^\top x = \kappa_c^* \mu_c^{*\top} x,$$

so that:

$$p_C(x) p_{L,c}(x) \propto \exp(\kappa_c^* \mu_c^{*\top} x),$$

which is exactly the unnormalized density of a vMF distribution with parameters  $(\mu_c^*, \kappa_c^*)$ . This proves the claim.  $\square$

The unified semantic anchors used in vMFCoOp arise as a direct corollary of Proposition 5.

**Corollary 1. *Unified semantic anchors***

*Define the CLIP and LLM contribution vectors:*

$$a_C := \kappa_C \mu_C, \quad a_{L,c} := \kappa_{L,c} \mu_{L,c},$$

*and the unified semantic anchor for class  $c$  as:*

$$u_c := \frac{a_C + a_{L,c}}{\|a_C + a_{L,c}\|_2} = \frac{\kappa_C \mu_C + \kappa_{L,c} \mu_{L,c}}{\|\kappa_C \mu_C + \kappa_{L,c} \mu_{L,c}\|_2}.$$

*Then  $u_c$  coincides with the mean direction  $\mu_c^*$  in Proposition 5, i.e.*

$$u_c = \mu_c^*.$$

*Proof.* Comparing with Proposition 5, we have  $m_c = \kappa_C \mu_C + \kappa_{L,c} \mu_{L,c}$  and  $\mu_c^* = m_c / \|m_c\|_2$ . Since  $a_C + a_{L,c} = m_c$ , we obtain:

$$u_c = \frac{a_C + a_{L,c}}{\|a_C + a_{L,c}\|_2} = \frac{m_c}{\|m_c\|_2} = \mu_c^*.$$

$\square$

**Remark 4.** *Corollary 1 shows that the fusion rule:*

$$u_c = \frac{\kappa_C \mu_C + \kappa_{L,c} \mu_{L,c}}{\|\kappa_C \mu_C + \kappa_{L,c} \mu_{L,c}\|_2},$$

*which vMFCoOp uses to define unified semantic anchors, is not an ad-hoc heuristic but the exact mean-direction parameter of the product of two vMF factors: a global CLIP semantic prior and a class-conditional LLM semantic prototype. The unified anchor  $u_c$  can thus be interpreted as a posterior semantic direction that reconciles these two priors on the shared hyperspherical manifold.*

## 2.2 Angular Geometry on the Unit Hypersphere

The losses used in vMFCoOp are defined in terms of  $\ell_2$  distances and cosine similarities between normalized vectors. The following basic geometric identity formalizes the equivalence of these metrics on  $\mathbb{S}^{d-1}$ .

**Proposition 6.** *Angular–Euclidean equivalence on  $\mathbb{S}^{d-1}$*

Let  $\tilde{p}, \tilde{u} \in \mathbb{S}^{d-1}$  be unit vectors and denote their angle by:

$$\theta = \arccos(\tilde{p}^\top \tilde{u}) \in [0, \pi].$$

Then

$$\|\tilde{p} - \tilde{u}\|_2^2 = 2(1 - \cos \theta) = 2(1 - \tilde{p}^\top \tilde{u}).$$

*Proof.* Expanding the squared Euclidean distance,

$$\|\tilde{p} - \tilde{u}\|_2^2 = (\tilde{p} - \tilde{u})^\top (\tilde{p} - \tilde{u}) = \|\tilde{p}\|_2^2 + \|\tilde{u}\|_2^2 - 2\tilde{p}^\top \tilde{u}.$$

Since  $\|\tilde{p}\|_2 = \|\tilde{u}\|_2 = 1$ , this simplifies to:

$$\|\tilde{p} - \tilde{u}\|_2^2 = 2(1 - \tilde{p}^\top \tilde{u}).$$

Using  $\tilde{p}^\top \tilde{u} = \cos \theta$  yields:

$$\|\tilde{p} - \tilde{u}\|_2^2 = 2(1 - \cos \theta),$$

as claimed.  $\square$

**Remark 5.** *Proposition 6 implies that, on the unit hypersphere, minimizing the squared  $\ell_2$  distance between two vectors is exactly equivalent (up to a constant factor and offset) to maximizing their cosine similarity or, equivalently, minimizing the angle between them. This observation underlies the geometric interpretation of the Semantic Anchor Loss and the Spherical Contrastive Loss in vMFCoOp.*

## 2.3 Geometric Interpretation of vMFCoOp Losses

We now formalize the geometric role of the Semantic Anchor Loss and the Spherical Contrastive Loss on the shared hyperspherical manifold.

### Semantic Anchor Loss as directional alignment

For each class  $c$ , let  $P_c \in \mathbb{R}^d$  denote the (unnormalized) prompt embedding produced by the prompt learner, and define its normalized version:

$$\tilde{P}_c := \frac{P_c}{\|P_c\|_2} \in \mathbb{S}^{d-1}.$$

Let  $u_c \in \mathbb{S}^{d-1}$  be the unified semantic anchor from Corollary 1. vMFCoOp introduces a dynamic target direction via a learnable offset  $\delta_c \in \mathbb{R}^d$  and a global scale  $\alpha > 0$ :

$$u_c^d := u_c + \alpha \delta_c, \quad \tilde{u}_c^d := \frac{u_c^d}{\|u_c^d\|_2} \in \mathbb{S}^{d-1}.$$

The Semantic Anchor Loss is then defined as:

$$L_{\text{anc}} = \frac{1}{C} \sum_{c=1}^C \|\tilde{P}_c - \tilde{u}_c^d\|_2^2.$$

**Proposition 7** (Semantic Anchor Loss as angular alignment). *For each class  $c$ , let  $\theta_c = \arccos(\tilde{P}_c^\top \tilde{u}_c^d)$  be the angle between the normalized prompt embedding and its dynamic anchor. Then*

$$L_{\text{anc}} = \frac{2}{C} \sum_{c=1}^C (1 - \cos \theta_c),$$

and in particular, minimizing  $L_{\text{anc}}$  is equivalent to minimizing the angular deviations  $\{\theta_c\}_{c=1}^C$  between prompts and their (unified) semantic anchors.

*Proof.* Applying Proposition 6 to the pair  $(\tilde{P}_c, \tilde{u}_c^d)$  yields:

$$\|\tilde{P}_c - \tilde{u}_c^d\|_2^2 = 2(1 - \tilde{P}_c^\top \tilde{u}_c^d) = 2(1 - \cos \theta_c).$$

Substituting into the definition of  $L_{\text{anc}}$  gives:

$$L_{\text{anc}} = \frac{1}{C} \sum_{c=1}^C \|\tilde{P}_c - \tilde{u}_c^d\|_2^2 = \frac{2}{C} \sum_{c=1}^C (1 - \cos \theta_c),$$

which shows that minimizing  $L_{\text{anc}}$  is equivalent to maximizing the average cosine similarity  $\tilde{P}_c^\top \tilde{u}_c^d$  and hence to minimizing the angular deviations  $\theta_c$ .  $\square$

**Remark 6.** *Combining Corollary 1 and Proposition 7, we obtain the following chain:*

$$\begin{aligned} \text{CLIP semantic prior} + \text{LLM semantic prototype} &\xrightarrow{\text{vMF product}} \text{unified anchor} \\ u_c &\xrightarrow{\text{Semantic Anchor Loss}} \text{angular alignment of prompts to } u_c \text{ on } \mathbb{S}^{d-1}. \end{aligned}$$

*In other words, the Semantic Anchor Loss drives prompt embeddings toward the posterior semantic directions implied by the joint vMF model of CLIP and LLM semantics, in a way that is geometrically consistent with the hyperspherical structure of the embedding space.*

### Spherical Contrastive Loss as supervised angular separation

Let  $\tilde{P} \in \mathbb{R}^{C \times d}$  be the matrix whose  $c$ -th row is  $\tilde{P}_c$ , and let  $U \in \mathbb{R}^{C \times d}$  be the matrix whose  $j$ -th row is the unified semantic anchor  $u_j$ . Both matrices have row-wise unit norm. vMFCoOp defines the prototype affinity matrix:

$$S = \tau \tilde{P} U^\top \in \mathbb{R}^{C \times C}, \quad S_{cj} = \tau \tilde{P}_c^\top u_j = \tau \cos \theta_{cj},$$

where  $\theta_{cj} = \arccos(\tilde{P}_c^\top u_j)$  is the angle between the prompt for class  $c$  and the unified anchor of class  $j$ , and  $\tau > 0$  is a temperature parameter (possibly annealed during training).

The Spherical Contrastive Loss is the row-wise softmax cross-entropy:

$$L_{sc} = -\frac{1}{C} \sum_{c=1}^C \log \frac{\exp(S_{cc})}{\sum_{j=1}^C \exp(S_{cj})}.$$

**Proposition 8** (Spherical Contrastive Loss as angular margin). *For each class  $c$ , the contribution of row  $c$  to  $L_{sc}$  is*

$$-\log \frac{\exp(\tau \cos \theta_{cc})}{\sum_{j=1}^C \exp(\tau \cos \theta_{cj})}.$$

*Minimizing  $L_{sc}$  encourages  $\theta_{cc}$  to be small and  $\theta_{cj}$  to be large for all  $j \neq c$ , thereby enforcing supervised angular separation between prompts and non-matching anchors on  $\mathbb{S}^{d-1}$ .*

*Proof sketch.* For fixed  $c$ , write

$$\ell_c := -\log \frac{\exp(\tau \cos \theta_{cc})}{\sum_{j=1}^C \exp(\tau \cos \theta_{cj})}.$$

The partial derivatives of  $\ell_c$  with respect to the logits  $\{\cos \theta_{cj}\}_j$  have the standard softmax-cross-entropy form:

$$\frac{\partial \ell_c}{\partial (\tau \cos \theta_{cc})} = p_{cc} - 1, \quad \frac{\partial \ell_c}{\partial (\tau \cos \theta_{cj})} = p_{cj}, \quad j \neq c,$$

where  $p_{cj} = \exp(S_{cj}) / \sum_k \exp(S_{ck})$  is the softmax probability on row  $c$ . Thus, gradient descent on  $\ell_c$  increases  $\cos \theta_{cc}$  (since  $p_{cc} < 1$ ) and decreases  $\cos \theta_{cj}$  for  $j \neq c$  (since  $p_{cj} > 0$ ). In terms of angles, this corresponds to decreasing  $\theta_{cc}$  and increasing  $\theta_{cj}$ , establishing supervised angular separation between the prompt for class  $c$  and the anchors of all other classes.  $\square$

**Remark 7.** *Propositions 7 and 8 together show that vMFCoOp optimizes prompt embeddings on the unit hypersphere under two complementary geometric criteria:*

- Anchor-centric alignment: *prompts are pulled toward their unified semantic anchors  $u_c$ , which themselves are posterior vMF directions fusing CLIP and LLM semantics;*

- Inter-class separation: *prompts are simultaneously pushed away from non-matching anchors via a supervised angular margin encoded in  $L_{\text{sc}}$ .*

*These constraints act entirely within the hyperspherical manifold, consistent with the directional nature of CLIP and vMF representations.*

### **Symmetric Cross-Entropy as distributional alignment**

Finally, note that image features and prompt features are both normalized to  $\mathbb{S}^{d-1}$  and compared via inner products. The Symmetric Cross-Entropy Loss  $L_{\text{SCE}}$  operates on the resulting class probabilities, encouraging agreement between visual and prompt-based predictions in a distributional sense, while the two geometric losses  $L_{\text{anc}}$  and  $L_{\text{sc}}$  shape the underlying angular geometry on the shared hyperspherical manifold. Together, these constraints drive few-shot samples toward a multimodal semantic equilibrium centered at the unified semantic anchor field.
